# Supplementary material for: Towards detection of molecular parity violation by microwave spectroscopy of CpRe(CH$_{3}$)(CO)(NO)
Source: arXiv:2303.08263 ancillary file (2023-05-08)
Supplement: Supplementary file 1 [file SupportingInformation.pdf]

# Supporting Information for

## **Towards detection of molecular parity violation by microwave spectroscopy of $\text{CpRe}(\text{CH}_3)(\text{CO})(\text{NO})$ .**

*Nityananda Sahu,<sup>1</sup> Konstantin Gaul,<sup>1</sup> Anke Wilm,<sup>1</sup> Melanie Schnell<sup>2</sup> and Robert Berger<sup>1,\*</sup>*

<sup>1</sup>*Fachbereich Chemie, Philipps-Universität Marburg, Hans-Meerwein-Straße 4, 35032 Marburg, Germany*

<sup>2</sup>*Deutsches Elektronen-Synchrotron DESY, Notkestr. 85, 22607 Hamburg, Germany*

## **1 Data on calculations of parity-violating rotational constant shifts and of nuclear electric quadrupole coupling tensors**

In the following all computed molecular structures, the corresponding rotational constants, Re-ligand distances, NEQC tensors for  $^{14}\text{N}$  and  $^{187}\text{Re}$ , PV energy shifts, PV energy gradients and harmonic force fields are given.

Table S1: Nuclear cartesian coordinates of  $\text{Cp}^{187}\text{Re}(\text{CH}_3)(\text{CO})(^{14}\text{NO})$  optimized at Hartree–Fock and density functional theory levels including the PBE, PBE0 and B3LYP exchange correlation functional. Calculations were performed on the one-component level with relativistic effective core potential (RECP), employing the basis sets cc-pV5Z on H, C, N and O and cc-pwCVQZ-PP on Re (cc5Z) or def2-TZVPP (def3Z) on all atoms and on the two-component zeroth order regular approximation (ZORA) level employing the all-electron basis sets x2c-TZVPPall-2c (x2c3Z). All coordinates in Å.

| Coordinate |   | def3Z       | B3LYP<br>cc5Z | x2c3Z      | def3Z      | HF<br>cc5Z | x2c3Z      | PBE0<br>cc5Z | x2c3Z      | def3Z      | PBE<br>cc5Z | x2c3Z      | B3LYP/cc5Z <sup>1</sup> |
|------------|---|-------------|---------------|------------|------------|------------|------------|--------------|------------|------------|-------------|------------|-------------------------|
| C          | x | -0.0051827  | -0.0061782    | 0.0049870  | -0.0233880 | -0.0251046 | -0.0090151 | -0.0010017   | 0.0083057  | -0.0055775 | -0.0063610  | 0.0083695  | 0.0000000               |
|            | y | -0.0071836  | -0.0021222    | 0.0599473  | -0.0311052 | -0.0268350 | -0.010811  | 0.0212458    | 0.0259381  | 0.0153597  | 0.0201423   | 0.0817608  | 0.0000000               |
|            | z | 0.0003314   | 0.0008897     | -0.0037983 | -0.0274071 | -0.0263234 | -0.0762999 | 0.0006750    | 0.0012257  | -0.0054390 | 0.0122433   | 0.0101607  | 0.0000000               |
| H          | x | -0.00913374 | -0.0112992    | 0.0094763  | -0.0510307 | -0.0543097 | -0.0344572 | -0.0041063   | -0.0059252 | 0.0136823  | -0.0094636  | -0.0110923 | 0.0163748               |
|            | y | -0.0079713  | -0.0028413    | 0.0639100  | -0.0538996 | -0.0500353 | -0.0571843 | 0.0336620    | 0.0378170  | 0.1078504  | 0.0310560   | 0.0353781  | 0.1035469               |
|            | z | 1.0775878   | 1.0773391     | 1.0719205  | 1.0407639  | 1.0412429  | 0.9900523  | 1.0791297    | 1.0792063  | 1.0715679  | 1.0977421   | 1.0978500  | 1.0945055               |
| C          | x | 1.1425216   | 1.1417559     | 1.1458863  | 1.1301429  | 1.1289498  | 1.1418843  | 1.1443693    | 1.1435988  | 1.1469902  | 1.1489908   | 1.1482926  | 1.1538808               |
|            | y | -0.0043995  | 0.0003963     | 0.0896088  | -0.0207679 | -0.0165796 | 0.0517871  | 0.0239257    | 0.0282354  | 0.1224074  | 0.0135674   | 0.0180391  | 0.1079699               |
|            | z | -0.8290140  | -0.8268099    | -0.8375465 | -0.8235947 | -0.8204029 | -0.8694782 | -0.8278463   | -0.8260154 | -0.8388150 | -0.8215829  | -0.8198511 | -0.8313797              |
| H          | x | 2.1630873   | 2.1611951     | 2.1638723  | 2.1349108  | 2.1326763  | 2.1426995  | 2.1656993    | 2.1642622  | 2.1658377  | 2.1770473   | 2.1757242  | 2.1804441               |
|            | y | 0.0397678   | 0.0440540     | 0.1654910  | 0.0184365  | 0.0217233  | 0.1917356  | 0.0797362    | 0.0826783  | 0.2148192  | 0.0651333   | 0.0685193  | 0.1936235               |
|            | z | -0.4878494  | -0.4846307    | -0.4993529 | -0.4631447 | -0.4585610 | -0.5063400 | -0.4863063   | -0.4836234 | -0.5022835 | -0.4768031  | -0.4742957 | -0.4935549              |
| C          | x | 0.7260820   | 0.7274108     | 0.7280835  | 0.7470114  | 0.7482183  | 0.7629031  | 0.7301496    | 0.7310563  | 0.7313181  | 0.7326300   | 0.7335243  | 0.7322875               |
|            | y | -0.0301108  | -0.0233162    | 0.0619488  | -0.0180676 | -0.0105971 | 0.0852884  | -0.0118978   | -0.0048999 | 0.0803847  | -0.0267125  | -0.0197736 | 0.0629081               |
|            | z | -2.1828789  | -2.1807037    | -2.1877732 | -2.1796420 | -2.1764696 | -2.2228522 | -2.1792484   | -2.1774299 | -2.1865636 | -2.1824290  | -2.1807468 | -2.1845200              |
| H          | x | 1.3695295   | 1.3715297     | 1.3709226  | 1.4039773  | 1.4061291  | 1.4226427  | 1.3752612    | 1.3768078  | 1.3766552  | 1.3827289   | 1.3842570  | 1.3804163               |
|            | y | -0.0473732  | -0.0398332    | 0.0744494  | -0.0311337 | -0.0223368 | 0.1280176  | -0.0274217   | -0.0196171 | 0.0940244  | -0.0449081  | -0.0373067 | 0.0736369               |
|            | z | -3.0467002  | -3.0430489    | -3.0505659 | -3.0218705 | -3.0172592 | -3.0606710 | -3.0434610   | -3.0405890 | -3.0493006 | -3.0518697  | -3.0491864 | -3.0570889              |
| C          | x | -1.1604004  | -1.1603283    | -1.1545022 | -1.1520190 | -1.1524189 | -1.1370604 | -1.1547952   | -1.1551352 | -1.1493550 | -1.1678755  | -1.1679928 | -1.1605348              |
|            | y | -0.0389311  | -0.0303601    | 0.0131641  | -0.0447957 | -0.0371939 | -0.0281706 | -0.0127108   | -0.0038253 | 0.0320847  | -0.0160689  | -0.0071964 | 0.0315741               |
|            | z | -0.8470569  | -0.8475330    | -0.8452801 | -0.8946017 | -0.8948554 | -0.9445172 | -0.8447946   | -0.8450687 | -0.8453400 | -0.8399011  | -0.8401332 | -0.8325027              |
| H          | x | -2.1854696  | -2.1850477    | -2.1743643 | -2.1753963 | -2.1756878 | -2.1565522 | -2.1813621   | -2.1813678 | -2.1703621 | -2.2012040  | -2.2012134 | -2.1808800              |
|            | y | -0.0910850  | -0.0817009    | -0.0691378 | -0.1091727 | -0.1008926 | -0.1340796 | -0.0630829   | -0.0533778 | -0.0519691 | -0.0628414  | -0.0532335 | -0.0457847              |
|            | z | -0.5219112  | -0.5237742    | -0.5150520 | -0.5962639 | -0.5980242 | -0.6488855 | -0.5191235   | -0.5203535 | -0.5141437 | -0.5121169  | -0.5132529 | -0.4963674              |
| C          | x | -0.7025823  | -0.7008406    | -0.6989817 | -0.6676251 | -0.6661751 | -0.6943891 | -0.6960555   | -0.6948490 | -0.6929089 | -0.7044456  | -0.7032669 | -0.7032574              |
|            | y | -0.0469389  | -0.0374912    | 0.0194155  | -0.0454898 | -0.0360070 | 0.0211785  | -0.0272240   | -0.0171653 | 0.0304697  | -0.0324738  | -0.0225980 | 0.0270838               |
|            | z | -2.1914785  | -2.1910813    | -2.1909724 | -2.2180079 | -2.2170258 | -2.2648258 | -2.1876248   | -2.1872145 | -2.1893505 | -2.1926276  | -2.1922809 | -2.1879841              |
| H          | x | -1.3269113  | -1.3236153    | -1.3234357 | -1.2679735 | -1.2647394 | -1.2451244 | -1.3210701   | -1.3186541 | -1.3174924 | -1.3327269  | -1.3304468 | -1.3341326              |
|            | y | -0.0737327  | -0.0617086    | -0.0053245 | -0.0608650 | -0.0486607 | 0.0301667  | -0.0530034   | -0.0398569 | 0.0002580  | -0.0592206  | -0.0463185 | -0.0010405              |
|            | z | -3.0696998  | -3.0695406    | -3.0674609 | -3.1026578 | -3.1022455 | -3.1514225 | -3.0670710   | -3.0670646 | -3.0674570 | -3.0784686  | -3.0785031 | -3.0704468              |
| Re         | x | -0.0977918  | -0.0962475    | -0.1206462 | -0.1032870 | -0.1021408 | -0.1261964 | -0.0948854   | -0.0928654 | -0.1242012 | -0.0931851  | -0.0912683 | -0.1141295              |
|            | y | 2.0071819   | 2.0033026     | 1.9722200  | 2.0139231  | 2.0103049  | 1.9667451  | 1.9783344    | 1.9747987  | 1.9583328  | 1.9837498   | 1.9800238  | 1.9548595               |
|            | z | -1.2454054  | -1.2444336    | -1.2448966 | -1.2487804 | -1.2471724 | -1.2454718 | -1.2521730   | -1.2506407 | -1.2548738 | -1.2503578  | -1.2489747 | -1.2484498              |
| C          | x | -1.0636799  | -1.0604579    | -1.0731677 | -0.9958119 | -0.9941168 | -1.0204220 | -1.0528420   | -1.0504218 | -1.0684128 | -1.0655647  | -1.0628925 | -1.0685661              |
|            | y | 3.0529608   | 3.0422094     | 3.0535153  | 3.1527625  | 3.1393404  | 3.1187330  | 3.0197146    | 3.0089253  | 3.0365841  | 3.0047276   | 2.9940499  | 3.0178425               |
|            | z | 0.0469531   | 0.0453810     | 0.0271216  | 0.0814571  | 0.0800736  | 0.0793523  | 0.0290985    | 0.0282569  | 0.0037412  | 0.0419666   | 0.0409852  | 0.0239162               |
| N          | x | -0.4212699  | -0.4213641    | -0.4377325 | -0.5261592 | -0.5238127 | -0.5346252 | -0.4213002   | -0.4207873 | -0.4456761 | -0.4115163  | -0.4110018 | -0.4270688              |
|            | y | 3.1827009   | 3.1710398     | 3.1513805  | 3.1252456  | 3.1144190  | 3.0904967  | 3.1587084    | 3.1462204  | 3.1391689  | 3.1811414   | 3.1686345  | 3.1521096               |
|            | z | -2.5395543  | -2.5349313    | -2.5217618 | -2.5351938 | -2.5272511 | -2.5032307 | -2.5267735   | -2.5229000 | -2.5138041 | -2.5408604  | -2.5370622 | -2.5280842              |
| O          | x | -1.6837865  | -1.6820191    | -1.6808978 | -1.5150984 | -1.5168217 | -1.5292937 | -1.6709650   | -1.6708914 | -1.6690212 | -1.7077880  | -1.7071577 | -1.6917942              |
|            | y | 3.6266972   | 3.6133281     | 3.6690640  | 3.7761346  | 3.7596831  | 3.7725454  | 3.5939933    | 3.5798073  | 3.6572572  | 3.5625463   | 3.5485167  | 3.6234841               |
|            | z | 0.8309861   | 0.8290089     | 0.7864037  | 0.8461303  | 0.8438505  | 0.8234058  | 0.8099499    | 0.8085997  | 0.7601097  | 0.8416684   | 0.8403035  | 0.8010889               |
| O          | x | -0.6578890  | -0.6602691    | -0.6576412 | -0.8390249 | -0.8363739 | -0.8237934 | -0.6608065   | -0.6624662 | -0.6691195 | -0.6460471  | -0.6474493 | -0.6447132              |
|            | y | 3.9130443   | 3.8997166     | 3.9076260  | 3.7916894  | 3.7815759  | 3.7842908  | 3.9003110    | 3.8847549  | 3.9028000  | 3.9339042   | 3.9186715  | 3.9260116               |
|            | z | -3.4273641  | -3.4240803    | -3.3883350 | -3.4132902 | -3.4058021 | -3.3664022 | -3.3932541   | -3.3918865 | -3.3616363 | -3.4230706  | -3.4216268 | -3.3925185              |
| C          | x | 1.7705555   | 1.7687003     | 1.7359430  | 1.7621722  | 1.7605019  | 1.7078363  | 1.7519770    | 1.7503879  | 1.7060201  | 1.7678128   | 1.7659134  | 1.7374159               |
|            | y | 2.9553516   | 2.9497787     | 2.9394298  | 2.9555496  | 2.9509727  | 2.9348099  | 2.9181903    | 2.9133705  | 2.9216268  | 2.9343895   | 2.9294247  | 2.9227644               |
|            | z | -0.5989134  | -0.6022929    | -0.6055415 | -0.5735206 | -0.5800855 | -0.5338871 | -0.6066692   | -0.6097149 | -0.6104370 | -0.6126028  | -0.6154790 | -0.6203115              |
| H          | x | 2.5824419   | 2.5796872     | 2.5519180  | 2.5901486  | 2.5873935  | 2.5427990  | 2.5708575    | 2.5689772  | 2.5314261  | 2.5855962   | 2.5835635  | 2.5595577               |
|            | y | 2.6988933   | 2.6947228     | 2.6634698  | 2.6882286  | 2.6831664  | 2.6931479  | 2.6623999    | 2.6591165  | 2.6523822  | 2.6739756   | 2.6704989  | 2.6383335               |
|            | z | -1.2821056  | -1.2858442    | -1.2742381 | -1.2210648 | -1.2280202 | -1.1811909 | -1.2835956   | -1.2868869 | -1.2726322 | -1.3004417  | -1.3033946 | -1.2915283              |
| H          | x | 1.6760359   | 1.6730322     | 1.6425963  | 1.6890391  | 1.6867342  | 1.6185655  | 1.6577895    | 1.6555445  | 1.6109020  | 1.6668707   | 1.6642818  | 1.6402976               |
|            | y | 0.4039478   | 0.4030856     | 4.0232299  | 0.40359130 | 0.40307667 | 0.40135618 | 0.40036574   | 0.39984006 | 0.4069510  | 0.40261033  | 0.40207660 | 0.40143691              |
|            | z | -0.5778467  | -0.5814777    | -0.6142316 | -0.5732428 | -0.5828691 | -0.5117174 | -0.5890177   | -0.5923294 | -0.6149380 | -0.5983031  | -0.6015564 | -0.6382459              |
| H          | x | 2.0502678   | 2.0507873     | 2.0099961  | 2.0258362  | 2.0275227  | 1.9721023  | 2.0296720    | 2.0310523  | 1.9766324  | 2.0501419   | 2.0510101  | 2.0121427               |
|            | y | 2.6328965   | 2.6288966     | 2.6387136  | 2.6586611  | 2.6584323  | 2.6185607  | 2.6026564    | 2.5999260  | 2.6209484  | 2.6178181   | 2.6150087  | 2.6280400               |
|            | z | 0.4052336   | 0.4008772     | 0.4054225  | 0.4372449  | 0.4305137  | 0.4702218  | 0.4014193    | 0.3977423  | 0.4031521  | 0.4011282   | 0.3977288  | 0.4009152               |

Table S2: Rotational constants of  $\text{Cp}^{187}\text{Re}(\text{CH}_3)(\text{CO})(^{14}\text{NO})$  for the  $^{187}\text{Re}$  nucleus at different levels of theory compared to those experimentally observed in Ref. 1. Hartree–Fock and DFT calculations including the LDA, PBE, PBE0 and B3LYP exchange correlation functional were performed at the RECP and two-component ZORA levels for the optimization of the molecular structure employing the basis sets x2c-TZVPPall-2c (x2c3Z), cc-pV5Z on H, C, N and O and cc-pwCVQZ-PP on Re (cc5Z) and def2-TZVPP (def3Z). Calculations with the x2c3Z basis set are on the two-component ZORA level and calculations with the cc5Z and def3Z basis sets are on the RECP level.

| Method                  | A/MHz  | B/MHz  | C/MHz  | $\Delta A/\%$ | $\Delta B/\%$ | $\Delta C/\%$ |
|-------------------------|--------|--------|--------|---------------|---------------|---------------|
| PBE/x2c3Z               | 1254.4 | 914.07 | 765.99 | 1.8           | 1.9           | 2.2           |
| PBE/def3Z               | 1223.6 | 883.90 | 741.46 | −0.7          | −1.5          | −1.1          |
| PBE/cc5Z                | 1225.6 | 891.18 | 746.82 | −0.5          | −0.7          | −0.4          |
| PBE0/x2c3Z              | 1287.8 | 920.10 | 776.31 | 4.5           | 2.6           | 3.5           |
| PBE0/def3Z              | 1252.5 | 892.95 | 752.94 | 1.7           | −0.5          | 0.4           |
| PBE0/cc5Z               | 1254.5 | 900.31 | 758.45 | 1.8           | 0.3           | 1.2           |
| B3LYP/x2c3Z             | 1263.4 | 903.59 | 761.73 | 2.5           | 0.7           | 1.6           |
| B3LYP/def3Z             | 1229.5 | 870.63 | 734.29 | −0.2          | −3.0          | −2.1          |
| B3LYP/cc5Z              | 1232.5 | 877.58 | 739.69 | 0.0           | −2.2          | −1.4          |
| B3LYP/cc5Z <sup>1</sup> | 1232.7 | 878.27 | 740.23 | 0.0           | −2.1          | −1.3          |
| HF/x2c3Z                | 1285.7 | 897.73 | 757.60 | 4.3           | 0.1           | 1.0           |
| HF/def3Z                | 1252.8 | 865.90 | 733.08 | 1.7           | −3.5          | −2.2          |
| HF/cc5Z                 | 1256.9 | 872.68 | 738.97 | 2.0           | −2.7          | −1.4          |
| Experiment <sup>1</sup> | 1232.2 | 897.21 | 749.82 |               |               |               |

Table S3: Distance  $d(\text{Re} - \text{X})$  of the ligands  $\text{X} = \text{Cp}, \text{CH}_3, \text{CO}, \text{NO}$  from the  $^{187}\text{Re}$  nucleus in  $\text{Cp}^{187}\text{Re}(\text{CH}_3)(\text{CO})(^{14}\text{NO})$  at different levels of theory compared to those observed by X-ray diffraction in Ref. 1. Hartree–Fock and DFT calculations including the LDA, PBE, PBE0 and B3LYP exchange correlation functional were performed at the RECP and the two-component ZORA levels for the optimization of the molecular structure employing the basis sets x2c-TZVPPall-2c (x2c3Z), cc-pV5Z on H, C, N and O and cc-pwCVQZ-PP on Re (cc5Z) and def2-TZVPP (def3Z). Calculations with the x2c3Z basis set are on the ZORA level and calculations with the cc5Z and def3Z basis sets are on the RECP level. The distance  $d(\text{Re} - \text{Cp})$  is computed as the distance between Re and the center of mass of the Carbon atoms of the Cp-ring. In the last column, the mean absolute error to experimental data is shown.

| Method                  | $d(\text{Re} - \text{X})/\text{pm}$ |        |        |                     | MAE |
|-------------------------|-------------------------------------|--------|--------|---------------------|-----|
|                         | X = Cp                              | X = CO | X = NO | X = CH <sub>3</sub> |     |
| PBE/x2c3Z               | 225.3                               | 191.3  | 178.0  | 218.2               | 3.5 |
| PBE/def3Z               | 233.8                               | 191.3  | 178.9  | 218.5               | 3.1 |
| PBE/cc5Z                | 232.8                               | 190.7  | 178.2  | 218.0               | 2.8 |
| PBE0/x2c3Z              | 224.5                               | 190.7  | 175.6  | 216.6               | 3.8 |
| PBE0/def3Z              | 232.2                               | 190.9  | 176.8  | 217.1               | 2.8 |
| PBE0/cc5Z               | 231.3                               | 190.3  | 176.0  | 216.6               | 2.5 |
| B3LYP/x2c3Z             | 227.6                               | 192.2  | 176.7  | 218.9               | 3.7 |
| B3LYP/cc5Z              | 235.8                               | 191.6  | 177.1  | 218.8               | 4.2 |
| B3LYP/def3Z             | 236.8                               | 192.3  | 177.8  | 219.3               | 4.5 |
| HF/x2c3Z                | 228.8                               | 197.0  | 173.5  | 219.3               | 5.4 |
| HF/cc5Z                 | 236.6                               | 195.8  | 174.2  | 219.1               | 6.2 |
| HF/def3Z                | 237.5                               | 196.6  | 175.2  | 219.6               | 6.5 |
| Experiment <sup>1</sup> | 230.1                               | 190.4  | 183.2  | 215.1               |     |

**Table S4:** Nuclear electric quadrupole coupling tensors of  $\text{Cp}^{187}\text{Re}(\text{CH}_3)(\text{CO})(^{14}\text{NO})$  for the  $^{187}\text{Re}$  nucleus in the principal axes system at different levels of theory. Hartree-Fock and DFT calculations including the LDA, PBE, PBE0 and B3LYP exchange correlation functional were performed at the RECP and two-component ZORA levels for the optimization of the molecular structure employing the basis sets x2c-TZVPPall-2c (x2c3Z), cc-pV5Z on H, C, N and O and cc-pwCVQZ-PP on Re (cc5Z) and def2-TZVPP (def3Z). Calculations with the x2c3Z basis set are on the ZORA level and calculations with the cc5Z and def3Z basis sets are on the RECP level. The electron density was computed at the level of ZORA with the x2c-TZVPPall-2c basis set for H, C, N and O and an even-tempered basis set on Re including 25 s, 25 p, 14 d, 11 f, and 3 g functions. The NEQC tensors with different methods are presented alongside the relative deviation to the tensor components of the experimental NEQC tensor of  $\text{Cp}^{187}\text{Re}(\text{CH}_3)(\text{CO})(^{14}\text{NO})$  measured in Ref. 1. In the last three columns the asymmetry  $\eta$  of the NEQC tensor, the relative average deviation (RAD) to the experiment and the relative maximum deviation (RMD) to the experiment of all tensor components are shown. The value for the nuclear electric quadrupole moment of  $^{187}\text{Re}$  suggested in Ref. 2  $eQ = 2.070\text{b}$  was used in all calculations.

| Method       |         |                  |                      |                  |                      |                  |                      |                  |                      |                  |                  |                      |        |      |       | $\eta$ | RAD/% | RMD/% |
|--------------|---------|------------------|----------------------|------------------|----------------------|------------------|----------------------|------------------|----------------------|------------------|------------------|----------------------|--------|------|-------|--------|-------|-------|
| Structure    | Density | $\chi_{aa}$ /MHz | $\Delta\chi_{aa}/\%$ | $\chi_{bb}$ /MHz | $\Delta\chi_{bb}/\%$ | $\chi_{cc}$ /MHz | $\Delta\chi_{cc}/\%$ | $\chi_{ab}$ /MHz | $\Delta\chi_{ab}/\%$ | $\chi_{ac}$ /MHz | $\chi_{bc}$ /MHz | $\Delta\chi_{ac}/\%$ |        |      |       |        |       |       |
| PBE/x2c3Z    | LDA     | 684              | 0.4                  | -166             | -18.2                | -519             | 8.7                  | -308             | -11.5                | -42.9            | 119              | -0.4                 | -0.413 | 7.3  | 18.2  |        |       |       |
| PBE/x2c3Z    | PBE     | 596              | -12.5                | -125             | -38.2                | -471             | -1.2                 | -304             | -12.6                | -59.5            | 116              | -2.5                 | -0.420 | 11.7 | 38.2  |        |       |       |
| PBE/x2c3Z    | BLYP    | 620              | -9.0                 | -156             | -23.1                | -464             | -2.7                 | -305             | -12.5                | -47.5            | 120              | 0.3                  | -0.391 | 8.6  | 23.1  |        |       |       |
| PBE/x2c3Z    | PBE0    | 595              | -12.7                | -134             | -33.7                | -461             | -3.4                 | -397             | -14.1                | -85.7            | 137              | 14.8                 | -0.313 | 15.4 | 33.7  |        |       |       |
| PBE/x2c3Z    | B3LYP   | 628              | -7.9                 | -163             | -19.3                | -464             | -2.7                 | -386             | 10.8                 | -69.8            | 139              | 16.1                 | -0.321 | 11.9 | 19.3  |        |       |       |
| PBE/x2c3Z    | BHLYP   | 549              | -19.5                | -190             | -6.2                 | -359             | -24.7                | -508             | 45.9                 | -113             | 153              | 28.5                 | -0.218 | 28.5 | 45.9  |        |       |       |
| PBE/x2c3Z    | HF      | 184              | -73.0                | -288             | 42.5                 | 104              | -121.8               | -732             | 110.2                | -217             | 129              | 7.9                  | -0.963 | 67.6 | 121.8 |        |       |       |
| PBE/def3Z    | LDA     | 956              | 40.3                 | -271             | 34.1                 | -685             | 43.5                 | -345             | -1.0                 | -15.5            | 138              | 15.9                 | -0.396 | 21.7 | 43.5  |        |       |       |
| PBE/def3Z    | PBE     | 860              | 26.1                 | -231             | 14.0                 | -629             | 31.8                 | -342             | -1.9                 | -31.9            | 136              | 13.6                 | -0.404 | 14.7 | 31.8  |        |       |       |
| PBE/def3Z    | BLYP    | 890              | 30.5                 | -266             | 31.4                 | -624             | 30.7                 | -343             | -1.5                 | -18.8            | 138              | 15.5                 | -0.374 | 18.1 | 31.4  |        |       |       |
| PBE/def3Z    | PBE0    | 854              | 25.3                 | -247             | 22.2                 | -606             | 27.1                 | -442             | 26.9                 | -54.8            | 156              | 31.0                 | -0.328 | 27.2 | 31.0  |        |       |       |
| PBE/def3Z    | B3LYP   | 892              | 30.9                 | -279             | 38.1                 | -613             | 28.5                 | -430             | 23.6                 | -39.3            | 158              | 32.2                 | -0.326 | 29.9 | 38.1  |        |       |       |
| PBE/def3Z    | BHLYP   | 814              | 19.4                 | -317             | 56.6                 | -497             | 4.2                  | -568             | 63.2                 | -74.7            | 175              | 46.9                 | -0.253 | 42.9 | 63.2  |        |       |       |
| PBE/def3Z    | HF      | 446              | -34.5                | -435             | 115.1                | -10.9            | -97.7                | -824             | 136.8                | -149             | 156              | 30.7                 | -0.897 | 83.2 | 136.8 |        |       |       |
| PBE/cc5Z     | LDA     | 781              | 14.6                 | -277             | 36.8                 | -504             | 5.7                  | -286             | -17.9                | -31.3            | 95.4             | -20.0                | -0.270 | 19.0 | 36.8  |        |       |       |
| PBE/cc5Z     | PBE     | 842              | 23.5                 | -233             | 15.0                 | -609             | 27.6                 | -331             | -5.0                 | -37.5            | 126              | 5.5                  | -0.385 | 12.5 | 27.6  |        |       |       |
| PBE/cc5Z     | BLYP    | 723              | 6.1                  | -268             | 32.6                 | -455             | -4.7                 | -292             | -16.1                | -37.1            | 98.4             | -17.5                | -0.251 | 15.8 | 32.6  |        |       |       |
| PBE/cc5Z     | PBE0    | 840              | 23.2                 | -248             | 22.4                 | -592             | 24.1                 | -431             | 23.8                 | -61.0            | 147              | 23.0                 | -0.311 | 23.3 | 24.1  |        |       |       |
| PBE/cc5Z     | B3LYP   | 876              | 28.5                 | -280             | 38.5                 | -596             | 24.8                 | -419             | 20.4                 | -45.1            | 148              | 24.2                 | -0.308 | 25.9 | 38.5  |        |       |       |
| PBE/cc5Z     | BHLYP   | 799              | 17.2                 | -315             | 55.9                 | -483             | 1.3                  | -555             | 59.4                 | -80.5            | 165              | 37.9                 | -0.237 | 38.4 | 55.9  |        |       |       |
| PBE/cc5Z     | HF      | 444              | -34.8                | -427             | 111.0                | -17.2            | -96.4                | -809             | 132.3                | -155             | 146              | 22.0                 | -0.879 | 78.7 | 132.3 |        |       |       |
| PBE0/x2c3Z   | LDA     | 618              | -9.4                 | -146             | -28.1                | -472             | -1.1                 | -223             | -36.0                | -32.0            | 85.7             | -28.1                | -0.451 | 23.8 | 36.0  |        |       |       |
| PBE0/x2c3Z   | PBE     | 528              | -22.5                | -102             | -49.4                | -426             | -10.8                | -220             | -36.8                | -49.0            | 83.3             | -30.2                | -0.481 | 30.9 | 49.4  |        |       |       |
| PBE0/x2c3Z   | BLYP    | 552              | -19.1                | -133             | -34.5                | -419             | -12.2                | -222             | -36.3                | -37.0            | 87.5             | -26.6                | -0.432 | 27.4 | 36.3  |        |       |       |
| PBE0/x2c3Z   | PBE0    | 527              | -22.6                | -102             | -49.4                | -425             | -11.0                | -311             | -10.8                | -72.5            | 103              | -13.9                | -0.369 | 18.9 | 49.4  |        |       |       |
| PBE0/x2c3Z   | B3LYP   | 558              | -18.1                | -132             | -34.6                | -426             | -10.8                | -299             | -14.0                | -56.9            | 105              | -11.6                | -0.363 | 16.4 | 34.6  |        |       |       |
| PBE0/x2c3Z   | BHLYP   | 483              | -29.1                | -143             | -29.3                | -340             | -28.7                | -414             | 18.9                 | -94.8            | 120              | 0.9                  | -0.184 | 18.1 | 29.3  |        |       |       |
| PBE0/x2c3Z   | HF      | 151              | -77.8                | -204             | 0.6                  | 52.2             | -110.9               | -623             | 78.9                 | -185             | 108              | -9.6                 | -0.949 | 52.3 | 110.9 |        |       |       |
| PBE0/def3Z   | LDA     | 884              | 29.7                 | -236             | 16.8                 | -648             | 35.8                 | -290             | -16.8                | 3.02             | 104              | -13.2                | -0.416 | 20.3 | 35.8  |        |       |       |
| PBE0/def3Z   | PBE     | 788              | 15.7                 | -193             | -4.6                 | -595             | 24.8                 | -287             | -17.6                | -13.9            | 101              | -15.8                | -0.433 | 16.0 | 24.8  |        |       |       |
| PBE0/def3Z   | BLYP    | 817              | 19.9                 | -227             | 12.0                 | -591             | 23.8                 | -289             | -17.1                | -1.02            | 105              | -12.2                | -0.396 | 16.3 | 23.8  |        |       |       |
| PBE0/def3Z   | PBE0    | 783              | 14.9                 | -199             | -1.8                 | -584             | 22.5                 | -385             | 10.6                 | -34.9            | 121              | 1.5                  | -0.357 | 9.1  | 22.5  |        |       |       |
| PBE0/def3Z   | B3LYP   | 820              | 20.4                 | -232             | 14.5                 | -588             | 23.3                 | -374             | 7.5                  | -19.6            | 124              | 3.6                  | -0.347 | 11.5 | 23.3  |        |       |       |
| PBE0/def3Z   | BHLYP   | 744              | 9.2                  | -252             | 24.6                 | -492             | 3.0                  | -504             | 44.8                 | -51.2            | 141              | 18.0                 | -0.232 | 23.2 | 44.8  |        |       |       |
| PBE0/def3Z   | HF      | 404              | -40.8                | -332             | 64.0                 | -71.7            | -85.0                | -745             | 113.8                | -120             | 131              | 9.9                  | -0.780 | 62.5 | 113.8 |        |       |       |
| PBE0/cc5Z    | LDA     | 719              | 5.5                  | -236             | 16.4                 | -484             | 1.4                  | -236             | -32.3                | -17.1            | 62.0             | -48.1                | -0.289 | 26.3 | 48.1  |        |       |       |
| PBE0/cc5Z    | PBE     | 618              | -9.3                 | -188             | -7.1                 | -430             | -9.8                 | -236             | -32.3                | -36.9            | 59.3             | -50.3                | -0.298 | 27.4 | 50.3  |        |       |       |
| PBE0/cc5Z    | BLYP    | 799              | 17.3                 | -229             | 13.1                 | -570             | 19.5                 | -279             | -19.8                | -6.70            | 95.4             | -20.1                | -0.375 | 18.5 | 20.1  |        |       |       |
| PBE0/cc5Z    | PBE0    | 769              | 12.8                 | -200             | -1.3                 | -569             | 19.3                 | -376             | 7.9                  | -41.3            | 111              | -6.6                 | -0.339 | 8.9  | 19.3  |        |       |       |
| PBE0/cc5Z    | B3LYP   | 624              | -8.5                 | -228             | 12.8                 | -395             | -17.1                | -314             | -9.7                 | -42.2            | 74.2             | -37.8                | -0.182 | 19.1 | 37.8  |        |       |       |
| PBE0/cc5Z    | BHLYP   | 530              | -22.3                | -233             | 15.0                 | -297             | -37.8                | -441             | 26.7                 | -80.1            | 84.2             | -29.5                | -0.206 | 26.8 | 37.8  |        |       |       |
| PBE0/cc5Z    | HF      | 167              | -75.4                | -267             | 31.8                 | 99.2             | -120.8               | -671             | 92.6                 | -160             | 57.7             | -51.6                | -0.848 | 73.8 | 120.8 |        |       |       |
| B3LYP/x2c3Z  | LDA     | 721              | 5.8                  | -191             | -5.6                 | -530             | 11.1                 | -270             | -22.6                | -16.8            | 113              | -5.2                 | -0.426 | 11.2 | 22.6  |        |       |       |
| B3LYP/x2c3Z  | PBE     | 630              | -7.6                 | -149             | -26.5                | -481             | 0.7                  | -265             | -23.8                | -33.4            | 110              | -7.7                 | -0.444 | 14.0 | 26.5  |        |       |       |
| B3LYP/x2c3Z  | BLYP    | 655              | -3.9                 | -179             | -11.4                | -476             | -0.3                 | -265             | -23.9                | -21.0            | 114              | -4.4                 | -0.413 | 10.3 | 23.9  |        |       |       |
| B3LYP/x2c3Z  | PBE0    | 625              | -8.3                 | -149             | -26.3                | -475             | -0.4                 | -357             | 2.6                  | -56.7            | 130              | 9.4                  | -0.362 | 8.4  | 26.3  |        |       |       |
| B3LYP/x2c3Z  | B3LYP   | 659              | -3.4                 | -180             | -11.0                | -479             | 0.3                  | -345             | -0.8                 | -41.1            | 133              | 11.3                 | -0.362 | 5.6  | 11.3  |        |       |       |
| B3LYP/x2c3Z  | BHLYP   | 580              | -14.9                | -194             | -4.4                 | -386             | -19.1                | -464             | 33.3                 | -78.6            | 149              | 24.8                 | -0.249 | 22.1 | 33.3  |        |       |       |
| B3LYP/x2c3Z  | HF      | 228              | -66.6                | -264             | 30.6                 | 36.3             | -107.6               | -679             | 95.0                 | -167             | 134              | 12.5                 | -0.932 | 60.0 | 107.6 |        |       |       |
| B3LYP/Pdef3Z | LDA     | 987              | 44.8                 | -290             | 43.2                 | -697             | 46.1                 | -336             | -3.4                 | 25.3             | 135              | 13.0                 | -0.396 | 23.9 | 46.1  |        |       |       |
| B3LYP/Pdef3Z | PBE     | 888              | 30.3                 | -248             | 22.3                 | -641             | 34.2                 | -333             | -4.4                 | 9.31             | 132              | 10.8                 | -0.408 | 16.7 | 34.2  |        |       |       |
| B3LYP/Pdef3Z | BLYP    | 919              | 34.9                 | -284             | 40.3                 | -635             | 33.1                 | -334             | -4.2                 | 22.6             | 135              | 12.9                 | -0.378 | 20.4 | 40.3  |        |       |       |
| B3LYP/Pdef3Z | PBE0    | 876              | 28.5                 | -255             | 25.9                 | -621             | 30.1                 | -432             | 24.0                 | -8.18            | 154              | 28.9                 | -0.353 | 27.2 | 30.1  |        |       |       |
| B3LYP/Pdef3Z | B3LYP   | 916              | 34.5                 | -289             | 42.6                 | -628             | 31.5                 | -420             | 20.7                 | 6.29             | 156              | 30.6                 | -0.348 | 30.2 | 42.6  |        |       |       |
| B3LYP/Pdef3Z | BHLYP   | 835              | 22.5                 | -312             | 53.9                 | -524             | 9.7                  | -556             | 59.6                 | -20.4            | 177              | 48.4                 | -0.293 | 43.2 | 59.6  |        |       |       |
| B3LYP/Pdef3Z | HF      | 475              | -30.4                | -402             | 98.5                 | -72.8            | -84.7                | -804             | 130.8                | -73.9            | 173              | 45.4                 | -0.836 | 80.9 | 130.8 |        |       |       |
| B3LYP/Pcc5Z  | LDA     | 813              | 19.3                 | -304             | 50.3                 | -509             | 6.6                  | -278             | -20.2                | 15.0             | 91.7             | -23.2                | -0.264 | 23.3 | 50.3  |        |       |       |
| B3LYP/Pcc5Z  | PBE     | 706              | 3.6                  | -258             | 27.2                 | -448             | -6.0                 | -275             | -20.9                | -3.60            | 88.1             | -26.1                | -0.264 | 18.7 | 27.2  |        |       |       |
| B3LYP/Pcc5Z  | BLYP    | 900              | 32.0                 | -287             | 42.0                 | -613             | 28.4                 | -325             | -6.7                 | 18.0             | 126              | 5.3                  | -0.356 | 18.1 | 42.0  |        |       |       |
| B3LYP/Pcc5Z  | PBE0    | 860              | 26.2                 | -257             | 27.1                 | -603             | 26.4                 | -423             | 21.5                 | -13.8            | 144              | 21.0                 | -0.334 | 23.5 | 27.1  |        |       |       |
| B3LYP/Pcc5Z  | B3LYP   | 722              | 5.9                  | -295             | 45.8                 | -426             | -10.6                | -362             | 3.8                  | -8.77            | 108              | -9.6                 | -0.240 | 12.7 | 45.8  |        |       |       |
| B3LYP/Pcc5Z  | BHLYP   | 820              | 20.3                 | -312             | 54.3                 | -507             | 6.3                  | -545             | 56.5                 | -25.7            | 167              | 39.7                 | -0.278 | 39.0 | 56.5  |        |       |       |
| B3LYP/Pcc5Z  | HF      | 239              | -64.9                | -345             | 70.4                 | 105              | -122.1               | -731             | 110.0                | -109             | 101              | -15.2                | -0.825 | 72.5 | 122.1 |        |       |       |
| HF/x2c3Z     | LDA     | 789              | 15.7                 | -113             | -44.0                | -675             | 41.5                 | -83.3            | -76.1                | -8.34            | -33.7            | -128.3               | -0.701 | 72.8 | 128.3 |        |       |       |
| HF/x2c3Z     | PBE     | 694              | 1.8                  | -72.4            | -64.2                | -621             | 30.2                 | -79.7            | -77.1                | -24.5            | -40.8            | -134.2               | -0.780 | 74.1 | 134.2 |        |       |       |
| HF/x2c3Z     | BLYP    | 722              | 5.9                  | -99.5            | -50.8                | -622             | 30.4                 | -74.3            | -78.7                | -11.9            | -31.8            | -126.7               | -0.714 | 71.1 | 126.7 |        |       |       |
| HF/x2c3Z     | PBE0    | 675              | -0.9                 | -40.1            | -80.2                | -635             | 33.1                 | -165             | -52.7                | -32.6            | -31.6            | -126.5               | -0.793 | 67.5 | 126.5 |        |       |       |
| HF/x2c3Z     | B3LYP   | 713              | 4.5                  | -72.0            | -64.4                | -641             | 34.2                 | -151             | -56.7                | -18.7            | -22.3            | -118.7               | -0.733 | 64.9 | 118.7 |        |       |       |
| HF/x2c3Z     | BHLYP   | 624              | -8.5                 | -44.8            | -77.8                | -579             | 21.3                 | -256             | -26.6                | -34.9            | -14.1            | -111.9               | -0.634 | 54.9 | 111.9 |        |       |       |
| HF/x2c3Z     | HF      | 287              | -58.0                | -51.1            | -74.8                | -235             | -50.7                | -434             | 24.5                 | -79.2            | -13.8            | -111.5               | -0.265 | 65.1 | 111.5 |        |       |       |
| HF/def3Z     | LDA     | 1010             | 48.2                 | -168             | -17.0                | -842             | 76.4                 | -218             | -37.4                | -17.5            | -114.7           | -114.7               | -0.606 | 63.7 | 114.7 |        |       |       |
| HF/def3Z     | PBE     | 910              | 33.5                 | -127             | -37.4                | -783             | 64.1                 | -215             | -38.2                | 33.1             | -23.0            | -119.3               | -0.645 | 64.3 | 119.3 |        |       |       |
| HF/def3Z     | BLYP    | 942              | 38.2                 | -161             | -20.7                | -781             | 63.7                 | -212             | -39.1                | 46.8             | -15.5            | -113.0               | -0.593 | 61.0 | 113.0 |        |       |       |
| HF/def3Z     | PBE0    | 887              | 30.2                 | -104             | -48.5                | -783             | 64.1                 | -311             | -10.7                | 30.0             | -12.0            | -110.0               | -      |      |       |        |       |       |

**Table S5:** Nuclear electric quadrupole coupling tensors of  $\text{Cp}^{187}\text{Re}(\text{CH}_3)(\text{CO})(^{14}\text{NO})$  for the  $^{14}\text{N}$  nucleus in the principal axes system at different levels of theory. Hartree-Fock and DFT calculations including the LDA, PBE, PBE0 and B3LYP exchange correlation functional were performed at the RECP and two-component ZORA levels for the optimization of the molecular structure employing the basis sets x2c-TZVPPall-2c (x2c3Z), cc-pV5Z on H, C, N and O and cc-pwCVQZ-PP on Re (cc5Z) and def2-TZVPP (def3Z). Calculations with the x2c3Z basis set are on the ZORA level and calculations with the cc5Z and def3Z basis sets are on the RECP level. The electron density was computed at the level of ZORA with the x2c-TZVPPall-2c basis set for H, C, N and O and an even-tempered basis set on Re including 25 s, 25 p, 14 d, 11 f, and 3 g functions. The NEQC tensors at different methods are presented alongside the relative deviation to the tensor components of the experimental NEQC tensor of  $\text{Cp}^{187}\text{Re}(\text{CH}_3)(\text{CO})(^{14}\text{NO})$  measured in Ref. 1. In the three last columns the asymmetry  $\eta$  of the NEQC tensor, the relative average deviation (RAD) to the experiment and the relative maximum deviation (RMD) to the experiment of all tensor components are shown. The value for the nuclear electric quadrupole moment of  $^{14}\text{N}$  suggested in Ref. 2  $eQ = 0.020\text{b}$  was used in all calculations.

| Method      |         |                        |                      |                        |                      |                        |                      |                        |                        |                        |        |       |       |
|-------------|---------|------------------------|----------------------|------------------------|----------------------|------------------------|----------------------|------------------------|------------------------|------------------------|--------|-------|-------|
| Structure   | Density | $\chi_{aa}/\text{MHz}$ | $\Delta\chi_{aa}/\%$ | $\chi_{bb}/\text{MHz}$ | $\Delta\chi_{bb}/\%$ | $\chi_{cc}/\text{MHz}$ | $\Delta\chi_{cc}/\%$ | $\chi_{ab}/\text{MHz}$ | $\chi_{ac}/\text{MHz}$ | $\chi_{bc}/\text{MHz}$ | $\eta$ | RAD/% | RMD/% |
| PBE/x2c3Z   | LDA     | 0.457                  | -18.4                | 0.517                  | 33.6                 | -0.974                 | 2.8                  | 1.14                   | 0.0864                 | -0.106                 | -0.255 | 18.3  | 33.6  |
| PBE/x2c3Z   | PBE     | 0.495                  | -11.5                | 0.541                  | 39.9                 | -1.04                  | 9.5                  | 1.09                   | 0.0709                 | -0.0832                | -0.321 | 20.3  | 39.9  |
| PBE/x2c3Z   | BLYP    | 0.517                  | -7.8                 | 0.553                  | 42.8                 | -1.07                  | 12.9                 | 1.16                   | 0.0821                 | -0.0897                | -0.297 | 21.2  | 42.8  |
| PBE/x2c3Z   | PBE0    | 0.450                  | -19.7                | 0.560                  | 44.8                 | -1.01                  | 6.7                  | 1.67                   | 0.203                  | -0.155                 | -0.244 | 23.7  | 44.8  |
| PBE/x2c3Z   | B3LYP   | 0.481                  | -14.0                | 0.570                  | 47.4                 | -1.05                  | 11.1                 | 1.64                   | 0.189                  | -0.147                 | -0.222 | 24.2  | 47.4  |
| PBE/x2c3Z   | BHLYP   | 0.528                  | -5.7                 | 0.692                  | 78.8                 | -1.22                  | 28.8                 | 2.42                   | 0.339                  | -0.185                 | -0.312 | 37.8  | 78.8  |
| PBE/x2c3Z   | HF      | 1.07                   | 91.3                 | 1.31                   | 238.0                | -2.38                  | 151.3                | 3.81                   | 0.525                  | 0.0187                 | -0.151 | 160.2 | 238.0 |
| PBE/def3Z   | LDA     | 0.458                  | -18.2                | 0.543                  | 40.3                 | -1.00                  | 5.7                  | 1.09                   | 0.0273                 | -0.118                 | -0.291 | 21.4  | 40.3  |
| PBE/def3Z   | PBE     | 0.496                  | -11.4                | 0.564                  | 45.7                 | -1.06                  | 12.0                 | 1.03                   | 0.00792                | -0.0954                | -0.370 | 23.0  | 45.7  |
| PBE/def3Z   | BLYP    | 0.515                  | -8.0                 | 0.577                  | 49.1                 | -1.09                  | 15.3                 | 1.11                   | 0.0177                 | -0.103                 | -0.338 | 24.1  | 49.1  |
| PBE/def3Z   | PBE0    | 0.453                  | -19.1                | 0.595                  | 53.8                 | -1.05                  | 10.7                 | 1.62                   | 0.150                  | -0.192                 | -0.226 | 27.9  | 53.8  |
| PBE/def3Z   | B3LYP   | 0.482                  | -14.0                | 0.604                  | 56.1                 | -1.09                  | 14.6                 | 1.58                   | 0.132                  | -0.181                 | -0.209 | 28.2  | 56.1  |
| PBE/def3Z   | BHLYP   | 0.533                  | -4.8                 | 0.748                  | 93.2                 | -1.28                  | 35.2                 | 2.38                   | 0.278                  | -0.250                 | -0.291 | 44.4  | 93.2  |
| PBE/def3Z   | HF      | 1.09                   | 95.3                 | 1.42                   | 267.7                | -2.52                  | 165.7                | 3.79                   | 0.378                  | -0.0856                | -0.131 | 176.2 | 267.7 |
| PBE/cc5Z    | LDA     | 0.647                  | 15.5                 | 0.494                  | 27.6                 | -1.14                  | 20.4                 | 0.901                  | -0.0235                | -0.103                 | -0.553 | 21.2  | 27.6  |
| PBE/cc5Z    | PBE     | 0.685                  | 22.3                 | 0.515                  | 33.2                 | -1.20                  | 26.7                 | 0.846                  | -0.0431                | -0.0802                | -0.656 | 27.4  | 33.2  |
| PBE/cc5Z    | BLYP    | 0.704                  | 25.8                 | 0.528                  | 36.5                 | -1.23                  | 30.2                 | 0.921                  | -0.0339                | -0.0881                | -0.602 | 30.8  | 36.5  |
| PBE/cc5Z    | PBE0    | 0.651                  | 16.2                 | 0.543                  | 40.2                 | -1.19                  | 26.0                 | 1.43                   | 0.0988                 | -0.180                 | -0.262 | 27.5  | 40.2  |
| PBE/cc5Z    | B3LYP   | 0.679                  | 21.2                 | 0.552                  | 42.6                 | -1.23                  | 29.9                 | 1.40                   | 0.0808                 | -0.168                 | -0.282 | 31.3  | 42.6  |
| PBE/cc5Z    | BHLYP   | 0.743                  | 32.7                 | 0.691                  | 78.6                 | -1.43                  | 51.4                 | 2.20                   | 0.225                  | -0.240                 | -0.226 | 54.2  | 78.6  |
| PBE/cc5Z    | HF      | 1.32                   | 136.6                | 1.36                   | 251.3                | -2.68                  | 183.5                | 3.62                   | 0.316                  | -0.0779                | -0.139 | 190.5 | 251.3 |
| PBE0/x2c3Z  | LDA     | 0.446                  | -20.3                | 0.456                  | 17.7                 | -0.902                 | -4.8                 | 1.23                   | 0.0841                 | -0.168                 | -0.225 | 14.3  | 20.3  |
| PBE0/x2c3Z  | PBE     | 0.484                  | -13.6                | 0.483                  | 24.8                 | -0.967                 | 2.1                  | 1.17                   | 0.0682                 | -0.147                 | -0.253 | 13.5  | 24.8  |
| PBE0/x2c3Z  | BLYP    | 0.505                  | -9.8                 | 0.490                  | 26.7                 | -0.995                 | 5.1                  | 1.24                   | 0.0781                 | -0.156                 | -0.239 | 13.9  | 26.7  |
| PBE0/x2c3Z  | PBE0    | 0.444                  | -20.7                | 0.478                  | 23.5                 | -0.922                 | -2.7                 | 1.73                   | 0.186                  | -0.224                 | -0.308 | 15.6  | 23.5  |
| PBE0/x2c3Z  | B3LYP   | 0.475                  | -15.2                | 0.488                  | 26.1                 | -0.963                 | 1.7                  | 1.70                   | 0.173                  | -0.218                 | -0.279 | 14.3  | 26.1  |
| PBE0/x2c3Z  | BHLYP   | 0.516                  | -7.9                 | 0.566                  | 46.3                 | -1.08                  | 14.3                 | 2.44                   | 0.303                  | -0.274                 | -0.388 | 22.8  | 46.3  |
| PBE0/x2c3Z  | HF      | 0.983                  | 75.6                 | 1.06                   | 173.3                | -2.04                  | 115.5                | 3.77                   | 0.459                  | -0.170                 | -0.237 | 121.5 | 173.3 |
| PBE0/def3Z  | LDA     | 0.456                  | -18.6                | 0.476                  | 22.9                 | -0.932                 | -1.6                 | 1.17                   | 0.0375                 | -0.180                 | -0.233 | 14.4  | 22.9  |
| PBE0/def3Z  | PBE     | 0.493                  | -12.0                | 0.500                  | 29.2                 | -0.993                 | 4.8                  | 1.11                   | 0.0178                 | -0.158                 | -0.282 | 15.3  | 29.2  |
| PBE0/def3Z  | BLYP    | 0.512                  | -8.5                 | 0.508                  | 31.4                 | -1.02                  | 7.8                  | 1.19                   | 0.0266                 | -0.169                 | -0.260 | 15.9  | 31.4  |
| PBE0/def3Z  | PBE0    | 0.459                  | -18.0                | 0.503                  | 30.0                 | -0.962                 | 1.6                  | 1.68                   | 0.147                  | -0.259                 | -0.286 | 16.5  | 30.0  |
| PBE0/def3Z  | B3LYP   | 0.487                  | -13.0                | 0.513                  | 32.5                 | -1.000                 | 5.6                  | 1.65                   | 0.131                  | -0.250                 | -0.259 | 17.1  | 32.5  |
| PBE0/def3Z  | BHLYP   | 0.539                  | -3.8                 | 0.608                  | 57.0                 | -1.15                  | 21.0                 | 2.41                   | 0.263                  | -0.334                 | -0.365 | 27.3  | 57.0  |
| PBE0/def3Z  | HF      | 1.04                   | 86.2                 | 1.15                   | 198.3                | -2.20                  | 132.0                | 3.77                   | 0.357                  | -0.254                 | -0.203 | 138.8 | 198.3 |
| PBE0/cc5Z   | LDA     | 0.640                  | 14.4                 | 0.450                  | 16.3                 | -1.09                  | 15.2                 | 0.959                  | -0.00445               | -0.167                 | -0.475 | 15.3  | 16.3  |
| PBE0/cc5Z   | PBE     | 0.677                  | 20.9                 | 0.475                  | 22.7                 | -1.15                  | 21.6                 | 0.899                  | -0.0244                | -0.145                 | -0.571 | 21.7  | 22.7  |
| PBE0/cc5Z   | BLYP    | 0.698                  | 24.6                 | 0.483                  | 24.8                 | -1.18                  | 24.7                 | 0.976                  | -0.0160                | -0.155                 | -0.521 | 24.7  | 24.8  |
| PBE0/cc5Z   | PBE0    | 0.653                  | 16.5                 | 0.474                  | 22.5                 | -1.13                  | 19.0                 | 1.47                   | 0.105                  | -0.248                 | -0.271 | 19.3  | 22.5  |
| PBE0/cc5Z   | B3LYP   | 0.680                  | 21.4                 | 0.484                  | 25.2                 | -1.16                  | 22.9                 | 1.44                   | 0.0885                 | -0.239                 | -0.276 | 23.2  | 25.2  |
| PBE0/cc5Z   | BHLYP   | 0.745                  | 33.0                 | 0.575                  | 48.5                 | -1.32                  | 39.3                 | 2.20                   | 0.220                  | -0.325                 | -0.281 | 40.3  | 48.5  |
| PBE0/cc5Z   | HF      | 1.27                   | 127.2                | 1.12                   | 188.2                | -2.39                  | 152.1                | 3.57                   | 0.307                  | -0.246                 | -0.164 | 155.8 | 188.2 |
| B3LYP/x2c3Z | LDA     | 0.507                  | -9.5                 | 0.414                  | 7.0                  | -0.921                 | -2.8                 | 1.16                   | 0.0580                 | -0.161                 | -0.235 | 6.4   | 9.5   |
| B3LYP/x2c3Z | PBE     | 0.542                  | -3.2                 | 0.441                  | 14.1                 | -0.984                 | 3.9                  | 1.10                   | 0.0418                 | -0.140                 | -0.285 | 7.1   | 14.1  |
| B3LYP/x2c3Z | BLYP    | 0.566                  | 1.0                  | 0.447                  | 15.5                 | -1.01                  | 6.9                  | 1.18                   | 0.0514                 | -0.149                 | -0.264 | 7.8   | 15.5  |
| B3LYP/x2c3Z | PBE0    | 0.526                  | -6.1                 | 0.418                  | 8.1                  | -0.944                 | -0.3                 | 1.67                   | 0.162                  | -0.225                 | -0.282 | 4.9   | 8.1   |
| B3LYP/x2c3Z | B3LYP   | 0.554                  | -1.0                 | 0.430                  | 11.1                 | -0.984                 | 3.9                  | 1.64                   | 0.148                  | -0.217                 | -0.255 | 5.4   | 11.1  |
| B3LYP/x2c3Z | BHLYP   | 0.632                  | 12.8                 | 0.490                  | 26.6                 | -1.12                  | 18.4                 | 2.41                   | 0.280                  | -0.280                 | -0.362 | 19.3  | 26.6  |
| B3LYP/x2c3Z | HF      | 1.20                   | 113.4                | 0.981                  | 153.4                | -2.18                  | 129.7                | 3.77                   | 0.425                  | -0.160                 | -0.198 | 132.2 | 153.4 |
| B3LYP/def3Z | LDA     | 0.518                  | -7.6                 | 0.427                  | 10.5                 | -0.945                 | -0.2                 | 1.10                   | -0.0165                | -0.187                 | -0.255 | 6.1   | 10.5  |
| B3LYP/def3Z | PBE     | 0.551                  | -1.5                 | 0.452                  | 16.9                 | -1.00                  | 6.0                  | 1.05                   | -0.0366                | -0.166                 | -0.324 | 8.1   | 16.9  |
| B3LYP/def3Z | BLYP    | 0.574                  | 2.4                  | 0.458                  | 18.4                 | -1.03                  | 9.0                  | 1.12                   | -0.0292                | -0.177                 | -0.294 | 9.9   | 18.4  |
| B3LYP/def3Z | PBE0    | 0.547                  | -2.3                 | 0.431                  | 11.5                 | -0.978                 | 3.3                  | 1.62                   | 0.0878                 | -0.280                 | -0.258 | 5.7   | 11.5  |
| B3LYP/def3Z | B3LYP   | 0.572                  | 2.1                  | 0.443                  | 14.4                 | -1.01                  | 7.2                  | 1.59                   | 0.0712                 | -0.269                 | -0.233 | 7.9   | 14.4  |
| B3LYP/def3Z | BHLYP   | 0.667                  | 19.1                 | 0.513                  | 32.5                 | -1.18                  | 24.6                 | 2.37                   | 0.191                  | -0.370                 | -0.336 | 25.4  | 32.5  |
| B3LYP/def3Z | HF      | 1.27                   | 127.5                | 1.05                   | 171.7                | -2.33                  | 145.6                | 3.76                   | 0.233                  | -0.306                 | -0.165 | 148.3 | 171.7 |
| B3LYP/cc5Z  | LDA     | 0.688                  | 22.8                 | 0.403                  | 4.1                  | -1.09                  | 15.2                 | 0.898                  | -0.0825                | -0.153                 | -0.510 | 14.1  | 22.8  |
| B3LYP/cc5Z  | PBE     | 0.722                  | 28.9                 | 0.428                  | 10.7                 | -1.15                  | 21.4                 | 0.840                  | -0.103                 | -0.132                 | -0.616 | 20.3  | 28.9  |
| B3LYP/cc5Z  | BLYP    | 0.744                  | 32.9                 | 0.434                  | 12.3                 | -1.18                  | 24.5                 | 0.915                  | -0.0960                | -0.143                 | -0.560 | 23.2  | 32.9  |
| B3LYP/cc5Z  | PBE0    | 0.725                  | 29.4                 | 0.405                  | 4.7                  | -1.13                  | 19.3                 | 1.42                   | 0.0210                 | -0.249                 | -0.242 | 17.8  | 29.4  |
| B3LYP/cc5Z  | B3LYP   | 0.749                  | 33.7                 | 0.417                  | 7.8                  | -1.17                  | 23.1                 | 1.39                   | 0.00391                | -0.238                 | -0.256 | 21.6  | 33.7  |
| B3LYP/cc5Z  | BHLYP   | 0.855                  | 52.6                 | 0.486                  | 25.5                 | -1.34                  | 41.5                 | 2.17                   | 0.121                  | -0.341                 | -0.240 | 39.9  | 52.6  |
| B3LYP/cc5Z  | HF      | 1.48                   | 164.3                | 1.02                   | 164.3                | -2.50                  | 164.3                | 3.57                   | 0.152                  | -0.280                 | -0.133 | 164.3 | 164.3 |
| HF/x2c3Z    | LDA     | 0.773                  | 38.0                 | -0.00689               | -101.8               | -0.766                 | -19.1                | 1.18                   | -0.138                 | -0.365                 | -0.256 | 53.0  | 101.8 |
| HF/x2c3Z    | PBE     | 0.793                  | 41.6                 | 0.0391                 | -89.9                | -0.832                 | -12.1                | 1.11                   | -0.150                 | -0.351                 | -0.250 | 47.9  | 89.9  |
| HF/x2c3Z    | BLYP    | 0.831                  | 48.4                 | 0.0226                 | -94.2                | -0.853                 | -9.9                 | 1.19                   | -0.154                 | -0.367                 | -0.243 | 50.8  | 94.2  |
| HF/x2c3Z    | PBE0    | 0.904                  | 61.4                 | -0.138                 | -135.6               | -0.766                 | -19.1                | 1.64                   | -0.105                 | -0.452                 | -0.374 | 72.0  | 135.6 |
| HF/x2c3Z    | B3LYP   | 0.923                  | 64.8                 | -0.119                 | -130.7               | -0.804                 | -15.1                | 1.62                   | -0.118                 | -0.449                 | -0.343 | 70.2  | 130.7 |
| HF/x2c3Z    | BHLYP   | 1.15                   | 105.6                | -0.265                 | -168.6               | -0.886                 | -6.5                 | 2.31                   | -0.0924                | -0.563                 | -0.451 | 93.5  | 168.6 |
| HF/x2c3Z    | HF      | 1.90                   | 238.7                | -0.176                 | -145.4               | -1.72                  | 81.7                 | 3.55                   | -0.158                 | -0.675                 | -0.302 | 155.3 | 238.7 |
| HF/def3Z    | LDA     | 0.703                  | 25.5                 | 0.100                  | -74.1                | -0.803                 | -15.2                | 1.17                   | -0.165                 | -0.370                 | -0.230 | 38.3  | 74.1  |
| HF/def3Z    | PBE     | 0.725                  | 29.5                 | 0.141                  | -63.7                | -0.866                 | -8.6                 | 1.10                   | -0.182                 | -0.354                 | -0.245 | 33.9  | 63.7  |
| HF/def3Z    | BLYP    | 0.759                  | 35.5                 | 0.128                  | -66.8                | -0.887                 | -6.3                 | 1.18                   | -0.186                 | -0.372                 | -0.231 | 36.2  | 66.8  |
| HF/def3Z    | PBE0    | 0.819                  | 46.2                 | -0.00769               | -102.0               | -0.811                 | -14.4                | 1.64                   | -0.123                 | -0.481                 | -0.343 | 54.2  | 102.0 |
| HF/def3Z    | B3LYP   | 0.837                  | 49.5                 | 0.00979                | -97.5                | -0.847                 | -10.6                | 1.62                   | -0.139                 | -0.475                 | -0.313 | 52.5  | 97.5  |
| HF/def3Z    | BHLYP   | 1.05                   | 86.8                 | -0.0945                | -124.4               | -0.952                 | 0.5                  | 2.34                   | -0.110                 | -0.619                 | -0.423 | 70.6  | 124.4 |
| HF/def3Z    | HF      | 1.78                   | 217.2                | 0.0995                 | -74.3                | -1.88                  | 98.1                 | 3.61                   | -0.228                 | -0.756                 | -0.259 | 129.9 | 217.2 |
| HF/cc5Z     | LDA     | 0.883                  | 57.6                 | 0.131                  | -66.2                | -1.01                  | 7.0                  | 0.859                  | -0.215                 | -0.340                 | -0.478 | 43.6  | 66.2  |
| HF/cc5Z     | PBE     | 0.905                  | 61.6                 | 0.171                  | -55.7                | -1.08                  | 13.6                 | 0.793                  | -0.232                 | -0.323                 | -0.578 | 43.6  | 61.6  |
| HF/cc5Z     | BLYP    | 0.939                  | 67.7                 | 0.160                  | -58.7                | -1.10                  | 16.0                 | 0.869                  | -0.236                 | -0.341                 |        |       |       |

Table S6: Cartesian HF and LDA parity-violating energy gradients in units of  $E_h/a_0$  for the equilibrium structure of  $\text{Cp}^{187}\text{Re}(\text{CH}_3)(\text{CO})(\text{NO})$  optimized at the level ZORA-B3LYP/x2c-TZVPPall-2c.

| <b>HF</b>  |                          |                          |                          |
|------------|--------------------------|--------------------------|--------------------------|
| Atom       | $x$                      | $y$                      | $z$                      |
| C          | $4.948 \times 10^{-15}$  | $1.688 \times 10^{-14}$  | $-1.265 \times 10^{-14}$ |
| H          | $-7.899 \times 10^{-16}$ | $1.334 \times 10^{-15}$  | $4.149 \times 10^{-16}$  |
| C          | $1.195 \times 10^{-14}$  | $-2.607 \times 10^{-14}$ | $-1.013 \times 10^{-15}$ |
| H          | $-1.421 \times 10^{-16}$ | $-1.150 \times 10^{-15}$ | $-2.685 \times 10^{-18}$ |
| C          | $-7.557 \times 10^{-16}$ | $-5.847 \times 10^{-15}$ | $7.918 \times 10^{-15}$  |
| H          | $1.951 \times 10^{-16}$  | $5.961 \times 10^{-16}$  | $-4.294 \times 10^{-16}$ |
| C          | $-1.310 \times 10^{-14}$ | $1.518 \times 10^{-14}$  | $-9.603 \times 10^{-16}$ |
| H          | $1.072 \times 10^{-16}$  | $-3.805 \times 10^{-15}$ | $5.688 \times 10^{-17}$  |
| C          | $-2.419 \times 10^{-15}$ | $1.916 \times 10^{-15}$  | $-6.774 \times 10^{-15}$ |
| H          | $-1.311 \times 10^{-16}$ | $-1.647 \times 10^{-15}$ | $5.222 \times 10^{-16}$  |
| Re         | $1.142 \times 10^{-13}$  | $1.011 \times 10^{-14}$  | $-2.401 \times 10^{-14}$ |
| C          | $-5.939 \times 10^{-14}$ | $3.063 \times 10^{-14}$  | $1.444 \times 10^{-14}$  |
| N          | $-5.108 \times 10^{-14}$ | $-2.704 \times 10^{-14}$ | $2.998 \times 10^{-17}$  |
| O          | $1.012 \times 10^{-14}$  | $3.209 \times 10^{-15}$  | $1.056 \times 10^{-14}$  |
| O          | $1.366 \times 10^{-14}$  | $5.431 \times 10^{-15}$  | $1.032 \times 10^{-14}$  |
| C          | $-1.531 \times 10^{-14}$ | $-1.540 \times 10^{-14}$ | $6.190 \times 10^{-15}$  |
| H          | $-4.881 \times 10^{-15}$ | $-2.791 \times 10^{-15}$ | $-1.619 \times 10^{-15}$ |
| H          | $-6.705 \times 10^{-15}$ | $-1.345 \times 10^{-15}$ | $-1.789 \times 10^{-15}$ |
| H          | $-4.976 \times 10^{-16}$ | $-2.117 \times 10^{-16}$ | $-1.213 \times 10^{-15}$ |
| <b>LDA</b> |                          |                          |                          |
| Atom       | $x$                      | $y$                      | $z$                      |
| C          | $8.934 \times 10^{-15}$  | $1.194 \times 10^{-14}$  | $-7.530 \times 10^{-15}$ |
| H          | $-3.237 \times 10^{-16}$ | $6.696 \times 10^{-16}$  | $2.784 \times 10^{-16}$  |
| C          | $4.973 \times 10^{-15}$  | $-1.294 \times 10^{-14}$ | $4.881 \times 10^{-15}$  |
| H          | $-3.912 \times 10^{-16}$ | $-5.075 \times 10^{-16}$ | $8.551 \times 10^{-17}$  |
| C          | $-5.122 \times 10^{-15}$ | $-5.735 \times 10^{-15}$ | $-1.175 \times 10^{-15}$ |
| H          | $1.795 \times 10^{-16}$  | $5.413 \times 10^{-17}$  | $-1.214 \times 10^{-16}$ |
| C          | $-7.169 \times 10^{-15}$ | $5.799 \times 10^{-15}$  | $-2.108 \times 10^{-15}$ |
| H          | $-2.910 \times 10^{-16}$ | $-1.419 \times 10^{-15}$ | $-1.220 \times 10^{-16}$ |
| C          | $5.971 \times 10^{-15}$  | $-9.522 \times 10^{-16}$ | $-1.681 \times 10^{-15}$ |
| H          | $2.187 \times 10^{-16}$  | $6.018 \times 10^{-16}$  | $2.380 \times 10^{-16}$  |
| Re         | $3.536 \times 10^{-14}$  | $3.489 \times 10^{-16}$  | $-2.122 \times 10^{-14}$ |
| C          | $-1.247 \times 10^{-14}$ | $2.081 \times 10^{-14}$  | $1.696 \times 10^{-14}$  |
| N          | $-4.544 \times 10^{-14}$ | $-1.570 \times 10^{-14}$ | $1.270 \times 10^{-14}$  |
| O          | $-7.007 \times 10^{-16}$ | $-3.845 \times 10^{-15}$ | $-9.002 \times 10^{-16}$ |
| O          | $2.426 \times 10^{-14}$  | $4.902 \times 10^{-15}$  | $-2.128 \times 10^{-15}$ |
| C          | $-4.718 \times 10^{-15}$ | $-3.222 \times 10^{-15}$ | $2.888 \times 10^{-15}$  |
| H          | $-1.616 \times 10^{-15}$ | $-1.193 \times 10^{-15}$ | $-9.030 \times 10^{-16}$ |
| H          | $-1.873 \times 10^{-15}$ | $7.211 \times 10^{-18}$  | $8.715 \times 10^{-19}$  |
| H          | $2.149 \times 10^{-16}$  | $3.897 \times 10^{-16}$  | $-1.534 \times 10^{-16}$ |

Table S7: Cartesian HF and LDA parity-violating energy gradients in units of  $E_h/a_0$  for the equilibrium structure of  $\text{Cp}^{185}\text{Re}(\text{CH}_3)(\text{CO})(\text{NO})$  optimized at the level ZORA-B3LYP/x2c-TZVPPall-2c.

| <b>HF</b>  |                          |                          |                          |
|------------|--------------------------|--------------------------|--------------------------|
| Atom       | $x$                      | $y$                      | $z$                      |
| C          | $4.861 \times 10^{-15}$  | $1.659 \times 10^{-14}$  | $-1.242 \times 10^{-14}$ |
| H          | $-7.759 \times 10^{-16}$ | $1.311 \times 10^{-15}$  | $4.076 \times 10^{-16}$  |
| C          | $1.174 \times 10^{-14}$  | $-2.560 \times 10^{-14}$ | $-9.949 \times 10^{-16}$ |
| H          | $-1.396 \times 10^{-16}$ | $-1.130 \times 10^{-15}$ | $-2.653 \times 10^{-18}$ |
| C          | $-7.423 \times 10^{-16}$ | $-5.744 \times 10^{-15}$ | $7.778 \times 10^{-15}$  |
| H          | $1.917 \times 10^{-16}$  | $5.856 \times 10^{-16}$  | $-4.218 \times 10^{-16}$ |
| C          | $-1.287 \times 10^{-14}$ | $1.491 \times 10^{-14}$  | $-9.433 \times 10^{-16}$ |
| H          | $1.053 \times 10^{-16}$  | $-3.737 \times 10^{-15}$ | $5.589 \times 10^{-17}$  |
| C          | $-2.376 \times 10^{-15}$ | $1.882 \times 10^{-15}$  | $-6.654 \times 10^{-15}$ |
| H          | $-1.288 \times 10^{-16}$ | $-1.618 \times 10^{-15}$ | $5.130 \times 10^{-16}$  |
| Re         | $1.122 \times 10^{-13}$  | $9.933 \times 10^{-15}$  | $-2.358 \times 10^{-14}$ |
| C          | $-5.834 \times 10^{-14}$ | $3.009 \times 10^{-14}$  | $1.419 \times 10^{-14}$  |
| N          | $-5.018 \times 10^{-14}$ | $-2.656 \times 10^{-14}$ | $2.950 \times 10^{-17}$  |
| O          | $9.940 \times 10^{-15}$  | $3.152 \times 10^{-15}$  | $1.038 \times 10^{-14}$  |
| O          | $1.342 \times 10^{-14}$  | $5.335 \times 10^{-15}$  | $1.014 \times 10^{-14}$  |
| C          | $-1.504 \times 10^{-14}$ | $-1.512 \times 10^{-14}$ | $6.081 \times 10^{-15}$  |
| H          | $-4.794 \times 10^{-15}$ | $-2.741 \times 10^{-15}$ | $-1.590 \times 10^{-15}$ |
| H          | $-6.586 \times 10^{-15}$ | $-1.321 \times 10^{-15}$ | $-1.757 \times 10^{-15}$ |
| H          | $-4.887 \times 10^{-16}$ | $-2.079 \times 10^{-16}$ | $-1.192 \times 10^{-15}$ |
| <b>LDA</b> |                          |                          |                          |
| Atom       | $x$                      | $y$                      | $z$                      |
| C          | $8.776 \times 10^{-15}$  | $1.173 \times 10^{-14}$  | $-7.397 \times 10^{-15}$ |
| H          | $-3.179 \times 10^{-16}$ | $6.578 \times 10^{-16}$  | $2.735 \times 10^{-16}$  |
| C          | $4.885 \times 10^{-15}$  | $-1.271 \times 10^{-14}$ | $4.795 \times 10^{-15}$  |
| H          | $-3.843 \times 10^{-16}$ | $-4.985 \times 10^{-16}$ | $8.399 \times 10^{-17}$  |
| C          | $-5.031 \times 10^{-15}$ | $-5.634 \times 10^{-15}$ | $-1.154 \times 10^{-15}$ |
| H          | $1.763 \times 10^{-16}$  | $5.317 \times 10^{-17}$  | $-1.193 \times 10^{-16}$ |
| C          | $-7.043 \times 10^{-15}$ | $5.696 \times 10^{-15}$  | $-2.071 \times 10^{-15}$ |
| H          | $-2.858 \times 10^{-16}$ | $-1.394 \times 10^{-15}$ | $-1.198 \times 10^{-16}$ |
| C          | $5.865 \times 10^{-15}$  | $-9.353 \times 10^{-16}$ | $-1.651 \times 10^{-15}$ |
| H          | $2.148 \times 10^{-16}$  | $5.911 \times 10^{-16}$  | $2.338 \times 10^{-16}$  |
| Re         | $3.473 \times 10^{-14}$  | $3.426 \times 10^{-16}$  | $-2.084 \times 10^{-14}$ |
| C          | $-1.225 \times 10^{-14}$ | $2.044 \times 10^{-14}$  | $1.666 \times 10^{-14}$  |
| N          | $-4.464 \times 10^{-14}$ | $-1.543 \times 10^{-14}$ | $1.248 \times 10^{-14}$  |
| O          | $-6.883 \times 10^{-16}$ | $-3.777 \times 10^{-15}$ | $-8.842 \times 10^{-16}$ |
| O          | $2.383 \times 10^{-14}$  | $4.816 \times 10^{-15}$  | $-2.090 \times 10^{-15}$ |
| C          | $-4.634 \times 10^{-15}$ | $-3.165 \times 10^{-15}$ | $2.837 \times 10^{-15}$  |
| H          | $-1.588 \times 10^{-15}$ | $-1.172 \times 10^{-15}$ | $-8.870 \times 10^{-16}$ |
| H          | $-1.840 \times 10^{-15}$ | $7.075 \times 10^{-18}$  | $8.572 \times 10^{-19}$  |
| H          | $2.111 \times 10^{-16}$  | $3.829 \times 10^{-16}$  | $-1.506 \times 10^{-16}$ |

Table S8: Parity violating (PV) energy  $E_{\text{PV}}$  and relative PV shifts of rotational constants ( $\Delta X/X$ ) of  $\text{Cp}^{187}\text{Re}(\text{CH}_3)(\text{CO})(\text{NO})$  and  $\text{Cp}^{185}\text{Re}(\text{CH}_3)(\text{CO})(\text{NO})$  optimized at the level ZORA-B3LYP/x2c-TZVPPall-2c.

| Method | $\text{Cp}^{187}\text{Re}(\text{CH}_3)(\text{CO})(\text{NO})$ |                             |                             | $\text{Cp}^{185}\text{Re}(\text{CH}_3)(\text{CO})(\text{NO})$ |                             |                             |
|--------|---------------------------------------------------------------|-----------------------------|-----------------------------|---------------------------------------------------------------|-----------------------------|-----------------------------|
|        | $E_{\text{PV}} \times 10^9/\text{cm}^{-1} \text{ } hc$        |                             |                             |                                                               |                             |                             |
| HF     | 1.281                                                         |                             |                             | 1.259                                                         |                             |                             |
| B3LYP  | 1.554                                                         |                             |                             | 1.527                                                         |                             |                             |
| BLYP   | 1.408                                                         |                             |                             | 1.383                                                         |                             |                             |
| LDA    | 1.391                                                         |                             |                             | 1.367                                                         |                             |                             |
|        | $\Delta A/A \times 10^{14}$                                   | $\Delta B/B \times 10^{14}$ | $\Delta C/C \times 10^{14}$ | $\Delta A/A \times 10^{14}$                                   | $\Delta B/B \times 10^{14}$ | $\Delta C/C \times 10^{14}$ |
| HF     | 2.017                                                         | −5.257                      | 1.994                       | 1.989                                                         | −5.161                      | 1.958                       |
| LDA    | −1.383                                                        | 1.046                       | −1.494                      | −1.358                                                        | 1.027                       | −1.467                      |

Table S9: Unscaled harmonic vibrational wavenumbers  $\tilde{\omega}$  (in  $\text{cm}^{-1}$ ) as obtained for the equilibrium structure of  $\text{Cp}^{187}\text{Re}(\text{CH}_3)(\text{CO})(\text{NO})$  and  $\text{Cp}^{185}\text{Re}(\text{CH}_3)(\text{CO})(\text{NO})$  optimized at the level ZORA-B3LYP/x2c-TZVPPall-2c. Masses used (in  $u$ ) for the harmonic force field calculation are 1.008, 12.000, 14.003, 15.995, 184.953, and 186.956 respectively for H, C, N, O,  $^{185}\text{Re}$  and  $^{187}\text{Re}$  atoms.

| Modes→     | $\text{Cp}^{187}\text{Re}(\text{CH}_3)(\text{CO})(\text{NO})$ | $\text{Cp}^{185}\text{Re}(\text{CH}_3)(\text{CO})(\text{NO})$ |
|------------|---------------------------------------------------------------|---------------------------------------------------------------|
| $\nu_1$    | 3267.47                                                       | 3267.47                                                       |
| $\nu_2$    | 3258.71                                                       | 3258.71                                                       |
| $\nu_3$    | 3255.76                                                       | 3255.76                                                       |
| $\nu_4$    | 3243.95                                                       | 3243.95                                                       |
| $\nu_5$    | 3240.99                                                       | 3240.99                                                       |
| $\nu_6$    | 3117.23                                                       | 3117.23                                                       |
| $\nu_7$    | 3086.31                                                       | 3086.31                                                       |
| $\nu_8$    | 3018.16                                                       | 3018.16                                                       |
| $\nu_9$    | 2032.97                                                       | 2032.97                                                       |
| $\nu_{10}$ | 1791.25                                                       | 1791.26                                                       |
| $\nu_{11}$ | 1492.13                                                       | 1492.13                                                       |
| $\nu_{12}$ | 1484.22                                                       | 1484.22                                                       |
| $\nu_{13}$ | 1462.37                                                       | 1462.37                                                       |
| $\nu_{14}$ | 1461.28                                                       | 1461.28                                                       |
| $\nu_{15}$ | 1399.08                                                       | 1399.08                                                       |
| $\nu_{16}$ | 1387.66                                                       | 1387.66                                                       |
| $\nu_{17}$ | 1269.03                                                       | 1269.03                                                       |
| $\nu_{18}$ | 1263.73                                                       | 1263.74                                                       |
| $\nu_{19}$ | 1141.93                                                       | 1141.93                                                       |
| $\nu_{20}$ | 1088.06                                                       | 1088.06                                                       |
| $\nu_{21}$ | 1078.56                                                       | 1078.56                                                       |
| $\nu_{22}$ | 1028.36                                                       | 1028.36                                                       |
| $\nu_{23}$ | 1017.95                                                       | 1017.95                                                       |
| $\nu_{24}$ | 924.37                                                        | 924.37                                                        |
| $\nu_{25}$ | 914.77                                                        | 914.77                                                        |
| $\nu_{26}$ | 854.99                                                        | 855.00                                                        |
| $\nu_{27}$ | 847.33                                                        | 847.34                                                        |
| $\nu_{28}$ | 842.90                                                        | 842.90                                                        |
| $\nu_{29}$ | 841.26                                                        | 841.27                                                        |
| $\nu_{30}$ | 832.33                                                        | 832.35                                                        |
| $\nu_{31}$ | 827.93                                                        | 827.93                                                        |
| $\nu_{32}$ | 814.90                                                        | 814.93                                                        |
| $\nu_{33}$ | 659.98                                                        | 660.13                                                        |
| $\nu_{34}$ | 628.66                                                        | 628.73                                                        |
| $\nu_{35}$ | 616.99                                                        | 617.01                                                        |
| $\nu_{36}$ | 607.62                                                        | 607.75                                                        |
| $\nu_{37}$ | 587.63                                                        | 587.97                                                        |
| $\nu_{38}$ | 535.10                                                        | 535.32                                                        |
| $\nu_{39}$ | 510.35                                                        | 510.52                                                        |
| $\nu_{40}$ | 496.83                                                        | 496.90                                                        |
| $\nu_{41}$ | 475.89                                                        | 476.11                                                        |
| $\nu_{42}$ | 394.42                                                        | 394.56                                                        |
| $\nu_{43}$ | 363.11                                                        | 363.31                                                        |
| $\nu_{44}$ | 348.76                                                        | 349.11                                                        |
| $\nu_{45}$ | 236.53                                                        | 236.54                                                        |
| $\nu_{46}$ | 180.20                                                        | 180.27                                                        |
| $\nu_{47}$ | 131.18                                                        | 131.26                                                        |
| $\nu_{48}$ | 101.85                                                        | 101.93                                                        |
| $\nu_{49}$ | 94.71                                                         | 94.76                                                         |
| $\nu_{50}$ | 77.45                                                         | 77.48                                                         |
| $\nu_{51}$ | 52.83                                                         | 52.83                                                         |

Table S10: Harmonic force field data [Cartesian force constant matrix] in  $E_h/a_0^2$  for the equilibrium structure of  $\text{Cp}^{187}\text{Re}(\text{CH}_3)(\text{CO})(\text{NO})$  at level of ZORA-B3LYP/x2c-TZVPPall-2c.

| Atom |    | 1C         |            |            | 2H         |            |            | 3C         |            |            | 4H         |            |            |
|------|----|------------|------------|------------|------------|------------|------------|------------|------------|------------|------------|------------|------------|
|      |    | dx         | dy         | dz         |
| 1C   | dx | 0.5240938  |            |            |            |            |            |            |            |            |            |            |            |
|      | dy | 0.0140675  | 0.1413143  |            |            |            |            |            |            |            |            |            |            |
|      | dz | -0.0152326 | -0.0299044 | 0.8132792  |            |            |            |            |            |            |            |            |            |
| 2H   | dx | -0.0559330 | -0.0017651 | -0.0016261 | 0.0487697  |            |            |            |            |            |            |            |            |
|      | dy | -0.0022067 | -0.0254568 | -0.0009540 | 0.0008084  | 0.0249750  |            |            |            |            |            |            |            |
|      | dz | -0.0011327 | 0.0031689  | -0.3575062 | 0.0011062  | -0.0002107 | 0.3718430  |            |            |            |            |            |            |
| 3C   | dx | -0.2388477 | -0.0111496 | 0.1058908  | 0.0077773  | -0.0001879 | -0.0033306 | 0.7963490  |            |            |            |            |            |
|      | dy | 0.0047023  | -0.0411010 | 0.0025995  | -0.0003432 | -0.0025576 | -0.0001490 | 0.0135032  | 0.1471508  |            |            |            |            |
|      | dz | 0.0900740  | 0.0186897  | -0.1717110 | 0.0236789  | -0.0035702 | -0.0075476 | 0.0860848  | 0.0056021  | 0.5695921  |            |            |            |
| 4H   | dx | -0.0118164 | -0.0008784 | -0.0097823 | 0.0004257  | 0.0000835  | 0.0003833  | -0.3254217 | -0.0184774 | -0.0890261 | 0.3380038  |            |            |
|      | dy | -0.0011250 | -0.0013484 | -0.0024696 | 0.0003178  | -0.0018354 | -0.0000894 | -0.0240123 | -0.0320777 | -0.0080192 | 0.0227527  | 0.0282363  |            |
|      | dz | 0.0174901  | 0.0014918  | 0.0122840  | -0.0009233 | 0.0002485  | 0.0002347  | -0.0887994 | -0.0061535 | -0.0873482 | 0.0956055  | 0.0075904  | 0.0821951  |
| 5C   | dx | 0.0083377  | -0.0113043 | 0.0148427  | -0.0054877 | 0.0002528  | 0.0016345  | -0.1211590 | 0.0080556  | -0.0525319 | 0.0005685  | -0.0021342 | -0.0263794 |
|      | dy | -0.0178597 | 0.0065995  | 0.0060721  | -0.0002277 | 0.0025007  | -0.0001039 | 0.0014548  | -0.0397634 | -0.0187300 | 0.0002851  | -0.0010547 | -0.0015215 |
|      | dz | 0.0315883  | -0.0148673 | -0.0538172 | 0.0028006  | 0.0005321  | -0.0005348 | -0.0697350 | 0.0025651  | -0.2900818 | 0.0010054  | 0.0015223  | 0.0001658  |
| 6H   | dx | -0.0018661 | -0.0001381 | -0.0036927 | 0.0010575  | 0.0002195  | -0.0003807 | 0.0122803  | 0.0000297  | -0.0089937 | 0.0001193  | 0.0001748  | 0.0007313  |
|      | dy | 0.0003579  | 0.0029258  | -0.0004361 | 0.0001907  | 0.0014390  | 0.0000931  | -0.0023215 | -0.0027480 | 0.0022613  | 0.0001607  | -0.0018078 | -0.0000361 |
|      | dz | -0.0026835 | 0.0001421  | -0.0044753 | 0.0012789  | 0.0000893  | -0.0002354 | 0.0181009  | 0.0001178  | -0.0115063 | -0.0005180 | 0.0002036  | 0.0005245  |
| 7C   | dx | -0.2132305 | -0.0010671 | -0.0888520 | 0.0078142  | 0.0015047  | 0.0031600  | -0.0608895 | -0.0106752 | 0.0081886  | -0.0020681 | -0.0001429 | 0.0038035  |
|      | dy | -0.0257529 | -0.0366303 | -0.0058656 | 0.0009722  | -0.0027409 | 0.0001080  | 0.0072142  | 0.0041560  | -0.0120578 | -0.0002445 | 0.0031590  | -0.0004861 |
|      | dz | -0.0794549 | 0.0106068  | -0.1607391 | -0.0224469 | -0.0036690 | -0.0063356 | -0.0084394 | -0.0111348 | 0.0158268  | 0.0026076  | -0.0001526 | -0.0033187 |
| 8H   | dx | -0.0107030 | -0.0009327 | 0.0092983  | 0.0002625  | 0.0002912  | -0.0003940 | -0.0023149 | -0.0005695 | -0.0027553 | -0.0002428 | -0.0000730 | 0.0007192  |
|      | dy | 0.0034039  | -0.0024030 | -0.0016189 | -0.0000781 | -0.0011512 | -0.0000927 | -0.0000895 | 0.0027071  | 0.0002117  | 0.0000589  | 0.0011735  | 0.0000517  |
|      | dz | -0.0161399 | -0.0021937 | 0.0125351  | 0.0005343  | 0.0002198  | 0.0001797  | -0.0038723 | -0.0002357 | -0.0043107 | -0.0006614 | 0.0003112  | 0.0009969  |
| 9C   | dx | 0.0055358  | 0.0099594  | -0.0129275 | -0.0057146 | -0.0005126 | -0.0018250 | -0.0334617 | -0.0161329 | -0.0495770 | 0.0004759  | -0.0002583 | -0.0011433 |
|      | dy | 0.0139893  | 0.0036111  | 0.0037814  | -0.0006398 | 0.0032527  | -0.0000907 | -0.0008339 | 0.0073848  | 0.0139972  | -0.0003861 | 0.0030426  | 0.0002900  |
|      | dz | -0.0275185 | -0.0166619 | -0.0518680 | -0.0028124 | -0.0002944 | -0.0005510 | -0.0290530 | 0.0023411  | -0.0095059 | 0.0003212  | 0.0003467  | -0.0062528 |
| 10H  | dx | -0.0017645 | 0.0001334  | 0.0037256  | 0.0010045  | -0.0002622 | 0.0003474  | -0.0066488 | -0.0007190 | 0.0011446  | 0.0002159  | 0.0003289  | -0.0013529 |
|      | dy | -0.0006569 | 0.0030595  | 0.0004857  | -0.0001793 | 0.0011818  | 0.0001892  | 0.0000662  | 0.0034360  | -0.0005656 | 0.0000569  | 0.0012395  | -0.0001284 |
|      | dz | 0.0024529  | 0.0000697  | -0.0044547 | -0.0011681 | -0.0000819 | -0.0001941 | 0.0023348  | 0.0003819  | -0.0002451 | 0.0000662  | -0.0003506 | 0.0005334  |
| 11Re | dx | -0.0090006 | 0.0012567  | -0.0020682 | -0.0004095 | -0.0000555 | 0.0003207  | -0.0278863 | 0.0143228  | -0.0053822 | -0.0003061 | 0.0037606  | 0.0001796  |
|      | dy | 0.0090907  | -0.0327999 | 0.0183276  | 0.0009910  | 0.0012853  | -0.0030816 | 0.0151887  | -0.0322505 | -0.0009754 | -0.0016888 | 0.0032861  | -0.0008678 |
|      | dz | 0.0030126  | 0.0103384  | -0.0399887 | -0.0001586 | 0.0098887  | 0.0005109  | -0.0100113 | -0.0014845 | 0.0010119  | 0.0002673  | 0.0007393  | -0.0002145 |
| 12C  | dx | 0.0046789  | 0.0044034  | 0.0065230  | 0.0005578  | -0.0012418 | -0.0000875 | 0.0003117  | 0.0040770  | -0.0024640 | -0.0000704 | 0.0000056  | 0.0000723  |
|      | dy | 0.0007370  | -0.0027272 | 0.0018276  | -0.0003628 | 0.0005024  | -0.0004583 | 0.0043465  | -0.0005189 | -0.0028238 | -0.0000980 | -0.0004781 | 0.0003329  |
|      | dz | -0.0075572 | -0.0005259 | 0.0031160  | -0.0007764 | 0.0005820  | 0.0000364  | 0.0024942  | -0.0006772 | -0.0045374 | 0.0001149  | -0.0002114 | 0.0002291  |
| 13N  | dx | 0.0043908  | -0.0033320 | -0.0027447 | 0.0001419  | 0.0005583  | -0.0000767 | -0.0026889 | 0.0070950  | 0.0039254  | -0.0001594 | -0.0004062 | -0.0000789 |
|      | dy | 0.0025933  | -0.0147541 | 0.0119744  | -0.0000035 | -0.0022687 | 0.0003369  | 0.0035788  | -0.0077103 | 0.0080705  | 0.0002876  | -0.0010773 | -0.0002113 |
|      | dz | -0.0025049 | 0.0217393  | 0.0059785  | 0.0001231  | -0.0025559 | -0.0002732 | 0.0007872  | 0.0086047  | -0.0067806 | 0.0001505  | 0.0001045  | 0.0000204  |
| 14O  | dx | -0.0015651 | -0.0020656 | -0.0027232 | -0.0003280 | 0.0007838  | 0.0002236  | 0.0002688  | -0.0003275 | 0.0020568  | 0.0000823  | 0.0000800  | 0.0000148  |
|      | dy | -0.0003118 | 0.0014575  | 0.0008583  | 0.0001143  | -0.0006216 | 0.0001000  | -0.0010548 | -0.0007972 | -0.0002967 | 0.0000100  | 0.0001790  | -0.0001013 |
|      | dz | 0.0025215  | 0.0006598  | -0.0002862 | 0.0003500  | -0.0008088 | 0.0003968  | -0.0010615 | -0.0012664 | 0.0006788  | 0.0001896  | 0.0000443  | 0.0000054  |
| 15O  | dx | -0.0014854 | 0.0027518  | 0.0003878  | -0.0000212 | 0.0000483  | -0.0001001 | 0.0023873  | -0.0035043 | -0.0016228 | 0.0000026  | 0.0002667  | -0.0000389 |
|      | dy | -0.0002269 | 0.0000626  | -0.0045082 | -0.0000530 | 0.0007760  | 0.0001452  | -0.0025220 | 0.0005068  | -0.0017331 | 0.0001140  | 0.0002934  | 0.0000796  |
|      | dz | -0.0002770 | -0.0023863 | -0.0030060 | 0.0000080  | 0.0011346  | -0.0006640 | 0.0011890  | 0.0005215  | 0.0014064  | -0.0009543 | 0.0002870  | -0.0002938 |
| 16C  | dx | -0.0019043 | 0.0003539  | -0.0004254 | 0.0003345  | 0.0000094  | 0.0001306  | 0.0000485  | -0.0025271 | -0.0047392 | -0.0004967 | 0.0012256  | -0.0004311 |
|      | dy | -0.0001752 | -0.0012364 | 0.0002957  | 0.0002700  | 0.0004612  | -0.0005776 | -0.0020493 | -0.0060246 | -0.0000252 | -0.0021263 | -0.0005641 | -0.0004999 |
|      | dz | 0.0070835  | -0.0008779 | 0.0001650  | 0.0001881  | -0.0001437 | 0.0000012  | -0.0044267 | -0.0026145 | 0.0070185  | -0.0002944 | 0.0005108  | 0.0006394  |
| 17H  | dx | -0.0004588 | 0.0001729  | 0.0002617  | -0.0003162 | -0.0000719 | -0.0001444 | 0.0006389  | 0.0007999  | -0.0011514 | 0.0003451  | -0.0003159 | 0.0002337  |
|      | dy | -0.0018870 | -0.0001553 | 0.0000379  | 0.0000181  | -0.0000332 | 0.0006259  | 0.0000330  | 0.0003906  | -0.0000424 | 0.0001359  | -0.0001292 | 0.0003547  |
|      | dz | -0.0003490 | 0.0000004  | -0.0011050 | -0.0000767 | -0.0002386 | 0.0011377  | 0.0005344  | -0.0008273 | -0.0012318 | 0.0000577  | 0.0006040  | -0.0001595 |
| 18H  | dx | 0.0000278  | -0.0001509 | -0.0008591 | 0.0000612  | 0.0001953  | -0.0000274 | -0.0002633 | 0.0013159  | 0.0015706  | 0.0000749  | -0.0007908 | 0.0001222  |
|      | dy | -0.0001111 | -0.0002834 | -0.0003142 | -0.0000044 | 0.0001456  | -0.0000269 | 0.0002639  | -0.0003939 | 0.0001674  | -0.0002875 | -0.0000267 | -0.0000866 |
|      | dz | -0.0009268 | 0.0001689  | 0.0012367  | -0.0000433 | -0.0000669 | -0.0005425 | 0.00011630 | 0.0003897  | -0.0003773 | 0.0000675  | -0.0002683 | -0.0000927 |
| 19H  | dx | 0.0015104  | -0.0003151 | 0.0000038  | 0.0000033  | -0.0002168 | 0.0001928  | -0.0004799 | -0.0006255 | 0.0015199  | 0.0002675  | 0.0003458  | 0.0001752  |
|      | dy | 0.0013712  | -0.0001345 | -0.0001892 | -0.0000255 | 0.0001457  | 0.0001137  | -0.0014285 | 0.0002110  | -0.0001605 | 0.0002418  | -0.0002101 | -0.0003472 |
|      | dz | -0.0004458 | 0.0003414  | 0.0003627  | -0.0000362 | -0.0003010 | 0.0000440  | 0.0001500  | 0.0014196  | -0.0003508 | 0.0004000  | -0.0007029 | -0.0001485 |

Table S10: Harmonic force field data [Cartesian force constant matrix] in  $E_h/a_0^2$  for the equilibrium structure of  $\text{Cp}^{187}\text{Re}(\text{CH}_3)(\text{CO})(\text{NO})$  at level of ZORA-B3LYP/x2c-TZVPPall-2c. (continued).

| Atom |    | 5C         |            | 6H         |            | 7C         |            | 8H        |            |
|------|----|------------|------------|------------|------------|------------|------------|-----------|------------|
|      | dx | dy         | dz         | dx         | dy         | dz         | dx         | dy        | dz         |
| 5C   | dx | 0.6180057  |            |            |            |            |            |           |            |
|      | dy | -0.0038377 | 0.1383883  |            |            |            |            |           |            |
|      | dz | -0.1343704 | 0.0250312  | 0.7218198  |            |            |            |           |            |
| 6H   | dx | -0.1640009 | -0.0023221 | 0.1445044  | 0.1634470  |            |            |           |            |
|      | dy | -0.0038079 | -0.0250112 | 0.0020701  | 0.0023852  | 0.0247565  |            |           |            |
|      | dz | 0.1440414  | -0.0008630 | -0.2492833 | -0.1547944 | -0.0019025 | 0.2561934  |           |            |
| 7C   | dx | -0.0306613 | -0.0019047 | 0.0252237  | -0.0056399 | -0.0009089 | -0.0023013 | 0.7710623 |            |
|      | dy | 0.0139300  | 0.0039689  | 0.0062565  | -0.0008055 | 0.0036117  | -0.0004263 | 0.0739303 | 0.1445054  |
|      | dz | 0.0384431  | 0.0187926  | -0.0102988 | -0.0015405 | 0.0001941  | -0.0003630 | 0.0975607 | -0.0201514 |
| 8H   | dx | -0.0070396 | -0.0072014 | -0.1000193 | 0.0220219  | 0.0038205  | 0.0074422  | 0.0681501 | 0.0135421  |
|      | dy | 0.0005249  | 0.0026482  | -0.0010055 | 0.0000634  | 0.0010284  | -0.0001971 | 0.0252653 | -0.0253508 |
|      | dz | 0.0006594  | 0.0001148  | -0.0057677 | 0.0013918  | 0.0001151  | 0.0007240  | 0.0882710 | 0.0077559  |
| 9C   | dx | -0.2877711 | 0.0031328  | 0.0074041  | -0.0057689 | -0.0006561 | -0.0029759 | 0.1177130 | -0.0151683 |
|      | dy | -0.0248289 | -0.0360775 | -0.0070259 | 0.0005097  | -0.0026597 | 0.0000390  | 0.0008072 | -0.0399688 |
|      | dz | -0.0070396 | -0.0072014 | -0.1000193 | 0.0220219  | 0.0038205  | 0.0074422  | 0.0681501 | 0.0135421  |
| 10H  | dx | -0.0055948 | -0.0010865 | -0.0231672 | 0.0000337  | 0.0002512  | 0.0003298  | 0.0121696 | 0.0004198  |
|      | dy | 0.0005414  | -0.0031921 | 0.0025149  | -0.0001984 | -0.0011452 | -0.0000244 | 0.0034818 | -0.0018446 |
|      | dz | 0.0025742  | 0.0005944  | 0.0075656  | -0.0003788 | -0.0000023 | 0.0002329  | 0.0170880 | -0.0003770 |
| 11Re | dx | -0.0206601 | 0.0128611  | 0.0183176  | -0.0006642 | 0.0068683  | 0.0001153  | 0.0391353 | -0.0266933 |
|      | dy | 0.0166673  | -0.0359561 | -0.0155259 | 0.0000910  | -0.0003909 | 0.0034555  | 0.0387194 | -0.0423669 |
|      | dz | 0.0192625  | -0.0097190 | -0.0227590 | 0.0016972  | -0.0075728 | 0.0002661  | 0.0078322 | 0.0109581  |
| 12C  | dx | 0.0058077  | 0.0058836  | 0.0005860  | 0.0001415  | -0.0012817 | 0.0002713  | 0.0006184 | 0.0024270  |
|      | dy | 0.0046780  | -0.0110813 | -0.0043870 | -0.0002453 | -0.0013395 | -0.0003563 | 0.0067855 | -0.0080707 |
|      | dz | -0.0009729 | -0.0152057 | 0.0006180  | -0.0003564 | 0.0011882  | -0.0004531 | 0.0117704 | -0.0069358 |
| 13N  | dx | 0.0039971  | 0.0033748  | -0.0094986 | -0.0000785 | -0.0017450 | 0.0002645  | 0.0048219 | 0.0015631  |
|      | dy | 0.0008471  | -0.0016332 | 0.0049714  | -0.0004271 | 0.0018907  | -0.0002742 | 0.0024657 | -0.0038230 |
|      | dz | 0.0037761  | 0.0035915  | 0.0052502  | 0.0001862  | -0.0008861 | 0.0003984  | 0.0028853 | 0.0063032  |
| 14O  | dx | -0.0027183 | 0.0016568  | -0.0002302 | -0.0001543 | 0.0006307  | -0.0000511 | 0.0014359 | -0.0021769 |
|      | dy | -0.0010715 | -0.0002970 | 0.0015157  | 0.0000305  | 0.0003963  | 0.0002516  | 0.0042375 | 0.0033993  |
|      | dz | 0.0012165  | -0.0004740 | -0.0002850 | 0.0002170  | -0.0003708 | 0.0000640  | 0.0057372 | 0.0039208  |
| 15O  | dx | -0.0005681 | -0.0010852 | 0.0033059  | 0.0000028  | 0.0006781  | 0.0000067  | 0.0005865 | 0.0012077  |
|      | dy | 0.0008766  | 0.0002526  | -0.0032528 | 0.0002587  | -0.0013775 | -0.0000126 | 0.0006987 | -0.0011869 |
|      | dz | -0.0024124 | -0.0011739 | -0.0012328 | -0.0006337 | 0.0010026  | 0.0004654  | 0.0004387 | 0.0007043  |
| 16C  | dx | 0.0022094  | -0.0011770 | 0.0037186  | 0.0010104  | 0.0002422  | -0.0008081 | 0.0014064 | -0.0033958 |
|      | dy | 0.0004469  | 0.0000289  | -0.0002589 | 0.0002604  | 0.0001060  | -0.0000905 | 0.0001952 | 0.0005285  |
|      | dz | -0.0030344 | 0.0009172  | -0.0019286 | -0.0001721 | 0.0002366  | -0.0000491 | 0.0023705 | -0.0026900 |
| 17H  | dx | 0.0006385  | 0.0000753  | 0.0002613  | 0.0000185  | -0.0004795 | -0.0001481 | 0.0005118 | -0.0005011 |
|      | dy | 0.0003976  | -0.0001909 | -0.0003321 | 0.0000444  | 0.0001930  | -0.0002121 | 0.0001575 | -0.0010289 |
|      | dz | 0.0007516  | -0.0002010 | 0.0009199  | 0.0001383  | -0.0000201 | -0.0000683 | 0.0002443 | -0.0009695 |
| 18H  | dx | -0.0005912 | 0.0003832  | -0.0010008 | -0.0000730 | -0.0000292 | -0.0000386 | 0.0005281 | -0.0001183 |
|      | dy | -0.0002726 | 0.0000470  | 0.0003355  | -0.0000200 | 0.0000136  | 0.0000108  | 0.0001065 | -0.0001910 |
|      | dz | -0.0002020 | -0.0000137 | -0.0001886 | 0.0000169  | 0.0000749  | 0.0000412  | 0.0000816 | 0.0001113  |
| 19H  | dx | -0.0005646 | 0.0005769  | -0.0003808 | -0.0001156 | -0.0002656 | -0.0000812 | 0.0006647 | -0.0003515 |
|      | dy | 0.0000390  | -0.0001768 | -0.0006595 | 0.0000891  | 0.0001189  | 0.0000493  | 0.0006664 | -0.0001259 |
|      | dz | -0.0002589 | 0.0000935  | -0.0001424 | 0.0000378  | 0.0001703  | 0.0000818  | 0.0002058 | 0.0002993  |

Table S10: Harmonic force field data [Cartesian force constant matrix] in  $E_h/a_0^2$  for the equilibrium structure of  $\text{Cp}^{187}\text{Re}(\text{CH}_3)(\text{CO})(\text{NO})$  at level of ZORA-B3LYP/x2c-TZVPPall-2c. (continued).

| Atom |               | 9C         |            | 10H        |            | 11Re       |            | 12C        |            |
|------|---------------|------------|------------|------------|------------|------------|------------|------------|------------|
|      | dx            | dy         | dz         | dx         | dy         | dz         | dx         | dy         | dz         |
| 9C   | dx 0.6113024  |            |            |            |            |            |            |            |            |
|      | dy 0.0288237  | 0.1475849  |            |            |            |            |            |            |            |
|      | dz 0.1346381  | 0.0325689  | 0.7179070  |            |            |            |            |            |            |
| 10H  | dx -0.1571237 | -0.0068240 | -0.1418166 | 0.1568464  |            |            |            |            |            |
|      | dy -0.0041405 | -0.0294955 | -0.0046624 | 0.0054421  | 0.0279731  |            |            |            |            |
|      | dz -0.1414185 | -0.0095473 | -0.2549921 | 0.1520665  | 0.0075350  | 0.2621336  |            |            |            |
| 11Re | dx -0.0123410 | -0.0087210 | -0.0208772 | -0.0003841 | -0.0060542 | -0.0004044 | 0.3920953  |            |            |
|      | dy -0.0064827 | -0.0480997 | -0.0247749 | 0.0024442  | -0.0002597 | 0.0011265  | -0.0401428 | 0.5054873  |            |
|      | dz -0.0114379 | -0.0148182 | -0.0298589 | 0.0002614  | -0.0074543 | -0.0008059 | -0.0100623 | -0.0491426 | 0.4652289  |
| 12C  | dx -0.0005895 | 0.0040690  | 0.0029893  | 0.0001143  | 0.0003752  | -0.0001006 | -0.1040852 | 0.0081069  | 0.0204307  |
|      | dy -0.0031382 | -0.0059529 | -0.0023520 | -0.0004263 | -0.0010001 | 0.0001213  | 0.0259503  | -0.0715886 | -0.0284508 |
|      | dz 0.0021891  | -0.0105187 | -0.0015186 | -0.0004569 | 0.0001699  | -0.0001503 | 0.0248373  | -0.0030307 | -0.0788572 |
| 13N  | dx 0.0069091  | 0.0022753  | 0.0028821  | 0.0002983  | 0.0005601  | -0.0002606 | -0.1244318 | 0.0164907  | -0.0232985 |
|      | dy 0.0022038  | -0.0067223 | 0.0074256  | -0.0000763 | 0.0034726  | 0.0002031  | 0.0363709  | -0.1813603 | 0.0739160  |
|      | dz -0.0058079 | 0.0054755  | 0.0068951  | 0.0002268  | -0.0014921 | 0.0005991  | -0.0260382 | 0.0480841  | -0.2029582 |
| 14O  | dx -0.0002246 | -0.0003886 | -0.0004206 | -0.0001039 | -0.0001226 | -0.0001191 | 0.0099256  | 0.0288903  | 0.0342215  |
|      | dy 0.0020537  | 0.0017721  | 0.0003358  | 0.0001029  | 0.0002965  | -0.0000438 | 0.0253784  | -0.0073894 | -0.0367440 |
|      | dz 0.0007332  | 0.0026985  | 0.0001226  | -0.0000704 | -0.0000111 | -0.0001627 | 0.0286685  | -0.0357930 | -0.0258892 |
| 15O  | dx -0.0021737 | -0.0005200 | -0.0009276 | -0.0000727 | -0.0000197 | 0.0001221  | 0.0391615  | 0.0128027  | -0.0114789 |
|      | dy -0.0031564 | 0.0017780  | -0.0033502 | -0.0002018 | -0.0022489 | -0.0001460 | 0.0078285  | -0.0024403 | 0.0604808  |
|      | dz 0.0044983  | -0.0025101 | -0.0017092 | 0.0006808  | 0.0016181  | 0.0004297  | -0.0081277 | 0.0554789  | -0.0167625 |
| 16C  | dx -0.0016945 | -0.0050101 | -0.0008186 | 0.0007418  | 0.0006400  | 0.0008825  | -0.0709402 | -0.0124048 | -0.0071921 |
|      | dy -0.0011736 | 0.0034467  | -0.0001793 | 0.0005338  | 0.0000164  | 0.0004386  | -0.0284197 | -0.0495079 | -0.0117576 |
|      | dz -0.0000796 | -0.0008877 | 0.0015820  | -0.0000575 | 0.0005810  | 0.0000797  | -0.0081558 | 0.0002128  | -0.0471281 |
| 17H  | dx -0.0001453 | -0.0002077 | 0.0000974  | 0.0000700  | -0.0000022 | -0.0000631 | -0.0170468 | -0.0006805 | 0.0062731  |
|      | dy 0.0001325  | -0.0001862 | -0.0008856 | 0.0000127  | -0.0001571 | -0.0000783 | -0.0079170 | 0.0014734  | 0.0070613  |
|      | dz -0.0006881 | -0.0005594 | 0.0000438  | -0.0000148 | -0.0000161 | -0.0000072 | -0.0075861 | 0.0031770  | 0.0058016  |
| 18H  | dx 0.0004976  | 0.0008514  | 0.0004571  | 0.0000031  | 0.0000188  | -0.0000030 | -0.0075072 | -0.0182244 | -0.0026495 |
|      | dy 0.0000429  | -0.0001147 | 0.0000295  | -0.0000288 | 0.0000037  | 0.0000245  | -0.0029161 | -0.0044274 | -0.0003050 |
|      | dz 0.0002443  | -0.0000652 | 0.0001439  | -0.0000426 | -0.0000009 | -0.0000017 | -0.0034308 | -0.0060766 | -0.0018029 |
| 19H  | dx 0.0001751  | -0.0014538 | 0.0004163  | 0.0000004  | 0.0001132  | 0.0000812  | -0.0083747 | 0.0042863  | -0.0158660 |
|      | dy -0.0005532 | -0.0014738 | 0.0002870  | -0.0000296 | 0.0002454  | -0.0000041 | -0.0037563 | 0.0007944  | -0.0078396 |
|      | dz 0.0003346  | 0.0003276  | 0.0000853  | 0.0000362  | 0.0000061  | -0.0000042 | -0.0028571 | -0.0018154 | -0.0022070 |

Table S10: Harmonic force field data [Cartesian force constant matrix] in  $E_h/a_0^2$  for the equilibrium structure of  $\text{Cp}^{187}\text{Re}(\text{CH}_3)(\text{CO})(\text{NO})$  at level of ZORA-B3LYP/x2c-TZVPPall-2c. (continued).

| Atom |               | 13N        |            | 14O        |            | 15O        |            | 16C        |            |
|------|---------------|------------|------------|------------|------------|------------|------------|------------|------------|
|      | dx            | dy         | dz         | dx         | dy         | dz         | dx         | dy         | dz         |
| 13N  | dx 0.1914135  |            |            |            |            |            |            |            |            |
|      | dy -0.1214426 | 0.5753950  |            |            |            |            |            |            |            |
|      | dz 0.1318173  | -0.4488949 | 0.6942696  |            |            |            |            |            |            |
| 14O  | dx -0.0047573 | 0.0082861  | -0.0093024 | 0.3141046  |            |            |            |            |            |
|      | dy -0.0004372 | -0.0085702 | 0.0073687  | -0.2931274 | 0.3243217  |            |            |            |            |
|      | dz -0.0018253 | -0.0107431 | 0.0191730  | -0.3596939 | 0.3679768  | 0.4748163  |            |            |            |
| 15O  | dx -0.0978589 | 0.0916731  | -0.1029487 | 0.0016499  | -0.0001372 | -0.0002558 | 0.0657370  |            |            |
|      | dy 0.0900867  | -0.3775151 | 0.3460086  | -0.0060663 | 0.0059484  | 0.0080094  | -0.1000682 | 0.3784649  |            |
|      | dz -0.1011245 | 0.3413007  | -0.4737827 | 0.0054533  | -0.0054838 | -0.0080609 | 0.1122635  | -0.3879890 | 0.4814644  |
| 16C  | dx -0.0024004 | 0.0001101  | -0.0052042 | 0.0043242  | 0.0000153  | -0.0009346 | 0.0004157  | -0.0015901 | 0.0030479  |
|      | dy 0.0052541  | 0.0034806  | 0.0048946  | -0.0023589 | 0.0001326  | 0.0012734  | -0.0024245 | 0.0029358  | -0.0054771 |
|      | dz -0.0174746 | -0.0059536 | -0.0037142 | -0.0044778 | 0.0001038  | 0.0004698  | 0.0050455  | -0.0017838 | 0.0043342  |
| 17H  | dx 0.0030025  | -0.0017665 | 0.0031715  | -0.0006347 | 0.0010736  | 0.0012397  | -0.0013407 | 0.0025433  | -0.0033958 |
|      | dy 0.0018846  | 0.0008887  | -0.0000382 | -0.0014535 | 0.0013974  | 0.0024339  | -0.0009452 | 0.0002890  | 0.0015130  |
|      | dz 0.0013045  | -0.0006451 | 0.0013136  | 0.0012600  | -0.0007281 | -0.0015476 | -0.0003148 | 0.0010528  | 0.0008722  |
| 18H  | dx 0.0024200  | -0.0020362 | 0.0039887  | -0.0015257 | 0.0012451  | 0.0015065  | -0.0016400 | 0.0032133  | -0.0044713 |
|      | dy 0.0019133  | 0.0000872  | 0.0023919  | -0.0014066 | 0.0008307  | 0.0013171  | -0.0008906 | 0.0008732  | -0.0017604 |
|      | dz 0.0003337  | -0.0014100 | 0.0014341  | -0.0005983 | -0.0000974 | 0.0000393  | -0.0003124 | 0.0016881  | -0.0015699 |
| 19H  | dx -0.0018533 | -0.0008180 | -0.0002814 | 0.0003755  | -0.0000901 | -0.0003508 | 0.0008426  | -0.0006031 | 0.0014480  |
|      | dy -0.0000514 | -0.0005730 | 0.0005892  | -0.0011100 | 0.0009981  | 0.0002583  | -0.0000571 | 0.0006075  | -0.0005857 |
|      | dz 0.0010359  | 0.0003390  | 0.0004827  | -0.0005880 | 0.0006868  | 0.0007373  | -0.0003318 | 0.0000767  | -0.0002293 |

**Table S10:** Harmonic force field data [Cartesian force constant matrix] in  $E_h/a_0^2$  for the equilibrium structure of  $\text{Cp}^{187}\text{Re}(\text{CH}_3)(\text{CO})(\text{NO})$  at level of ZORA-B3LYP/x2c-TZVPPall-2c. (continued).

| Atom |    | dx         | 17H<br>dy  | dz         | dx         | 18H<br>dy  | dz         | dx         | 19H<br>dy  | dz        |
|------|----|------------|------------|------------|------------|------------|------------|------------|------------|-----------|
| 17H  | dx | 0.1951272  |            |            |            |            |            |            |            |           |
|      | dy | -0.0576594 | 0.0662492  |            |            |            |            |            |            |           |
|      | dz | -0.1327165 | 0.0458551  | 0.1563857  |            |            |            |            |            |           |
| 18H  | dx | -0.0032581 | 0.0239261  | -0.0009991 | 0.0452014  |            |            |            |            |           |
|      | dy | -0.0001553 | -0.0066455 | 0.0007395  | -0.0326114 | 0.3363988  |            |            |            |           |
|      | dz | 0.0019825  | -0.0213503 | 0.0001871  | -0.0014292 | -0.0049193 | 0.0447546  |            |            |           |
| 19H  | dx | 0.0063067  | -0.0072881 | 0.0223608  | -0.0022944 | 0.0004124  | -0.0032489 | 0.0565615  |            |           |
|      | dy | -0.0025560 | 0.0014670  | -0.0085947 | 0.0080787  | -0.0087251 | 0.0314342  | -0.0227117 | 0.0690408  |           |
|      | dz | -0.0049435 | 0.0052611  | -0.0180741 | -0.0008181 | -0.0002429 | -0.0003589 | 0.0615513  | -0.0777560 | 0.2940333 |

Table S11: Harmonic force field data [Cartesian force constant matrix] in  $E_h/a_0^2$  for the equilibrium structure of  $\text{Cp}^{185}\text{Re}(\text{CH}_3)(\text{CO})(\text{NO})$  at level of ZORA-B3LYP/x2c-TZVPPall-2c.

| Atom |               | 1C         |            | 2H         |            | 3C         |            | 4H         |            |
|------|---------------|------------|------------|------------|------------|------------|------------|------------|------------|
|      | dx            | dy         | dz         | dx         | dy         | dz         | dx         | dy         | dz         |
| 1C   | dx 0.5240942  |            |            |            |            |            |            |            |            |
|      | dy 0.0140677  | 0.1413145  |            |            |            |            |            |            |            |
|      | dz -0.0152326 | -0.0299045 | 0.8132788  |            |            |            |            |            |            |
| 2H   | dx -0.0559330 | -0.0017652 | -0.0016261 | 0.0487697  |            |            |            |            |            |
|      | dy -0.0022066 | -0.0254568 | -0.0009540 | 0.0008084  | 0.0249750  |            |            |            |            |
|      | dz -0.0011326 | 0.0031688  | -0.3575061 | 0.0011062  | -0.0002107 | 0.3718430  |            |            |            |
| 3C   | dx -0.2388476 | -0.0111500 | 0.1058906  | 0.0077773  | -0.0001880 | -0.0033305 | 0.7963487  |            |            |
|      | dy 0.0047024  | -0.0411010 | 0.0025993  | -0.0003432 | -0.0025577 | -0.0001491 | 0.0135028  | 0.1471507  |            |
|      | dz 0.0900739  | 0.0186896  | -0.1717113 | 0.0236790  | -0.0035702 | -0.0075475 | 0.0860847  | 0.0056020  | 0.5695919  |
| 4H   | dx -0.0118162 | -0.0008783 | -0.0097821 | 0.0004257  | 0.0000835  | 0.0003833  | -0.3254216 | -0.0184773 | -0.0890259 |
|      | dy -0.0011250 | -0.0013484 | -0.0024696 | 0.0003178  | -0.0018354 | -0.0000894 | -0.0240123 | -0.0320777 | -0.0080192 |
|      | dz 0.0174901  | 0.0014918  | 0.0122841  | -0.0009233 | 0.0002485  | 0.0002348  | -0.0887994 | -0.0061535 | -0.0873482 |
| 5C   | dx 0.0083380  | -0.0113044 | 0.0148427  | -0.0054877 | 0.0002528  | 0.0016345  | -0.1211591 | 0.0080555  | -0.0525319 |
|      | dy -0.0178596 | 0.0065996  | 0.0060720  | -0.0002277 | 0.0025007  | -0.0001040 | 0.0014544  | -0.0397634 | -0.0187302 |
|      | dz 0.0315879  | -0.0148672 | -0.0538172 | 0.0028006  | 0.0005321  | -0.0005347 | -0.0697355 | 0.0025653  | -0.2900817 |
| 6H   | dx -0.0018663 | -0.0001382 | -0.0036925 | 0.0010575  | 0.0002194  | -0.0003807 | 0.0122802  | 0.0000297  | -0.0089935 |
|      | dy 0.0003579  | 0.0029258  | -0.0004360 | 0.0001907  | 0.0014390  | 0.0000931  | -0.0023216 | -0.0027480 | 0.0022613  |
|      | dz -0.0026833 | 0.0001422  | -0.0044755 | 0.0012789  | 0.0000893  | -0.0002354 | 0.0181010  | 0.0001179  | -0.0115065 |
| 7C   | dx -0.2132306 | -0.0010671 | -0.0888515 | 0.0078142  | 0.0015047  | 0.0031601  | -0.0608898 | -0.0106751 | 0.0081891  |
|      | dy -0.0257528 | -0.0366301 | -0.0058656 | 0.0009722  | -0.0027409 | 0.0001079  | 0.0072139  | 0.0041560  | -0.0120578 |
|      | dz -0.0794552 | 0.0106066  | -0.1607393 | -0.0224469 | -0.0036691 | -0.0063355 | -0.0084397 | -0.0111350 | 0.0158267  |
| 8H   | dx -0.0107028 | -0.0009327 | 0.0092980  | 0.0002625  | 0.0002912  | -0.0003940 | -0.0023147 | -0.0005695 | -0.0027557 |
|      | dy 0.0034039  | -0.0024030 | -0.0016189 | -0.0000781 | -0.0011512 | -0.0000927 | -0.0000895 | 0.0027071  | 0.0002116  |
|      | dz -0.0161399 | -0.0021937 | 0.0125352  | 0.0005343  | 0.0002198  | 0.0001797  | -0.0038723 | -0.0002357 | -0.0043106 |
| 9C   | dx 0.0055360  | 0.0099597  | -0.0129273 | -0.0057146 | -0.0005125 | -0.0018249 | -0.0334617 | -0.0161327 | -0.0495768 |
|      | dy 0.0139895  | 0.0036113  | 0.0037813  | -0.0006399 | 0.0032526  | -0.0000908 | -0.0008342 | 0.0073848  | 0.0139971  |
|      | dz -0.0275183 | -0.0166615 | -0.0518681 | -0.0028124 | -0.0002944 | -0.0005509 | -0.0290530 | 0.0023414  | -0.0095059 |
| 10H  | dx -0.0017646 | 0.0001333  | 0.0037255  | 0.0010045  | -0.0002622 | 0.0003474  | -0.0066490 | -0.0007190 | 0.0011445  |
|      | dy -0.0006569 | 0.0030595  | 0.0004857  | -0.0001793 | 0.0011818  | 0.0001892  | 0.0000661  | 0.0034360  | -0.0005656 |
|      | dz 0.0024527  | 0.0000696  | -0.0044548 | -0.0011681 | -0.0000819 | -0.0001941 | 0.0023345  | 0.0003818  | -0.0002452 |
| 11Re | dx -0.0090026 | 0.0012568  | -0.0020688 | -0.0004093 | -0.0000555 | 0.0003201  | -0.0278849 | 0.0143236  | -0.0053833 |
|      | dy 0.0090890  | -0.0328007 | 0.0183289  | 0.0009913  | 0.0012857  | -0.0030806 | 0.0151928  | -0.0322500 | -0.0009742 |
|      | dz 0.0030142  | 0.0103382  | -0.0399863 | -0.0001591 | 0.0098887  | 0.0005096  | -0.0100083 | -0.0014843 | 0.0010130  |
| 12C  | dx 0.0046791  | 0.0044029  | 0.0065233  | 0.0005577  | -0.0012418 | -0.0000875 | 0.0003116  | 0.0040764  | -0.0024638 |
|      | dy 0.0007374  | -0.0027266 | 0.0018272  | -0.0003628 | 0.0005024  | -0.0004584 | 0.0043464  | -0.0005183 | -0.0002824 |
|      | dz -0.0075573 | -0.0005253 | 0.0031155  | -0.0007763 | 0.0005821  | 0.0000365  | 0.0024940  | -0.0006766 | -0.0045378 |
| 13N  | dx 0.0043909  | -0.0033321 | -0.0027446 | 0.0001419  | 0.0005583  | -0.0000766 | -0.0026891 | 0.0070948  | 0.0039255  |
|      | dy 0.0025933  | -0.0147535 | 0.0119743  | -0.0000035 | -0.0022687 | 0.0003368  | 0.0035781  | -0.0077098 | 0.0080704  |
|      | dz -0.0025048 | 0.0217387  | 0.0059781  | 0.0001232  | -0.0025560 | -0.0002731 | 0.0007871  | 0.0086039  | -0.0067808 |
| 14O  | dx -0.0015648 | -0.0020651 | -0.0027233 | -0.0003280 | 0.0007839  | 0.0002237  | 0.0002688  | -0.0003271 | 0.0020568  |
|      | dy -0.0003118 | 0.0014571  | 0.0008585  | 0.0001143  | -0.0006217 | 0.0000999  | -0.0010554 | -0.0007978 | -0.0002965 |
|      | dz 0.0025211  | 0.0006591  | -0.0002862 | 0.0003501  | -0.0008088 | 0.0003969  | -0.0010620 | -0.0012671 | 0.0006790  |
| 15O  | dx -0.0014851 | 0.0027519  | 0.0003878  | -0.0000212 | 0.0000483  | -0.0001000 | 0.0023871  | -0.0035042 | -0.0016226 |
|      | dy -0.0002264 | 0.0000619  | -0.0045085 | -0.0000530 | 0.0007759  | 0.0001451  | -0.0025222 | 0.0005059  | -0.0017335 |
|      | dz -0.0002775 | -0.0023854 | -0.0030060 | 0.0000080  | 0.0013347  | -0.0006639 | 0.0011883  | 0.0005224  | 0.0014065  |
| 16C  | dx -0.0019041 | 0.0003539  | -0.0004253 | 0.0003344  | 0.0000094  | 0.0001306  | 0.0000484  | -0.0025272 | -0.0047390 |
|      | dy -0.0001749 | -0.0012361 | 0.0002956  | 0.0002700  | 0.0004612  | -0.0005777 | -0.0020495 | -0.0060245 | -0.0000254 |
|      | dz 0.0070831  | -0.0008780 | 0.0001650  | 0.0001881  | -0.0001437 | 0.0000014  | -0.0044273 | -0.0026147 | 0.0070185  |
| 17H  | dx -0.0004589 | 0.0001728  | 0.0002617  | -0.0003162 | -0.0000719 | -0.0001444 | 0.0006387  | 0.0007999  | -0.0011514 |
|      | dy -0.0018869 | -0.0001553 | 0.0000379  | 0.0000181  | -0.0000332 | 0.0006258  | 0.0000330  | 0.0003907  | -0.0000424 |
|      | dz -0.0003490 | 0.0000005  | -0.0011050 | -0.0000767 | -0.0002386 | 0.0011377  | 0.0005345  | -0.0008272 | -0.0012318 |
| 18H  | dx 0.0000279  | -0.0001509 | -0.0008591 | 0.0000612  | 0.0001953  | -0.0000274 | -0.0002633 | 0.0013159  | 0.0015706  |
|      | dy -0.0001112 | -0.0002835 | -0.0003142 | -0.0000044 | 0.0001456  | -0.0000269 | 0.0002638  | -0.0003941 | 0.0001674  |
|      | dz -0.0009268 | 0.0001689  | 0.0012367  | -0.0000433 | -0.0000669 | -0.0005425 | 0.00011629 | 0.0003896  | -0.0003773 |
| 19H  | dx 0.0015105  | -0.0003151 | 0.0000038  | 0.0000033  | -0.0002168 | 0.0001928  | -0.0004799 | -0.0006255 | 0.0015199  |
|      | dy 0.0013712  | -0.0001345 | -0.0001892 | -0.0000256 | 0.0001457  | 0.0001137  | -0.0014286 | 0.0002110  | -0.0001604 |
|      | dz -0.0004456 | 0.0003415  | 0.0003626  | -0.0000362 | -0.0003009 | 0.0000440  | 0.0001502  | 0.0014197  | -0.0003509 |

Table S11: Harmonic force field data [Cartesian force constant matrix] in  $E_h/a_0^2$  for the equilibrium structure of  $\text{Cp}^{185}\text{Re}(\text{CH}_3)(\text{CO})(\text{NO})$  at level of ZORA-B3LYP/x2c-TZVPPall-2c. (continued).

| Atom |               | 5C         |            | 6H         |            | 7C         |            | 8H         |            |
|------|---------------|------------|------------|------------|------------|------------|------------|------------|------------|
|      | dx            | dy         | dz         | dx         | dy         | dz         | dx         | dy         | dz         |
| 5C   | dx 0.6180060  |            |            |            |            |            |            |            |            |
|      | dy -0.0038378 | 0.1383884  |            |            |            |            |            |            |            |
|      | dz -0.1343707 | 0.0250314  | 0.7218203  |            |            |            |            |            |            |
| 6H   | dx -0.1640010 | -0.0023222 | 0.1445045  | 0.1634469  |            |            |            |            |            |
|      | dy -0.0038079 | -0.0250111 | 0.0020702  | 0.0023852  | 0.0247565  |            |            |            |            |
|      | dz 0.1440416  | -0.0008629 | -0.2492835 | -0.1547944 | -0.0019025 | 0.2561933  |            |            |            |
| 7C   | dx -0.0306614 | -0.0019045 | 0.0252238  | -0.0056400 | -0.0009089 | -0.0023011 | 0.7710617  |            |            |
|      | dy 0.0139299  | 0.0039690  | 0.0062567  | -0.0008056 | 0.0036117  | -0.0004262 | 0.0739303  | 0.1445055  |            |
|      | dz 0.0384429  | 0.0187923  | -0.0102985 | -0.0015403 | 0.0001941  | -0.0003631 | -0.0975604 | -0.0201516 | 0.5461277  |
| 8H   | dx 0.0002127  | -0.0001837 | -0.0003333 | 0.0002505  | -0.0002695 | -0.0000084 | -0.3285428 | -0.0264562 | 0.0887851  |
|      | dy 0.0005249  | 0.0026482  | -0.0010055 | 0.0000634  | 0.0010284  | -0.0001971 | -0.0252653 | -0.0253508 | 0.0076669  |
|      | dz 0.0006594  | 0.0001148  | -0.0057676 | 0.0013918  | 0.0001151  | 0.0007240  | 0.0882710  | 0.0077559  | -0.0850292 |
| 9C   | dx -0.2877709 | 0.0031330  | 0.0074040  | -0.0057690 | -0.0006561 | -0.0029757 | -0.1177132 | -0.0151681 | 0.0537480  |
|      | dy -0.0248290 | -0.0360774 | -0.0070257 | 0.0005097  | -0.0026597 | 0.0000391  | -0.0008071 | -0.0399687 | -0.0149778 |
|      | dz -0.0070394 | -0.0072011 | -0.1000190 | 0.0220220  | 0.0038205  | 0.0074420  | 0.0681507  | 0.0135425  | -0.2794216 |
| 10H  | dx -0.0055950 | -0.0010866 | -0.0231673 | 0.0000337  | 0.0002512  | 0.0003298  | 0.0121695  | 0.0004197  | 0.0085908  |
|      | dy 0.0005413  | -0.0031921 | 0.0025149  | -0.0001984 | -0.0011452 | -0.0000244 | 0.0034818  | -0.0018446 | 0.0015304  |
|      | dz 0.0025740  | 0.0005943  | 0.0075655  | -0.0003788 | -0.0000023 | 0.0002329  | -0.0170881 | -0.0003771 | -0.0107142 |
| 11Re | dx -0.0206619 | 0.0128612  | 0.0183211  | -0.0006627 | 0.0068684  | 0.0001129  | -0.0391322 | -0.0266931 | 0.0219995  |
|      | dy 0.0166684  | -0.0359562 | -0.0155277 | 0.0000917  | -0.0003910 | 0.0034545  | -0.0387205 | -0.0423674 | 0.0106101  |
|      | dz 0.0192634  | -0.0097188 | -0.0227618 | 0.0016956  | -0.0075731 | 0.0002683  | 0.0078274  | 0.0109569  | -0.0032912 |
| 12C  | dx 0.0058079  | 0.0058831  | 0.0005859  | 0.0001414  | -0.0012817 | 0.0002715  | -0.0006187 | 0.0024265  | -0.0069586 |
|      | dy 0.0046781  | -0.0110807 | -0.0043871 | -0.0002454 | -0.0013394 | -0.0003562 | 0.0067858  | -0.0080701 | -0.0059880 |
|      | dz -0.0009729 | -0.0152051 | 0.0006180  | -0.0003563 | 0.0011882  | -0.0004534 | 0.0117709  | -0.0069351 | 0.0012094  |
| 13N  | dx 0.0039973  | 0.0033746  | -0.0094989 | -0.0000787 | -0.0017451 | 0.0002648  | 0.0048216  | 0.0015629  | 0.0032101  |
|      | dy 0.0008468  | -0.0016327 | 0.0049717  | -0.0004272 | 0.0018908  | -0.0002741 | -0.0024657 | -0.0038225 | 0.0034681  |
|      | dz 0.0037763  | 0.0035908  | 0.0052504  | 0.0001864  | -0.0008861 | 0.0003982  | -0.0028845 | 0.0063027  | -0.0049491 |
| 14O  | dx -0.0027180 | 0.0016573  | -0.0002308 | -0.0001545 | 0.0006307  | -0.0000508 | 0.0014355  | -0.0021765 | 0.0019424  |
|      | dy -0.0010718 | -0.0002975 | 0.0015162  | 0.0000304  | 0.0003963  | 0.0002518  | -0.0042377 | 0.0033988  | 0.0022314  |
|      | dz 0.0012162  | -0.0004748 | -0.0002843 | 0.0002172  | -0.0003708 | 0.0000637  | -0.0057368 | 0.0039203  | 0.0000087  |
| 15O  | dx -0.0005679 | -0.0010850 | 0.0033054  | 0.0000026  | 0.0006781  | 0.0000070  | -0.0005868 | 0.0012078  | -0.0013392 |
|      | dy 0.0008768  | 0.0002518  | -0.0032527 | 0.0002587  | -0.0013776 | -0.0000125 | 0.0006992  | -0.0011875 | -0.0005721 |
|      | dz -0.0024128 | -0.0011730 | -0.0012322 | -0.0006335 | 0.0010027  | 0.0004651  | 0.0004390  | 0.0007053  | 0.0014374  |
| 16C  | dx 0.0022096  | -0.0011770 | 0.0037184  | 0.0010103  | 0.0002422  | -0.0008079 | 0.0014061  | -0.0033958 | -0.0013547 |
|      | dy 0.0004469  | 0.0000290  | -0.0002588 | 0.0002603  | 0.0001060  | -0.0000904 | 0.0001954  | 0.0005287  | 0.0010510  |
|      | dz -0.0030348 | 0.0009170  | -0.0019282 | -0.0001720 | 0.0002367  | -0.0000493 | -0.0023704 | -0.0026900 | -0.0008797 |
| 17H  | dx 0.0006383  | 0.0000752  | 0.0002613  | 0.0000185  | -0.0004795 | -0.0001481 | 0.0005116  | -0.0005011 | -0.0000638 |
|      | dy 0.0003976  | -0.0001908 | -0.0003321 | 0.0000444  | 0.0001930  | -0.0002121 | 0.0001576  | -0.0010289 | 0.0007942  |
|      | dz 0.0007517  | -0.0002010 | 0.0009199  | 0.0001383  | -0.0000201 | -0.0000683 | 0.0002444  | -0.0009694 | -0.0001546 |
| 18H  | dx -0.0005911 | 0.0003832  | -0.0010009 | -0.0000730 | -0.0000292 | -0.0000386 | 0.0005281  | -0.0001183 | 0.0003885  |
|      | dy -0.0002727 | 0.0000468  | 0.0003355  | -0.0000200 | 0.0000136  | 0.0000108  | 0.0001064  | -0.0001912 | 0.0000186  |
|      | dz -0.0002020 | -0.0000138 | -0.0001886 | 0.0000169  | 0.0000749  | 0.0000412  | -0.0000816 | 0.0001113  | 0.0001903  |
| 19H  | dx -0.0005646 | 0.0005769  | -0.0003809 | -0.0001156 | -0.0002656 | -0.0000812 | -0.0006647 | -0.0003515 | -0.0005562 |
|      | dy 0.0000389  | -0.0001768 | -0.0006594 | 0.0000891  | 0.0001189  | 0.0000493  | -0.0006665 | -0.0001260 | -0.0003175 |
|      | dz -0.0002587 | 0.0000935  | -0.0001425 | 0.0000378  | 0.0001704  | 0.0000818  | -0.0002056 | 0.0002993  | 0.0006944  |

Table S11: Harmonic force field data [Cartesian force constant matrix] in  $E_h/a_0^2$  for the equilibrium structure of  $\text{Cp}^{185}\text{Re}(\text{CH}_3)(\text{CO})(\text{NO})$  at level of ZORA-B3LYP/x2c-TZVPPall-2c. (continued).

| Atom |               | 9C         |            | 10H        |            | 11Re       |            | 12C        |            |
|------|---------------|------------|------------|------------|------------|------------|------------|------------|------------|
|      | dx            | dy         | dz         | dx         | dy         | dz         | dx         | dy         | dz         |
| 9C   | dx 0.6113026  |            |            |            |            |            |            |            |            |
|      | dy 0.0288240  | 0.1475850  |            |            |            |            |            |            |            |
|      | dz 0.1346385  | 0.0325693  | 0.7179072  |            |            |            |            |            |            |
| 10H  | dx -0.1571239 | -0.0068241 | -0.1418167 | 0.1568464  |            |            |            |            |            |
|      | dy -0.0041406 | -0.0294955 | -0.0046624 | 0.0054421  | 0.0279731  |            |            |            |            |
|      | dz -0.1414187 | -0.0095474 | -0.2549923 | 0.1520665  | 0.0075350  | 0.2621336  |            |            |            |
| 11Re | dx -0.0123421 | -0.0087215 | -0.0208804 | -0.0003825 | -0.0060537 | -0.0004020 | 0.3920964  |            |            |
|      | dy -0.0064853 | -0.0481001 | -0.0247791 | 0.0024451  | -0.0002598 | 0.0011279  | -0.0401423 | 0.5054839  |            |
|      | dz -0.0114393 | -0.0148186 | -0.0298604 | 0.0002627  | -0.0074544 | -0.0008039 | -0.0100633 | -0.0491410 | 0.4652312  |
| 12C  | dx -0.0005894 | 0.0040686  | 0.0029897  | 0.0001142  | 0.0003751  | -0.0001008 | -0.1040855 | 0.0081124  | 0.0204292  |
|      | dy -0.0031378 | -0.0059523 | -0.0023520 | -0.0004263 | -0.0010001 | 0.0001211  | 0.0259483  | -0.0715947 | -0.0284477 |
|      | dz 0.0021894  | -0.0105181 | -0.0015187 | -0.0004570 | 0.0001700  | -0.0001505 | 0.0248364  | -0.0030377 | -0.0788539 |
| 13N  | dx 0.0069092  | 0.0022752  | 0.0028825  | 0.0002981  | 0.0005601  | -0.0002608 | -0.1244314 | 0.0164924  | -0.0232991 |
|      | dy 0.0022039  | -0.0067218 | 0.0074261  | -0.0000764 | 0.0034727  | 0.0002029  | 0.0363734  | -0.1813658 | 0.0739149  |
|      | dz -0.0058075 | 0.0054749  | 0.0068951  | 0.0002267  | -0.0014922 | 0.0005989  | -0.0260415 | 0.0480917  | -0.2029565 |
| 14O  | dx -0.0002245 | -0.0003881 | -0.0004205 | -0.0001041 | -0.0001226 | -0.0001194 | 0.0099249  | 0.0288842  | 0.0342238  |
|      | dy 0.0020537  | 0.0017716  | 0.0003366  | 0.0001028  | 0.0002965  | -0.0000439 | 0.0253808  | -0.0073827 | -0.0367479 |
|      | dz 0.0007333  | 0.0026979  | 0.0001230  | -0.0000705 | -0.0000112 | -0.0001629 | 0.0286700  | -0.0357853 | -0.0258932 |
| 15O  | dx -0.0021735 | -0.0005198 | -0.0009272 | -0.0000729 | -0.0000198 | 0.0001217  | 0.0391611  | 0.0128005  | -0.0114786 |
|      | dy -0.0031558 | 0.0017773  | -0.0033499 | -0.0002019 | -0.0022489 | -0.0001462 | 0.0078244  | -0.0024315 | 0.0604831  |
|      | dz 0.0044982  | -0.0025091 | -0.0017088 | 0.0006806  | 0.0016182  | 0.0004295  | -0.0081236 | 0.0554687  | -0.0167660 |
| 16C  | dx -0.0016944 | -0.0050100 | -0.0008183 | 0.0007417  | 0.0006400  | 0.0008823  | -0.0709406 | -0.0124048 | -0.0071924 |
|      | dy -0.0011733 | 0.0034469  | -0.0001789 | 0.0005338  | 0.0000164  | 0.0004385  | -0.0284211 | -0.0495094 | -0.0117573 |
|      | dz -0.0000798 | -0.0008878 | 0.0015823  | -0.0000577 | 0.0005810  | 0.0000795  | -0.0081519 | 0.0002144  | -0.0471301 |
| 17H  | dx -0.0001454 | -0.0002077 | 0.0000974  | 0.0000700  | -0.0000022 | -0.0000631 | -0.0170452 | -0.0006799 | 0.0062731  |
|      | dy 0.0001326  | -0.0001861 | -0.0008855 | 0.0000127  | -0.0001571 | -0.0000783 | -0.0079174 | 0.0014729  | 0.0070613  |
|      | dz -0.0006880 | -0.0005593 | 0.0000438  | -0.0000148 | -0.0000161 | -0.0000072 | -0.0075871 | 0.0031762  | 0.0058014  |
| 18H  | dx 0.0004976  | 0.0008514  | 0.0004571  | 0.0000031  | 0.0000188  | -0.0000030 | -0.0075076 | -0.0182243 | -0.0026492 |
|      | dy 0.0000429  | -0.0001149 | 0.0000295  | -0.0000288 | 0.0000037  | 0.0000245  | -0.0029151 | -0.0044250 | -0.0003049 |
|      | dz 0.0002443  | -0.0000653 | 0.0001438  | -0.0000426 | -0.0000009 | -0.0000017 | -0.0034309 | -0.0060765 | -0.0018024 |
| 19H  | dx 0.0001751  | -0.0014538 | 0.0004163  | 0.0000004  | 0.0001132  | 0.0000811  | -0.0083752 | 0.0042863  | -0.0158657 |
|      | dy -0.0005532 | -0.0014738 | 0.0002871  | -0.0000297 | 0.0002454  | -0.0000041 | -0.0037555 | 0.0007946  | -0.0078402 |
|      | dz 0.0003348  | 0.0003277  | 0.0000852  | 0.0000363  | 0.0000061  | -0.0000042 | -0.0028597 | -0.0018161 | -0.0022054 |

Table S11: Harmonic force field data [Cartesian force constant matrix] in  $E_h/a_0^2$  for the equilibrium structure of  $\text{Cp}^{185}\text{Re}(\text{CH}_3)(\text{CO})(\text{NO})$  at level of ZORA-B3LYP/x2c-TZVPPall-2c. (continued).

| Atom |               | 13N        |            | 14O        |            | 15O        |            | 16C        |            |
|------|---------------|------------|------------|------------|------------|------------|------------|------------|------------|
|      | dx            | dy         | dz         | dx         | dy         | dz         | dx         | dy         | dz         |
| 13N  | dx 0.1914134  |            |            |            |            |            |            |            |            |
|      | dy -0.1214431 | 0.5753962  |            |            |            |            |            |            |            |
|      | dz 0.1318177  | -0.4488956 | 0.6942692  |            |            |            |            |            |            |
| 14O  | dx -0.0047573 | 0.0082864  | -0.0093021 | 0.3141048  |            |            |            |            |            |
|      | dy -0.0004377 | -0.0085703 | 0.0073683  | -0.2931270 | 0.3243202  |            |            |            |            |
|      | dz -0.0018253 | -0.0107437 | 0.0191731  | -0.3596943 | 0.3679763  | 0.4748172  |            |            |            |
| 15O  | dx -0.0978590 | 0.0916730  | -0.1029483 | 0.0016500  | -0.0001372 | -0.0002560 | 0.0657371  |            |            |
|      | dy 0.0900869  | -0.3775153 | 0.3460074  | -0.0060650 | 0.0059468  | 0.0080082  | -0.1000674 | 0.3784628  |            |
|      | dz -0.1011249 | 0.3413019  | -0.4737825 | 0.0054524  | -0.0054823 | -0.0080600 | 0.1122630  | -0.3879881 | 0.4814653  |
| 16C  | dx -0.0024004 | 0.0001099  | -0.0052038 | 0.0043243  | 0.0000151  | -0.0009347 | 0.0004158  | -0.0015897 | 0.0030475  |
|      | dy 0.0052541  | 0.0034813  | 0.0048939  | -0.0023582 | 0.0001322  | 0.0012726  | -0.0024241 | 0.0029352  | -0.0054762 |
|      | dz -0.0174749 | -0.0059537 | -0.0037141 | -0.0044785 | 0.0001039  | 0.0004704  | 0.0050450  | -0.0017843 | 0.0043347  |
| 17H  | dx 0.0030023  | -0.0017666 | 0.0031716  | -0.0006349 | 0.0010735  | 0.0012397  | -0.0013409 | 0.0025433  | -0.0033959 |
|      | dy 0.0018846  | 0.0008888  | -0.0000383 | -0.0014534 | 0.0013974  | 0.0024338  | -0.0009452 | 0.0002889  | -0.0015129 |
|      | dz 0.0013046  | -0.0006451 | 0.0013136  | 0.0012601  | -0.0007280 | -0.0015475 | -0.0003147 | 0.0010529  | -0.0008722 |
| 18H  | dx 0.0024200  | -0.0020363 | 0.0039887  | -0.0015257 | 0.0012451  | 0.0015065  | -0.0016400 | 0.0032133  | -0.0044713 |
|      | dy 0.0019131  | 0.0000870  | 0.0023918  | -0.0014067 | 0.0008304  | 0.0013170  | -0.0008907 | 0.0008729  | -0.0017604 |
|      | dz 0.0003337  | -0.0014100 | 0.0014340  | -0.0005983 | -0.0000973 | 0.0000393  | -0.0003123 | 0.0016880  | -0.0015699 |
| 19H  | dx -0.0018532 | -0.0008180 | -0.0002814 | 0.0003756  | -0.0000901 | -0.0003509 | 0.0008426  | -0.0006031 | 0.0014479  |
|      | dy -0.0000515 | -0.0005730 | 0.0005892  | -0.0011100 | 0.0009980  | 0.0002583  | -0.0000572 | 0.0006074  | -0.0005855 |
|      | dz 0.0010362  | 0.0003390  | 0.0004825  | -0.0005877 | 0.0006870  | 0.0007371  | -0.0003315 | 0.0000767  | -0.0002295 |

**Table S11:** Harmonic force field data [Cartesian force constant matrix] in  $E_h/a_0^2$  for the equilibrium structure of  $\text{Cp}^{185}\text{Re}(\text{CH}_3)(\text{CO})(\text{NO})$  at level of ZORA-B3LYP/x2c-TZVPPall-2c. (continued).

| Atom |    | dx         | 17H<br>dy  | dz         | dx         | 18H<br>dy  | dz         | dx         | 19H<br>dy  | dz        |
|------|----|------------|------------|------------|------------|------------|------------|------------|------------|-----------|
| 17H  | dx | 0.1951271  |            |            |            |            |            |            |            |           |
|      | dy | -0.0576594 | 0.0662492  |            |            |            |            |            |            |           |
|      | dz | -0.1327165 | 0.0458551  | 0.1563857  |            |            |            |            |            |           |
| 18H  | dx | -0.0032581 | 0.0239261  | -0.0009991 | 0.0452014  |            |            |            |            |           |
|      | dy | -0.0001553 | -0.0066455 | 0.0007395  | -0.0326114 | 0.3363988  |            |            |            |           |
|      | dz | 0.0019825  | -0.0213503 | 0.0001871  | -0.0014293 | -0.0049193 | 0.0447546  |            |            |           |
| 19H  | dx | 0.0063067  | -0.0072881 | 0.0223608  | -0.0022944 | 0.0004124  | -0.0032489 | 0.0565615  |            |           |
|      | dy | -0.0025560 | 0.0014670  | -0.0085947 | 0.0080787  | -0.0087252 | 0.0314342  | -0.0227117 | 0.0690408  |           |
|      | dz | -0.0049435 | 0.0052611  | -0.0180741 | -0.0008181 | -0.0002429 | -0.0003590 | 0.0615513  | -0.0777560 | 0.2940332 |

## **1.1 Equilibrium structure at level RECP-B3LYP/cc5Z from Ref. 1**

Table S12: Cartesian HF and LDA parity-violating energy gradients in units of  $E_h/a_0$  for the equilibrium structure of  $\text{Cp}^{187}\text{Re}(\text{CH}_3)(\text{CO})(\text{NO})$  optimized at the level RECP-B3LYP/cc-pV5Z,cc-pwCVQZ-PP.

| <b>HF</b>  |                          |                          |                          |
|------------|--------------------------|--------------------------|--------------------------|
| Atom       | $x$                      | $y$                      | $z$                      |
| C          | $1.106 \times 10^{-14}$  | $1.402 \times 10^{-14}$  | $-1.261 \times 10^{-14}$ |
| H          | $-6.533 \times 10^{-16}$ | $1.424 \times 10^{-15}$  | $3.950 \times 10^{-16}$  |
| C          | $6.107 \times 10^{-15}$  | $-2.272 \times 10^{-14}$ | $4.447 \times 10^{-15}$  |
| H          | $-2.407 \times 10^{-16}$ | $-6.234 \times 10^{-16}$ | $1.609 \times 10^{-16}$  |
| C          | $-6.542 \times 10^{-15}$ | $-6.179 \times 10^{-15}$ | $4.283 \times 10^{-15}$  |
| H          | $8.545 \times 10^{-17}$  | $7.134 \times 10^{-16}$  | $-4.412 \times 10^{-16}$ |
| C          | $-1.728 \times 10^{-14}$ | $1.627 \times 10^{-14}$  | $-9.073 \times 10^{-16}$ |
| H          | $-3.578 \times 10^{-17}$ | $-4.642 \times 10^{-15}$ | $4.959 \times 10^{-17}$  |
| C          | $1.755 \times 10^{-15}$  | $-1.280 \times 10^{-17}$ | $-8.212 \times 10^{-15}$ |
| H          | $-6.607 \times 10^{-17}$ | $-1.344 \times 10^{-15}$ | $4.286 \times 10^{-16}$  |
| Re         | $1.328 \times 10^{-13}$  | $6.560 \times 10^{-15}$  | $-2.993 \times 10^{-14}$ |
| C          | $-5.914 \times 10^{-14}$ | $3.603 \times 10^{-14}$  | $2.006 \times 10^{-14}$  |
| N          | $-6.380 \times 10^{-14}$ | $-3.073 \times 10^{-14}$ | $-5.591 \times 10^{-15}$ |
| O          | $8.374 \times 10^{-15}$  | $1.990 \times 10^{-15}$  | $1.068 \times 10^{-14}$  |
| O          | $1.797 \times 10^{-14}$  | $8.942 \times 10^{-15}$  | $1.073 \times 10^{-14}$  |
| C          | $-1.765 \times 10^{-14}$ | $-1.486 \times 10^{-14}$ | $1.268 \times 10^{-14}$  |
| H          | $-6.330 \times 10^{-15}$ | $-4.236 \times 10^{-15}$ | $-2.905 \times 10^{-15}$ |
| H          | $-7.017 \times 10^{-15}$ | $-1.376 \times 10^{-15}$ | $-1.628 \times 10^{-15}$ |
| H          | $5.662 \times 10^{-16}$  | $7.818 \times 10^{-16}$  | $-1.702 \times 10^{-15}$ |
| <b>LDA</b> |                          |                          |                          |
| Atom       | $x$                      | $y$                      | $z$                      |
| C          | $9.951 \times 10^{-15}$  | $1.227 \times 10^{-14}$  | $-6.980 \times 10^{-15}$ |
| H          | $-2.764 \times 10^{-16}$ | $6.232 \times 10^{-16}$  | $2.856 \times 10^{-16}$  |
| C          | $3.738 \times 10^{-15}$  | $-1.205 \times 10^{-14}$ | $5.356 \times 10^{-15}$  |
| H          | $-3.769 \times 10^{-16}$ | $-4.092 \times 10^{-16}$ | $1.166 \times 10^{-16}$  |
| C          | $-6.624 \times 10^{-15}$ | $-6.312 \times 10^{-15}$ | $-1.213 \times 10^{-15}$ |
| H          | $1.584 \times 10^{-16}$  | $1.854 \times 10^{-16}$  | $-1.102 \times 10^{-16}$ |
| C          | $-9.241 \times 10^{-15}$ | $6.506 \times 10^{-15}$  | $-1.828 \times 10^{-15}$ |
| H          | $-2.643 \times 10^{-16}$ | $-1.864 \times 10^{-15}$ | $-1.264 \times 10^{-16}$ |
| C          | $6.921 \times 10^{-15}$  | $-5.498 \times 10^{-17}$ | $-1.803 \times 10^{-15}$ |
| H          | $2.493 \times 10^{-16}$  | $6.831 \times 10^{-16}$  | $2.029 \times 10^{-16}$  |
| Re         | $4.590 \times 10^{-14}$  | $-1.298 \times 10^{-15}$ | $-2.735 \times 10^{-14}$ |
| C          | $-1.376 \times 10^{-14}$ | $2.284 \times 10^{-14}$  | $2.102 \times 10^{-14}$  |
| N          | $-5.390 \times 10^{-14}$ | $-2.014 \times 10^{-14}$ | $1.217 \times 10^{-14}$  |
| O          | $-1.338 \times 10^{-15}$ | $-4.289 \times 10^{-15}$ | $-1.145 \times 10^{-15}$ |
| O          | $2.824 \times 10^{-14}$  | $7.357 \times 10^{-15}$  | $-1.765 \times 10^{-15}$ |
| C          | $-5.247 \times 10^{-15}$ | $-3.110 \times 10^{-15}$ | $4.508 \times 10^{-15}$  |
| H          | $-2.237 \times 10^{-15}$ | $-1.739 \times 10^{-15}$ | $-1.408 \times 10^{-15}$ |
| H          | $-2.257 \times 10^{-15}$ | $-1.425 \times 10^{-17}$ | $2.868 \times 10^{-16}$  |
| H          | $3.617 \times 10^{-16}$  | $8.212 \times 10^{-16}$  | $-2.124 \times 10^{-16}$ |

Table S13: Cartesian HF and LDA parity-violating energy gradients in units of  $E_h/a_0$  for the equilibrium structure of  $\text{Cp}^{185}\text{Re}(\text{CH}_3)(\text{CO})(\text{NO})$  optimized at the level RECP-B3LYP/cc-pV5Z,cc-pwCVQZ-PP.

| <b>HF</b>  |                          |                          |                          |
|------------|--------------------------|--------------------------|--------------------------|
| Atom       | $x$                      | $y$                      | $z$                      |
| C          | $1.087 \times 10^{-14}$  | $1.377 \times 10^{-14}$  | $-1.238 \times 10^{-14}$ |
| H          | $-6.418 \times 10^{-16}$ | $1.399 \times 10^{-15}$  | $3.880 \times 10^{-16}$  |
| C          | $5.999 \times 10^{-15}$  | $-2.232 \times 10^{-14}$ | $4.369 \times 10^{-15}$  |
| H          | $-2.364 \times 10^{-16}$ | $-6.124 \times 10^{-16}$ | $1.580 \times 10^{-16}$  |
| C          | $-6.427 \times 10^{-15}$ | $-6.070 \times 10^{-15}$ | $4.207 \times 10^{-15}$  |
| H          | $8.393 \times 10^{-17}$  | $7.008 \times 10^{-16}$  | $-4.334 \times 10^{-16}$ |
| C          | $-1.697 \times 10^{-14}$ | $1.598 \times 10^{-14}$  | $-8.912 \times 10^{-16}$ |
| H          | $-3.515 \times 10^{-17}$ | $-4.560 \times 10^{-15}$ | $4.872 \times 10^{-17}$  |
| C          | $1.724 \times 10^{-15}$  | $-1.255 \times 10^{-17}$ | $-8.067 \times 10^{-15}$ |
| H          | $-6.490 \times 10^{-17}$ | $-1.320 \times 10^{-15}$ | $4.210 \times 10^{-16}$  |
| Re         | $1.305 \times 10^{-13}$  | $6.444 \times 10^{-15}$  | $-2.940 \times 10^{-14}$ |
| C          | $-5.810 \times 10^{-14}$ | $3.539 \times 10^{-14}$  | $1.971 \times 10^{-14}$  |
| N          | $-6.267 \times 10^{-14}$ | $-3.019 \times 10^{-14}$ | $-5.492 \times 10^{-15}$ |
| O          | $8.226 \times 10^{-15}$  | $1.955 \times 10^{-15}$  | $1.049 \times 10^{-14}$  |
| O          | $1.766 \times 10^{-14}$  | $8.784 \times 10^{-15}$  | $1.054 \times 10^{-14}$  |
| C          | $-1.733 \times 10^{-14}$ | $-1.460 \times 10^{-14}$ | $1.246 \times 10^{-14}$  |
| H          | $-6.218 \times 10^{-15}$ | $-4.162 \times 10^{-15}$ | $-2.853 \times 10^{-15}$ |
| H          | $-6.893 \times 10^{-15}$ | $-1.352 \times 10^{-15}$ | $-1.600 \times 10^{-15}$ |
| H          | $5.562 \times 10^{-16}$  | $7.680 \times 10^{-16}$  | $-1.672 \times 10^{-15}$ |
| <b>LDA</b> |                          |                          |                          |
| Atom       | $x$                      | $y$                      | $z$                      |
| C          | $9.776 \times 10^{-15}$  | $1.205 \times 10^{-14}$  | $-6.857 \times 10^{-15}$ |
| H          | $-2.715 \times 10^{-16}$ | $6.122 \times 10^{-16}$  | $2.806 \times 10^{-16}$  |
| C          | $3.672 \times 10^{-15}$  | $-1.184 \times 10^{-14}$ | $5.261 \times 10^{-15}$  |
| H          | $-3.703 \times 10^{-16}$ | $-4.019 \times 10^{-16}$ | $1.145 \times 10^{-16}$  |
| C          | $-6.507 \times 10^{-15}$ | $-6.201 \times 10^{-15}$ | $-1.192 \times 10^{-15}$ |
| H          | $1.556 \times 10^{-16}$  | $1.821 \times 10^{-16}$  | $-1.083 \times 10^{-16}$ |
| C          | $-9.078 \times 10^{-15}$ | $6.391 \times 10^{-15}$  | $-1.795 \times 10^{-15}$ |
| H          | $-2.596 \times 10^{-16}$ | $-1.831 \times 10^{-15}$ | $-1.242 \times 10^{-16}$ |
| C          | $6.798 \times 10^{-15}$  | $-5.401 \times 10^{-17}$ | $-1.772 \times 10^{-15}$ |
| H          | $2.449 \times 10^{-16}$  | $6.710 \times 10^{-16}$  | $1.993 \times 10^{-16}$  |
| Re         | $4.509 \times 10^{-14}$  | $-1.275 \times 10^{-15}$ | $-2.687 \times 10^{-14}$ |
| C          | $-1.352 \times 10^{-14}$ | $2.243 \times 10^{-14}$  | $2.064 \times 10^{-14}$  |
| N          | $-5.294 \times 10^{-14}$ | $-1.978 \times 10^{-14}$ | $1.196 \times 10^{-14}$  |
| O          | $-1.314 \times 10^{-15}$ | $-4.214 \times 10^{-15}$ | $-1.125 \times 10^{-15}$ |
| O          | $2.774 \times 10^{-14}$  | $7.227 \times 10^{-15}$  | $-1.734 \times 10^{-15}$ |
| C          | $-5.154 \times 10^{-15}$ | $-3.055 \times 10^{-15}$ | $4.428 \times 10^{-15}$  |
| H          | $-2.197 \times 10^{-15}$ | $-1.708 \times 10^{-15}$ | $-1.383 \times 10^{-15}$ |
| H          | $-2.217 \times 10^{-15}$ | $-1.401 \times 10^{-17}$ | $2.817 \times 10^{-16}$  |
| H          | $3.553 \times 10^{-16}$  | $8.067 \times 10^{-16}$  | $-2.087 \times 10^{-16}$ |

Table S14: Parity violating (PV) energy  $E_{PV}$ , relative PV vibrational frequency splittings ( $\Delta\nu/\nu$ ) from 1D and 2D perturbative treatment for fundamental transitions of  $\nu_9$  and  $\nu_{10}$  stretching vibrations and relative PV shifts of rotational constants ( $\Delta X/X$ ) of  $\text{Cp}^{187}\text{Re}(\text{CH}_3)(\text{CO})(\text{NO})$  and  $\text{Cp}^{185}\text{Re}(\text{CH}_3)(\text{CO})(\text{NO})$  optimized at the level RECP-B3LYP/cc-pV5Z,cc-pwCVQZ-PP.

| Method   | $\text{Cp}^{187}\text{Re}(\text{CH}_3)(\text{CO})(\text{NO})$ |                                          | $\text{Cp}^{185}\text{Re}(\text{CH}_3)(\text{CO})(\text{NO})$ |                                          |                             |                             |
|----------|---------------------------------------------------------------|------------------------------------------|---------------------------------------------------------------|------------------------------------------|-----------------------------|-----------------------------|
|          | $E_{\text{PV}} \times 10^9/\text{cm}^{-1} \text{ } hc$        |                                          | $E_{\text{PV}} \times 10^9/\text{cm}^{-1} \text{ } hc$        |                                          |                             |                             |
| HF       | 1.568                                                         |                                          | 1.540                                                         |                                          |                             |                             |
| B3LYP    | 1.531                                                         |                                          | 1.504                                                         |                                          |                             |                             |
| BLYP     | 1.381                                                         |                                          | 1.356                                                         |                                          |                             |                             |
| LDA      | 1.372                                                         |                                          | 1.348                                                         |                                          |                             |                             |
|          | $\Delta\nu_9/\nu_9 \times 10^{14}$                            | $\Delta\nu_{10}/\nu_{10} \times 10^{14}$ | $\Delta\nu_9/\nu_9 \times 10^{14}$                            | $\Delta\nu_{10}/\nu_{10} \times 10^{14}$ |                             |                             |
| HF (1D)  | −8.418                                                        | 1.950                                    | −8.270                                                        | 1.915                                    |                             |                             |
| HF (2D)  | 3.908                                                         | 1.379                                    | 3.802                                                         | 1.317                                    |                             |                             |
| LDA (1D) | −3.381                                                        | 1.876                                    | −3.321                                                        | 1.842                                    |                             |                             |
| LDA (2D) | 1.766                                                         | −2.768                                   | 1.741                                                         | −2.713                                   |                             |                             |
|          | $\Delta A/A \times 10^{14}$                                   | $\Delta B/B \times 10^{14}$              | $\Delta C/C \times 10^{14}$                                   | $\Delta A/A \times 10^{14}$              | $\Delta B/B \times 10^{14}$ | $\Delta C/C \times 10^{14}$ |
| HF       | 1.431                                                         | −5.609                                   | 2.991                                                         | 1.418                                    | −5.505                      | 2.937                       |
| LDA      | −0.726                                                        | 1.615                                    | −2.420                                                        | −0.714                                   | 1.585                       | −2.376                      |

## 2 Computational details and data of calculations of PV shifts in vibrational spectra

The equilibrium structure of  $(R)\text{-CpRe}(\text{CH}_3)(\text{CO})(\text{NO})$  is taken from the earlier study by Schnell and coworkers<sup>1</sup>. Structure optimizations and harmonic force field calculation were performed at B3LYP level of theory with the Gaussian 09 program package,<sup>3</sup> using the correlation consistent polarized quintuple zeta basis set (cc-pV5Z) on period 1-3 atoms (H, C, N and O) whereas the cc-pwCVQZ-PP basis set and an energy-consistent pseudo-potential of the Stuttgart group<sup>4,5</sup> were employed on rhenium atom. Calculations of anharmonic vibrational force fields were performed on the above optimized structure employing a hybrid approach<sup>6</sup> within the Gaussian program package assuming that the normal modes from two levels of theories are similar. Harmonic force field data at B3LYP/cc-pV5Z,cc-pwCVQZ-PP level was utilized for the computation of anharmonic contributions at a lower level. The latter have been computed at B3LYP level using the scalar relativistic Stuttgart pseudo potential together with an energy-optimized valence basis set with a (12s11p10d8f)/[8s7p6d4f] contraction on Re atom<sup>7</sup> and cc-pVDZ basis set for H, C, N and O atoms.

Subsequently, PV energies were calculated as described in the computational details section at fixed nuclear coordinates for  $(R)\text{-CpRe}(\text{CH}_3)(\text{CO})(\text{NO})$  containing either  $^{187}\text{Re}$  or  $^{185}\text{Re}$  isotopes of Re. According to the procedure described in Ref. 8, a one-dimensional cut through the PV potential hypersurfaces  $E_{PV}(\vec{q})$  along the dimensionless reduced normal coordinate  $q_9$  and  $q_{10}$  corresponding to the  $-\text{CO}$  and  $-\text{NO}$  stretching modes of  $(R)\text{-Cp}^{187}\text{Re}(\text{CH}_3)(\text{CO})(\text{NO})$  and  $(R)\text{-Cp}^{185}\text{Re}(\text{CH}_3)(\text{CO})(\text{NO})$  are approximated. Due to the choice of phase in the computation of dimensionless reduced normal coordinates a bond expansion is observed for N–O bond in the direction  $q_{10} = -3.0$  to  $q_{10} = 3.0$ , whereas a bond compression for the C–O stretching vibration is observed in the direction of  $q_9 = -3.0$  to  $q_9 = 3.0$ . Figure S1 depicts the variation of the parity conserving and parity violating energies along the respective dimensionless reduced normal coordinates. Both of the coordinates are aligned from bond compression (left) to bond expansion (right) so that the abscissa read as  $q_{NO}$  and  $-q_{CO}$ . The variation of parity violating energies are similar for LDA, BLYP and B3LYP levels, whereas the curves for HF is far from the DFT ones, indicating that the HF method may not be very useful for compounds containing transition metals such as Re.

The current work employs a perturbative approach<sup>9</sup> for estimating the relative PV vibrational frequency splittings in the enantiomers of  $\text{CpRe}(\text{CH}_3)(\text{CO})(\text{NO})$  where the PC and PV potentials are expanded in a Taylor series. In this, the influence of multi-mode effects<sup>10–13</sup> are estimated by the calculations of the derivatives of the PV potentials with

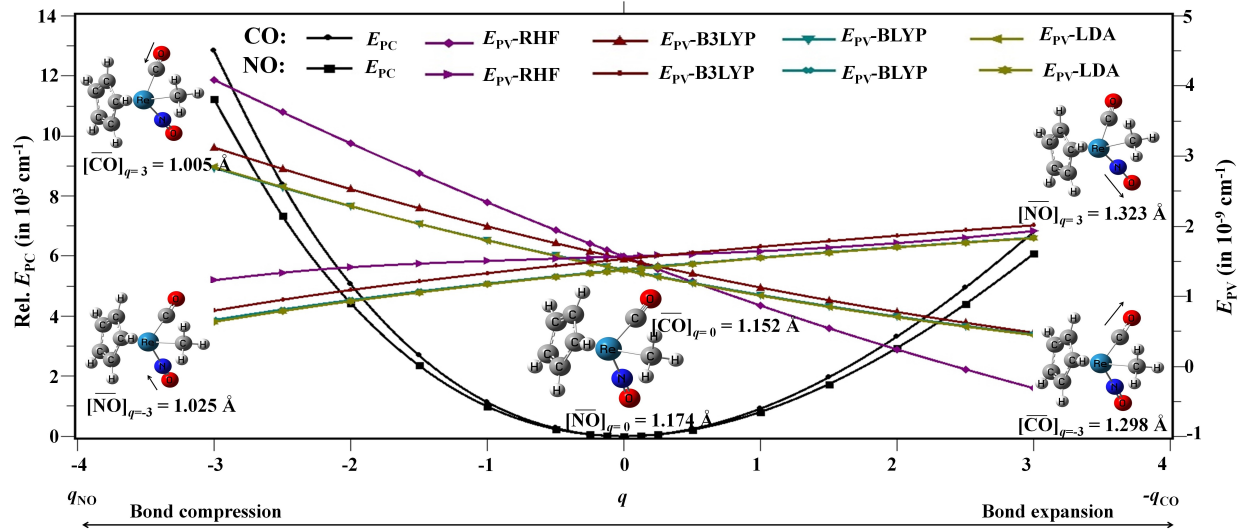

Figure S1: Variation of the parity conserving and parity violating energies along the dimensionless reduced normal coordinates of  $q_9$  and  $q_{10}$  for  $(R)\text{-Cp}^{187}\text{Re}(\text{CH}_3)(\text{CO})(\text{NO})$  structure optimized at B3LYP/cc-pV5Z,cc-pwCVQZ-PP level of theory.

respect to all normal coordinates as described in our recent paper 10. The second derivatives of the PV potential  $\frac{\partial^2 E_{\text{PV}}}{\partial q^2}$  are computed semi-numerical from a linear fit of  $\frac{\partial E_{\text{PV}}}{\partial q}$  evaluated at three points (viz.  $q = -0.125, 0.0$  and  $+0.125$ ) close to the minimum.

Table S15: Cartesian displacements (in Å) corresponding to a unit shift along the dimensionless reduced normal coordinates for  $\nu_9$  and  $\nu_{10}$  of  $\text{Cp}^{187}\text{Re}(\text{CH}_3)(\text{CO})(\text{NO})$  from the molecular structure optimized at the level RECP-B3LYP/cc-pV5Z,cc-pwCVQZ-PP.

| Mode       | Atom | $x$           | $y$           | $z$           |
|------------|------|---------------|---------------|---------------|
| $\nu_9$    | C    | -0.0002374615 | -0.0001115604 | -0.0000457018 |
|            | H    | -0.0002266901 | 0.0004605104  | -0.0000236219 |
|            | C    | 0.0000828887  | -0.0000355733 | -0.0000608315 |
|            | H    | 0.0000519750  | -0.0000821230 | 0.0001473078  |
|            | C    | -0.0000884880 | -0.0002280144 | -0.0000101590 |
|            | H    | -0.0001805629 | 0.0002924403  | -0.0000128248 |
|            | C    | 0.0002655930  | -0.0001805658 | 0.0000999434  |
|            | H    | 0.0002990616  | 0.0012117607  | -0.0000050270 |
|            | C    | 0.0000390316  | -0.0001805221 | -0.0000939642 |
|            | H    | -0.0000852249 | 0.0000333921  | -0.0000065654 |
|            | Re   | 0.0000901767  | -0.0000653103 | -0.0000234949 |
|            | C    | -0.0157455122 | 0.0143008229  | 0.0193709158  |
|            | N    | -0.0006852353 | 0.0023979786  | -0.0028988264 |
|            | O    | 0.0108533925  | -0.0099128736 | -0.0134744468 |
|            | O    | 0.0004848993  | -0.0015877903 | 0.0019470246  |
|            | C    | 0.0002230561  | -0.0000663082 | -0.0001152978 |
|            | H    | -0.0002554712 | -0.0007085339 | -0.0005732117 |
|            | H    | -0.0016830097 | 0.0001635231  | -0.0003000361 |
|            | H    | -0.0009840139 | -0.0007718247 | 0.0004030832  |
| $\nu_{10}$ | C    | -0.0001418225 | 0.0004195308  | 0.0000314520  |
|            | H    | 0.0000428854  | -0.0001238880 | 0.0000840136  |
|            | C    | 0.0000239685  | 0.0001844626  | -0.0003507102 |
|            | H    | -0.0002254493 | 0.0000901324  | 0.0002779352  |
|            | C    | 0.0002313246  | 0.0000041441  | 0.0000126466  |
|            | H    | 0.0002788477  | -0.0007722002 | -0.0000254368 |
|            | C    | 0.0000482671  | 0.0000454901  | -0.0002350969 |
|            | H    | 0.0002357047  | 0.0002074913  | 0.0003254524  |
|            | C    | -0.0002340184 | 0.0001458981  | 0.0000585136  |
|            | H    | -0.0001022528 | -0.0012914912 | -0.0000488929 |
|            | Re   | -0.0000869796 | 0.0001971977  | -0.0002455231 |
|            | C    | -0.0023293688 | 0.0022509305  | 0.0024269308  |
|            | N    | 0.0058019415  | -0.0180470511 | 0.0218663433  |
|            | O    | 0.0017529440  | -0.0016412570 | -0.0020802643 |
|            | O    | -0.0041626684 | 0.0128089472  | -0.0156122871 |
|            | C    | -0.0001192358 | 0.0000668338  | -0.0002701783 |
|            | H    | 0.0009443691  | 0.0008161218  | 0.0010757190  |
|            | H    | 0.0022161629  | 0.0001448707  | 0.0011196348  |
|            | H    | 0.0003904334  | 0.0007435595  | -0.0002145768 |

Table S16: Cartesian displacements (in Å) corresponding to a unit shift along the dimensionless reduced normal coordinates for  $\nu_9$  and  $\nu_{10}$  of  $\text{Cp}^{185}\text{Re}(\text{CH}_3)(\text{CO})(\text{NO})$  from the molecular structure optimized at the level RECP-B3LYP/cc-pV5Z,cc-pwCVQZ-PP.

| Mode       | Atom | $x$           | $y$           | $z$           |
|------------|------|---------------|---------------|---------------|
| $\nu_9$    | C    | -0.0002374650 | -0.0001115516 | -0.0000457049 |
|            | H    | -0.0002266988 | 0.0004604768  | -0.0000236306 |
|            | C    | 0.0000828723  | -0.0000355632 | -0.0000608375 |
|            | H    | 0.0000519459  | -0.0000821073 | 0.0001473048  |
|            | C    | -0.0000885049 | -0.0002279982 | -0.0000101385 |
|            | H    | -0.0001806021 | 0.0002924860  | -0.0000127956 |
|            | C    | 0.0002655876  | -0.0001805630 | 0.0000999536  |
|            | H    | 0.0002990528  | 0.0012116975  | -0.0000050263 |
|            | C    | 0.0000390358  | -0.0001805105 | -0.0000939670 |
|            | H    | -0.0000852289 | 0.0000333634  | -0.0000065567 |
|            | Re   | 0.0000911688  | -0.0000660328 | -0.0000237511 |
|            | C    | -0.0157455332 | 0.0143008378  | 0.0193708880  |
|            | N    | -0.0006853210 | 0.0023981276  | -0.0028989247 |
|            | O    | 0.0108533449  | -0.0099128231 | -0.0134743711 |
|            | O    | 0.0004849276  | -0.0015878387 | 0.0019470635  |
|            | C    | 0.0002230240  | -0.0000663022 | -0.0001152951 |
|            | H    | -0.0002556184 | -0.0007086260 | -0.0005733092 |
|            | H    | -0.0016829719 | 0.0001635446  | -0.0003000231 |
|            | H    | -0.0009840764 | -0.0007718477 | 0.0004030965  |
| $\nu_{10}$ | C    | -0.0001418197 | 0.0004194866  | 0.0000315770  |
|            | H    | 0.0000428855  | -0.0001240402 | 0.0000841988  |
|            | C    | 0.0000240518  | 0.0001844309  | -0.0003507448 |
|            | H    | -0.0002253837 | 0.0000901166  | 0.0002780354  |
|            | C    | 0.0002312935  | 0.0000040890  | 0.0000126394  |
|            | H    | 0.0002788956  | -0.0007720280 | -0.0000253966 |
|            | C    | 0.0000482028  | 0.0000454428  | -0.0002351311 |
|            | H    | 0.0002356635  | 0.0002074996  | 0.0003255808  |
|            | C    | -0.0002339731 | 0.0001458484  | 0.0000585438  |
|            | H    | -0.0001022500 | -0.0012912011 | -0.0000488301 |
|            | Re   | -0.0000879420 | 0.0001993934  | -0.0002482489 |
|            | C    | -0.0023294203 | 0.0022509278  | 0.0024272057  |
|            | N    | 0.0058019760  | -0.0180471342 | 0.0218663671  |
|            | O    | 0.0017529919  | -0.0016412885 | -0.0020803772 |
|            | O    | -0.0041625561 | 0.0128085370  | -0.0156118021 |
|            | C    | -0.0001191844 | 0.0000667967  | -0.0002700860 |
|            | H    | 0.0009442960  | 0.0008158966  | 0.0010757787  |
|            | H    | 0.0022157713  | 0.0001447803  | 0.0011197050  |
|            | H    | 0.0003911280  | 0.0007439072  | -0.0002145290 |

Table S17: HF and LDA level PV energy gradients (in  $10^{-10} \text{ cm}^{-1}$ ) along the dimensionless reduced normal coordinates  $q = -0.125, +0.00$  and  $+0.125$  corresponding to  $\nu_9$  and  $\nu_{10}$  of  $\text{Cp}^{187}\text{Re}(\text{CH}_3)(\text{CO})(\text{NO})$  and  $\text{Cp}^{185}\text{Re}(\text{CH}_3)(\text{CO})(\text{NO})$  from the molecular structure optimized at the level RECP-B3LYP/cc-pV5Z,cc-pwCVQZ-PP.

| level→                                                                          | HF       |         |          | LDA      |         |          |
|---------------------------------------------------------------------------------|----------|---------|----------|----------|---------|----------|
| $q \rightarrow$                                                                 | $-0.125$ | $+0.00$ | $+0.125$ | $-0.125$ | $+0.00$ | $+0.125$ |
| <b><math>\text{Cp}^{187}\text{Re}(\text{CH}_3)(\text{CO})(\text{NO})</math></b> |          |         |          |          |         |          |
| $\nu_9$                                                                         | 7.276    | 7.367   | 7.459    | 3.856    | 3.932   | 4.010    |
| $\nu_{10}$                                                                      | 0.621    | 0.635   | 0.654    | 1.906    | 1.868   | 1.832    |
| <b><math>\text{Cp}^{185}\text{Re}(\text{CH}_3)(\text{CO})(\text{NO})</math></b> |          |         |          |          |         |          |
| $\nu_9$                                                                         | 7.148    | 7.238   | 7.327    | 3.788    | 3.863   | 3.939    |
| $\nu_{10}$                                                                      | 0.610    | 0.624   | 0.643    | 1.872    | 1.835   | 1.800    |

Table S18: Unscaled fundamental harmonic and anharmonic wavenumbers  $\tilde{\omega}$  (in  $\text{cm}^{-1}$ ) and corresponding intensities (in  $\text{km/mol}$ ) as obtained for the equilibrium structure of  $\text{Cp}^{187}\text{Re}(\text{CH}_3)(\text{CO})(\text{NO})$ . B3LYP/cc-pV5Z,cc-pwCVQZ-PP level harmonic force field was utilised for the anhamonic calculation at B3LYP level with (12s11p10d8f)/[8s7p6d4f] contraction on Re atom and cc-pVDZ basis set for H, C, N and O atoms. Masses used (in  $u$ ) for the harmonic force field calculation are 1.008, 12.000, 14.003, 15.995, 184.953, and 186.956 respectively for H, C, N, O,  $^{185}\text{Re}$  and  $^{187}\text{Re}$  atoms.

| Molecules→                       | Harmonic         |           | Anharmonic       |           |
|----------------------------------|------------------|-----------|------------------|-----------|
| modes ↓                          | $\tilde{\omega}$ | Intensity | $\tilde{\omega}$ | Intensity |
| $\nu_1$                          | 3257.185         | 0.23      | 3130.891         | 2.73      |
| $\nu_2$                          | 3249.319         | 0.03      | 3105.795         | 0.43      |
| $\nu_3$                          | 3244.545         | 0.10      | 3131.651         | 2.67      |
| $\nu_4$                          | 3235.582         | 0.12      | 3096.794         | 0.92      |
| $\nu_5$                          | 3231.059         | 0.13      | 3079.022         | 1.30      |
| $\nu_6$                          | 3106.092         | 21.82     | 2971.460         | 26.52     |
| $\nu_7$                          | 3080.915         | 25.10     | 2945.858         | 48.85     |
| $\nu_8$                          | 3016.802         | 47.32     | 2913.357         | 44.02     |
| $\nu_9$ ( $\nu_{\text{CO}}$ )    | 2029.103         | 944.08    | 2000.699         | 720.32    |
| $\nu_{10}$ ( $\nu_{\text{NO}}$ ) | 1781.451         | 1120.17   | 1745.610         | 22.71     |
| $\nu_{11}$                       | 1484.623         | 4.08      | 1429.273         | 1.75      |
| $\nu_{12}$                       | 1475.124         | 4.12      | 1422.076         | 3.03      |
| $\nu_{13}$                       | 1464.553         | 5.10      | 1429.506         | 8.06      |
| $\nu_{14}$                       | 1460.182         | 1.77      | 1425.642         | 2.76      |
| $\nu_{15}$                       | 1384.608         | 2.91      | 1343.193         | 3.60      |
| $\nu_{16}$                       | 1377.159         | 2.19      | 1336.353         | 1.47      |
| $\nu_{17}$                       | 1298.092         | 0.00      | 1271.617         | 0.19      |
| $\nu_{18}$                       | 1258.477         | 8.84      | 1218.616         | 14.38     |
| $\nu_{19}$                       | 1130.039         | 2.03      | 1108.270         | 0.73      |
| $\nu_{20}$                       | 1086.339         | 0.60      | 1072.805         | 0.52      |
| $\nu_{21}$                       | 1078.457         | 0.73      | 1064.530         | 0.73      |
| $\nu_{22}$                       | 1029.650         | 5.69      | 1012.006         | 14.02     |
| $\nu_{23}$                       | 1019.231         | 8.56      | 1001.361         | 8.30      |
| $\nu_{24}$                       | 946.191          | 3.17      | 919.984          | 4.93      |
| $\nu_{25}$                       | 927.992          | 1.39      | 903.470          | 0.76      |
| $\nu_{26}$                       | 858.176          | 1.86      | 846.655          | 0.63      |
| $\nu_{27}$                       | 853.026          | 1.60      | 825.610          | 15.99     |
| $\nu_{28}$                       | 849.506          | 8.21      | 853.179          | 2.57      |
| $\nu_{29}$                       | 834.941          | 7.01      | 810.541          | 6.00      |
| $\nu_{30}$                       | 828.495          | 49.70     | 803.992          | 47.98     |
| $\nu_{31}$                       | 820.449          | 3.11      | 782.947          | 0.84      |
| $\nu_{32}$                       | 798.679          | 4.06      | 768.231          | 9.34      |
| $\nu_{33}$                       | 641.103          | 5.94      | 633.667          | 6.52      |
| $\nu_{34}$                       | 621.375          | 4.52      | 612.636          | 12.90     |
| $\nu_{35}$                       | 613.273          | 18.78     | 606.213          | 15.57     |
| $\nu_{36}$                       | 605.007          | 3.04      | 593.783          | 3.81      |
| $\nu_{37}$                       | 581.705          | 16.26     | 569.204          | 12.58     |
| $\nu_{38}$                       | 530.007          | 6.68      | 519.194          | 5.00      |
| $\nu_{39}$                       | 504.694          | 8.62      | 504.722          | 7.10      |
| $\nu_{40}$                       | 499.315          | 8.14      | 485.667          | 3.84      |
| $\nu_{41}$                       | 483.751          | 16.80     | 474.378          | 15.16     |
| $\nu_{42}$                       | 335.594          | 3.89      | 327.962          | 5.81      |
| $\nu_{43}$                       | 299.473          | 3.66      | 290.279          | 61.58     |
| $\nu_{44}$                       | 287.540          | 0.65      | 280.574          | 0.87      |
| $\nu_{45}$                       | 185.792          | 1.30      | 153.128          | 1.06      |
| $\nu_{46}$                       | 172.384          | 0.23      | 92.868           | 0.05      |
| $\nu_{47}$                       | 138.031          | 0.24      | 143.229          | 0.21      |
| $\nu_{48}$                       | 99.218           | 0.14      | 96.282           | 0.52      |
| $\nu_{49}$                       | 94.048           | 0.15      | 91.340           | 0.53      |
| $\nu_{50}$                       | 78.475           | 0.08      | 74.026           | 0.30      |

Table S19: Unscaled harmonic and anharmonic wavenumbers  $\tilde{\omega}$  (in  $\text{cm}^{-1}$ ) and corresponding anharmonic intensities (in  $\text{km/mol}$ ) for the overtone bands as obtained for the equilibrium structure of  $\text{Cp}^{187}\text{Re}(\text{CH}_3)(\text{CO})(\text{NO})$ . B3LYP/cc-pV5Z,cc-pwCVQZ-PP level harmonic force field was utilised for the anharmonic calculation at B3LYP level with (12s11p10d8f)/[8s7p6d4f] contraction on Re atom and cc-pVDZ basis set for H, C, N and O atoms. Masses used (in  $u$ ) for the harmonic force field calculation are 1.008, 12.000, 14.003, 15.995, 184.953, and 186.956 respectively for H, C, N, O,  $^{185}\text{Re}$  and  $^{187}\text{Re}$  atoms.

| Molecules→                  | Harmonic         | Anharmonic       |           |
|-----------------------------|------------------|------------------|-----------|
| modes ↓                     | $\tilde{\omega}$ | $\tilde{\omega}$ | Intensity |
| $\nu_1$                     | 6514.37          | 6238.568         | 0.00      |
| $\nu_2$                     | 6498.64          | 6185.335         | 0.12      |
| $\nu_3$                     | 6489.09          | 6207.890         | 0.02      |
| $\nu_4$                     | 6471.16          | 6076.373         | 0.90      |
| $\nu_5$                     | 6462.12          | 6141.587         | 0.94      |
| $\nu_6$                     | 6212.18          | 5823.130         | 0.41      |
| $\nu_7$                     | 6161.83          | 5758.677         | 0.67      |
| $\nu_8$                     | 6033.60          | 5695.575         | 0.02      |
| $\nu_9(\nu_{\text{CO}})$    | 4058.21          | 3974.674         | 9.46      |
| $\nu_{10}(\nu_{\text{NO}})$ | 3562.90          | 3460.279         | 20.88     |
| $\nu_{11}$                  | 2969.25          | 2862.564         | 0.77      |
| $\nu_{12}$                  | 2950.25          | 2782.828         | 17.00     |
| $\nu_{13}$                  | 2929.11          | 2854.413         | 0.00      |
| $\nu_{14}$                  | 2920.37          | 2842.476         | 0.00      |
| $\nu_{15}$                  | 2769.22          | 2676.892         | 0.04      |
| $\nu_{16}$                  | 2754.32          | 2661.605         | 0.04      |
| $\nu_{17}$                  | 2596.18          | 2539.750         | 0.00      |
| $\nu_{18}$                  | 2516.96          | 2414.027         | 0.53      |
| $\nu_{19}$                  | 2260.08          | 2213.184         | 0.01      |
| $\nu_{20}$                  | 2172.68          | 2146.491         | 0.10      |
| $\nu_{21}$                  | 2156.91          | 2129.810         | 0.09      |
| $\nu_{22}$                  | 2059.30          | 2022.164         | 0.02      |
| $\nu_{23}$                  | 2038.46          | 2000.986         | 0.03      |
| $\nu_{24}$                  | 1892.38          | 1828.444         | 1.18      |
| $\nu_{25}$                  | 1855.98          | 1801.983         | 1.64      |
| $\nu_{26}$                  | 1716.35          | 1691.820         | 0.02      |
| $\nu_{27}$                  | 1706.05          | 1672.324         | 0.54      |
| $\nu_{28}$                  | 1699.01          | 1660.230         | 0.59      |
| $\nu_{29}$                  | 1669.88          | 1615.136         | 1.37      |
| $\nu_{30}$                  | 1656.99          | 1600.154         | 1.55      |
| $\nu_{31}$                  | 1640.90          | 1585.122         | 0.10      |
| $\nu_{32}$                  | 1597.36          | 1536.431         | 0.31      |
| $\nu_{33}$                  | 1282.21          | 1263.590         | 0.47      |
| $\nu_{34}$                  | 1242.75          | 1217.650         | 0.20      |
| $\nu_{35}$                  | 1226.55          | 1211.972         | 0.06      |
| $\nu_{36}$                  | 1210.01          | 1193.549         | 0.12      |
| $\nu_{37}$                  | 1163.41          | 1136.530         | 0.42      |
| $\nu_{38}$                  | 1060.01          | 1036.318         | 0.93      |
| $\nu_{39}$                  | 1009.39          | 991.569          | 0.08      |
| $\nu_{40}$                  | 998.63           | 983.889          | 0.04      |
| $\nu_{41}$                  | 967.50           | 947.640          | 0.68      |
| $\nu_{42}$                  | 671.19           | 652.878          | 0.06      |
| $\nu_{43}$                  | 598.95           | 576.744          | 1.70      |
| $\nu_{44}$                  | 575.08           | 560.001          | 0.27      |
| $\nu_{45}$                  | 371.58           | 298.968          | 0.01      |
| $\nu_{46}$                  | 344.77           | 156.012          | 0.02      |
| $\nu_{47}$                  | 276.06           | 260.706          | 0.00      |
| $\nu_{48}$                  | 198.44           | 191.927          | 0.00      |
| $\nu_{49}$                  | 188.10           | 182.090          | 0.01      |
| $\nu_{50}$                  | 156.95           | 147.442          | 0.00      |

Table S20: Unscaled fundamental harmonic and anharmonic wavenumbers  $\tilde{\omega}$  (in  $\text{cm}^{-1}$ ) and corresponding intensities (in  $\text{km/mol}$ ) as obtained for the equilibrium structure of  $\text{Cp}^{185}\text{Re}(\text{CH}_3)(\text{CO})(\text{NO})$ . B3LYP/cc-pV5Z,cc-pwCVQZ-PP level harmonic force field was utilised for the anhamonic calculation at B3LYP level with (12s11p10d8f)/[8s7p6d4f] contraction on Re atom and cc-pVDZ basis set for H, C, N and O atoms. Masses used (in  $u$ ) for the harmonic force field calculation are 1.008, 12.000, 14.003, 15.995, 184.953, and 186.956 respectively for H, C, N, O,  $^{185}\text{Re}$  and  $^{187}\text{Re}$  atoms.

| Molecules→                       | Harmonic         |           | Anharmonic       |           |
|----------------------------------|------------------|-----------|------------------|-----------|
| modes ↓                          | $\tilde{\omega}$ | Intensity | $\tilde{\omega}$ | Intensity |
| $\nu_1$                          | 3257.185         | 0.23      | 3130.854         | 1.99      |
| $\nu_2$                          | 3249.319         | 0.03      | 3105.733         | 1.28      |
| $\nu_3$                          | 3244.545         | 0.10      | 3131.595         | 4.79      |
| $\nu_4$                          | 3235.582         | 0.12      | 3096.845         | 0.75      |
| $\nu_5$                          | 3231.059         | 0.13      | 3078.940         | 1.28      |
| $\nu_6$                          | 3106.092         | 21.82     | 2971.587         | 26.04     |
| $\nu_7$                          | 3080.915         | 25.10     | 2945.689         | 58.39     |
| $\nu_8$                          | 3016.802         | 47.32     | 2912.979         | 50.09     |
| $\nu_9$ ( $\nu_{\text{CO}}$ )    | 2029.104         | 944.09    | 2000.562         | 695.33    |
| $\nu_{10}$ ( $\nu_{\text{NO}}$ ) | 1781.461         | 1120.22   | 1745.651         | 583.11    |
| $\nu_{11}$                       | 1484.623         | 4.08      | 1429.351         | 1.70      |
| $\nu_{12}$                       | 1475.124         | 4.12      | 1421.466         | 1.04      |
| $\nu_{13}$                       | 1464.553         | 5.10      | 1429.697         | 10.10     |
| $\nu_{14}$                       | 1460.183         | 1.77      | 1425.862         | 2.33      |
| $\nu_{15}$                       | 1384.608         | 2.91      | 1343.220         | 2.87      |
| $\nu_{16}$                       | 1377.159         | 2.19      | 1336.500         | 1.13      |
| $\nu_{17}$                       | 1298.092         | 0.00      | 1271.619         | 0.16      |
| $\nu_{18}$                       | 1258.479         | 8.84      | 1218.986         | 23.50     |
| $\nu_{19}$                       | 1130.040         | 2.03      | 1108.485         | 1.16      |
| $\nu_{20}$                       | 1086.340         | 0.60      | 1072.576         | 0.47      |
| $\nu_{21}$                       | 1078.457         | 0.73      | 1064.536         | 0.73      |
| $\nu_{22}$                       | 1029.652         | 5.69      | 1012.122         | 16.30     |
| $\nu_{23}$                       | 1019.232         | 8.56      | 1001.338         | 11.74     |
| $\nu_{24}$                       | 946.191          | 3.17      | 919.989          | 6.43      |
| $\nu_{25}$                       | 927.992          | 1.39      | 903.595          | 0.39      |
| $\nu_{26}$                       | 858.177          | 1.86      | 846.667          | 0.61      |
| $\nu_{27}$                       | 853.029          | 1.60      | 825.780          | 17.16     |
| $\nu_{28}$                       | 849.511          | 8.21      | 853.060          | 2.38      |
| $\nu_{29}$                       | 834.958          | 6.97      | 811.084          | 6.85      |
| $\nu_{30}$                       | 828.504          | 49.72     | 804.319          | 48.35     |
| $\nu_{31}$                       | 820.464          | 3.12      | 782.329          | 1.27      |
| $\nu_{32}$                       | 798.713          | 4.08      | 768.396          | 11.58     |
| $\nu_{33}$                       | 641.411          | 5.86      | 633.996          | 6.25      |
| $\nu_{34}$                       | 621.518          | 4.77      | 613.774          | 21.08     |
| $\nu_{35}$                       | 613.368          | 18.79     | 606.340          | 19.75     |
| $\nu_{36}$                       | 605.073          | 2.90      | 593.859          | 4.82      |
| $\nu_{37}$                       | 581.858          | 16.23     | 569.040          | 16.62     |
| $\nu_{38}$                       | 530.023          | 6.69      | 518.707          | 2.80      |
| $\nu_{39}$                       | 504.909          | 8.81      | 507.055          | 13.30     |
| $\nu_{40}$                       | 499.506          | 8.13      | 484.265          | 17.75     |
| $\nu_{41}$                       | 483.799          | 16.71     | 474.410          | 14.19     |
| $\nu_{42}$                       | 335.707          | 3.88      | 328.927          | 14.88     |
| $\nu_{43}$                       | 299.546          | 3.66      | 290.169          | 70.44     |
| $\nu_{44}$                       | 287.902          | 0.65      | 281.412          | 5.11      |
| $\nu_{45}$                       | 185.839          | 1.30      | 153.823          | 1.01      |
| $\nu_{46}$                       | 172.399          | 0.23      | 92.865           | 0.07      |
| $\nu_{47}$                       | 138.101          | 0.24      | 143.997          | 0.21      |
| $\nu_{48}$                       | 99.279           | 0.14      | 96.271           | 0.97      |
| $\nu_{49}$                       | 94.112           | 0.15      | 90.739           | 0.87      |
| $\nu_{50}$                       | 78.519           | 0.08      | 73.990           | 0.45      |

Table S21: Unscaled harmonic and anharmonic wavenumbers  $\tilde{\omega}$  (in  $\text{cm}^{-1}$ ) and corresponding anharmonic intensities (in  $\text{km/mol}$ ) for the overtone bands as obtained for the equilibrium structure of  $\text{Cp}^{185}\text{Re}(\text{CH}_3)(\text{CO})(\text{NO})$ . B3LYP/cc-pV5Z,cc-pwCVQZ-PP level harmonic force field was utilised for the anharmonic calculation at B3LYP level with (12s11p10d8f)/[8s7p6d4f] contraction on Re atom and cc-pVDZ basis set for H, C, N and O atoms. Masses used (in  $u$ ) for the harmonic force field calculation are 1.008, 12.000, 14.003, 15.995, 184.953, and 186.956 respectively for H, C, N, O,  $^{185}\text{Re}$  and  $^{187}\text{Re}$  atoms.

| Molecules→                  | Harmonic         | Anharmonic       |           |
|-----------------------------|------------------|------------------|-----------|
| modes ↓                     | $\tilde{\omega}$ | $\tilde{\omega}$ | Intensity |
| $\nu_1$                     | 6514.37          | 6238.503         | 0.00      |
| $\nu_2$                     | 6498.64          | 6185.108         | 0.12      |
| $\nu_3$                     | 6489.09          | 6207.840         | 0.02      |
| $\nu_4$                     | 6471.16          | 6076.332         | 0.90      |
| $\nu_5$                     | 6462.12          | 6141.593         | 0.94      |
| $\nu_6$                     | 6212.18          | 5823.222         | 0.42      |
| $\nu_7$                     | 6161.83          | 5758.530         | 0.67      |
| $\nu_8$                     | 6033.60          | 5695.349         | 0.02      |
| $\nu_9(\nu_{\text{CO}})$    | 4058.21          | 3974.382         | 9.46      |
| $\nu_{10}(\nu_{\text{NO}})$ | 3562.92          | 3460.415         | 20.88     |
| $\nu_{11}$                  | 2969.25          | 2862.170         | 0.79      |
| $\nu_{12}$                  | 2950.25          | 2782.273         | 19.40     |
| $\nu_{13}$                  | 2929.11          | 2854.712         | 0.00      |
| $\nu_{14}$                  | 2920.37          | 2842.922         | 0.00      |
| $\nu_{15}$                  | 2769.22          | 2676.944         | 0.04      |
| $\nu_{16}$                  | 2754.32          | 2661.901         | 0.04      |
| $\nu_{17}$                  | 2596.18          | 2539.754         | 0.00      |
| $\nu_{18}$                  | 2516.96          | 2414.768         | 0.53      |
| $\nu_{19}$                  | 2260.08          | 2213.553         | 0.01      |
| $\nu_{20}$                  | 2172.68          | 2146.048         | 0.10      |
| $\nu_{21}$                  | 2156.91          | 2129.824         | 0.09      |
| $\nu_{22}$                  | 2059.30          | 2022.398         | 0.02      |
| $\nu_{23}$                  | 2038.46          | 2000.940         | 0.03      |
| $\nu_{24}$                  | 1892.38          | 1828.456         | 1.18      |
| $\nu_{25}$                  | 1855.98          | 1802.375         | 1.64      |
| $\nu_{26}$                  | 1716.35          | 1691.844         | 0.02      |
| $\nu_{27}$                  | 1706.06          | 1672.223         | 0.54      |
| $\nu_{28}$                  | 1699.02          | 1660.253         | 0.58      |
| $\nu_{29}$                  | 1669.92          | 1615.055         | 1.37      |
| $\nu_{30}$                  | 1657.01          | 1600.266         | 1.54      |
| $\nu_{31}$                  | 1640.93          | 1585.562         | 0.10      |
| $\nu_{32}$                  | 1597.43          | 1536.741         | 0.31      |
| $\nu_{33}$                  | 1282.82          | 1264.234         | 0.47      |
| $\nu_{34}$                  | 1243.04          | 1219.424         | 0.20      |
| $\nu_{35}$                  | 1226.74          | 1212.177         | 0.06      |
| $\nu_{36}$                  | 1210.15          | 1194.195         | 0.12      |
| $\nu_{37}$                  | 1163.72          | 1135.761         | 0.42      |
| $\nu_{38}$                  | 1060.05          | 1035.328         | 0.93      |
| $\nu_{39}$                  | 1009.82          | 991.504          | 0.08      |
| $\nu_{40}$                  | 999.01           | 986.394          | 0.04      |
| $\nu_{41}$                  | 967.60           | 947.733          | 0.68      |
| $\nu_{42}$                  | 671.42           | 654.572          | 0.06      |
| $\nu_{43}$                  | 599.09           | 576.475          | 1.71      |
| $\nu_{44}$                  | 575.81           | 561.670          | 0.28      |
| $\nu_{45}$                  | 371.68           | 300.414          | 0.01      |
| $\nu_{46}$                  | 344.80           | 155.749          | 0.02      |
| $\nu_{47}$                  | 276.20           | 262.270          | 0.00      |
| $\nu_{48}$                  | 198.56           | 191.863          | 0.00      |
| $\nu_{49}$                  | 188.23           | 180.820          | 0.01      |
| $\nu_{50}$                  | 157.04           | 147.386          | 0.00      |

Table S22: Combination bands  $\tilde{\omega}$  (in  $\text{cm}^{-1}$ ) that have intensities (in  $\text{km/mol}$ ) larger than 0.5 units for the equilibrium structure of  $\text{Cp}^{187}\text{Re}(\text{CH}_3)(\text{CO})(\text{NO})$  and  $\text{Cp}^{185}\text{Re}(\text{CH}_3)(\text{CO})(\text{NO})$ . B3LYP/cc-pV5Z,cc-pwCVQZ-PP level harmonic force field was utilised for the anharmonic calculation at B3LYP level with (12s11p10d8f)/[8s7p6d4f] contraction on Re atom and cc-pVDZ basis set for H, C, N and O atoms. Masses used (in  $u$ ) for the harmonic force field calculation are 1.008, 12.000, 14.003, 15.995, 184.953, and 186.956 respectively for H, C, N, O,  $^{185}\text{Re}$  and  $^{187}\text{Re}$  atoms.

| $\text{Cp}^{187}\text{Re}(\text{CH}_3)(\text{CO})(\text{NO})$ |                  |           | $\text{Cp}^{185}\text{Re}(\text{CH}_3)(\text{CO})(\text{NO})$ |                  |           |
|---------------------------------------------------------------|------------------|-----------|---------------------------------------------------------------|------------------|-----------|
| modes ↓                                                       | $\tilde{\omega}$ | Intensity | modes ↓                                                       | $\tilde{\omega}$ | Intensity |
| $\nu_{29} + \nu_{24}$                                         | 1724.693         | 1603.89   | $\nu_{29} + \nu_{24}$                                         | 1724.640         | 1682.50   |
| $\nu_{12} + \nu_{11}$                                         | 2832.757         | 7.37      | $\nu_{27} + \nu_{25}$                                         | 1734.942         | 1577.98   |
| $\nu_{50} + \nu_{39}$                                         | 572.876          | 5.50      | $\nu_{12} + \nu_{11}$                                         | 2832.263         | 8.91      |
| $\nu_{48} + \nu_{39}$                                         | 593.809          | 4.45      | $\nu_{48} + \nu_{39}$                                         | 592.239          | 5.85      |
| $\nu_{34} + \nu_{10}$                                         | 2353.592         | 4.20      | $\nu_{50} + \nu_{39}$                                         | 572.586          | 4.79      |
| $\nu_{33} + \nu_{10}$                                         | 2376.903         | 3.83      | $\nu_{34} + \nu_{10}$                                         | 2354.514         | 4.22      |
| $\nu_{38} + \nu_{18}$                                         | 1737.324         | 3.45      | $\nu_{33} + \nu_{10}$                                         | 2377.288         | 3.89      |
| $\nu_{40} + \nu_9$                                            | 2494.201         | 3.32      | $\nu_{38} + \nu_{18}$                                         | 1737.193         | 3.46      |
| $\nu_{24} + \nu_{21}$                                         | 1982.928         | 2.57      | $\nu_{40} + \nu_9$                                            | 2495.278         | 3.26      |
| $\nu_{49} + \nu_{38}$                                         | 609.477          | 2.50      | $\nu_{49} + \nu_{38}$                                         | 608.672          | 2.63      |
| $\nu_{44} + \nu_{43}$                                         | 569.829          | 1.91      | $\nu_{33} + \nu_{29}$                                         | 1444.529         | 2.60      |
| $\nu_{33} + \nu_{16}$                                         | 1969.867         | 1.71      | $\nu_{24} + \nu_{21}$                                         | 1982.940         | 2.57      |
| $\nu_{35} + \nu_{28}$                                         | 1438.475         | 1.61      | $\nu_{42} + \nu_{40}$                                         | 822.744          | 2.23      |
| $\nu_{47} + \nu_{40}$                                         | 623.222          | 1.58      | $\nu_{33} + \nu_{16}$                                         | 1970.324         | 1.79      |
| $\nu_{36} + \nu_{10}$                                         | 2341.626         | 1.45      | $\nu_{44} + \nu_{43}$                                         | 570.555          | 1.76      |
| $\nu_{45} + \nu_{43}$                                         | 443.926          | 1.40      | $\nu_{35} + \nu_{28}$                                         | 1438.692         | 1.69      |
| $\nu_{35} + \nu_{10}$                                         | 2350.482         | 1.17      | $\nu_{47} + \nu_{40}$                                         | 626.268          | 1.51      |
| $\nu_{30} + \nu_{24}$                                         | 1716.362         | 1.16      | $\nu_{36} + \nu_{10}$                                         | 2342.027         | 1.39      |
| $\nu_{43} + \nu_{21}$                                         | 1355.754         | 1.13      | $\nu_{33} + \nu_{15}$                                         | 1977.046         | 1.35      |
| $\nu_{33} + \nu_{15}$                                         | 1976.679         | 1.09      | $\nu_{34} + \nu_{27}$                                         | 1447.288         | 1.30      |
| $\nu_{42} + \nu_{40}$                                         | 820.773          | 1.06      | $\nu_{45} + \nu_{43}$                                         | 444.604          | 1.28      |
| $\nu_{38} + \nu_{37}$                                         | 1086.560         | 1.02      | $\nu_{30} + \nu_{24}$                                         | 1716.423         | 1.16      |
| $\nu_{25} + \nu_{20}$                                         | 1976.659         | 0.99      | $\nu_{35} + \nu_{10}$                                         | 2350.747         | 1.14      |
| $\nu_{48} + \nu_{40}$                                         | 589.539          | 0.99      | $\nu_{38} + \nu_{37}$                                         | 1085.644         | 1.02      |
| $\nu_{39} + \nu_9$                                            | 2498.051         | 0.96      | $\nu_{39} + \nu_9$                                            | 2497.785         | 1.00      |
| $\nu_{49} + \nu_9$                                            | 2092.311         | 0.88      | $\nu_{25} + \nu_{20}$                                         | 1976.634         | 0.99      |
| $\nu_{28} + \nu_{25}$                                         | 1731.387         | 0.88      | $\nu_{43} + \nu_{21}$                                         | 1355.633         | 0.96      |
| $\nu_{34} + \nu_{27}$                                         | 1446.470         | 0.88      | $\nu_{48} + \nu_{40}$                                         | 590.681          | 0.96      |
| $\nu_{41} + \nu_{33}$                                         | 1107.065         | 0.87      | $\nu_{43} + \nu_{30}$                                         | 1094.540         | 0.89      |
| $\nu_{43} + \nu_{30}$                                         | 1094.554         | 0.85      | $\nu_{49} + \nu_9$                                            | 2091.370         | 0.88      |
| $\nu_{30} + \nu_{29}$                                         | 1608.146         | 0.83      | $\nu_{28} + \nu_{25}$                                         | 1731.597         | 0.87      |
| $\nu_{35} + \nu_{27}$                                         | 1443.718         | 0.73      | $\nu_{41} + \nu_{33}$                                         | 1107.390         | 0.86      |
| $\nu_{28} + \nu_{27}$                                         | 1667.026         | 0.67      | $\nu_{35} + \nu_{27}$                                         | 1443.780         | 0.86      |
| $\nu_{43} + \nu_{40}$                                         | 785.090          | 0.66      | $\nu_{30} + \nu_{29}$                                         | 1608.140         | 0.83      |
| $\nu_{50} + \nu_{10}$                                         | 1819.956         | 0.66      | $\nu_{28} + \nu_{27}$                                         | 1666.985         | 0.67      |
| $\nu_{51} + \nu_{43}$                                         | 324.016          | 0.60      | $\nu_{50} + \nu_{10}$                                         | 1820.122         | 0.66      |
| $\nu_{18} + \nu_{10}$                                         | 2964.253         | 0.59      | $\nu_{44} + \nu_{38}$                                         | 799.245          | 0.65      |
| $\nu_{51} + \nu_{10}$                                         | 1776.474         | 0.59      | $\nu_{51} + \nu_{43}$                                         | 325.196          | 0.60      |
| $\nu_{25} + \nu_{24}$                                         | 1821.008         | 0.58      | $\nu_{18} + \nu_{10}$                                         | 2964.689         | 0.59      |
| $\nu_{27} + \nu_{25}$                                         | 1735.423         | 0.58      | $\nu_{25} + \nu_{24}$                                         | 1821.216         | 0.58      |
| $\nu_{27} + \nu_{24}$                                         | 1753.129         | 0.57      | $\nu_{51} + \nu_{10}$                                         | 1776.671         | 0.57      |
| $\nu_{51} + \nu_9$                                            | 2031.230         | 0.56      | $\nu_{27} + \nu_{24}$                                         | 1753.087         | 0.57      |
| $\nu_{44} + \nu_{38}$                                         | 798.942          | 0.52      | $\nu_{51} + \nu_9$                                            | 2031.390         | 0.56      |
| $\nu_{47} + \nu_{10}$                                         | 1876.228         | 0.52      | $\nu_{46} + \nu_7$                                            | 3060.155         | 0.52      |
| $\nu_{46} + \nu_7$                                            | 3060.221         | 0.52      | $\nu_{41} + \nu_{37}$                                         | 1042.059         | 0.51      |
| $\nu_{41} + \nu_{37}$                                         | 1042.362         | 0.51      | $\nu_{47} + \nu_{10}$                                         | 1876.825         | 0.50      |

Table S23: Phases used for the normal modes for vibrational frequency splittings.

| Molecules→      | Cp <sup>187</sup> Re(CH <sub>3</sub> )(CO)(NO) | Cp <sup>185</sup> Re(CH <sub>3</sub> )(CO)(NO) |
|-----------------|------------------------------------------------|------------------------------------------------|
| v <sub>1</sub>  | 1.0                                            | 1.0                                            |
| v <sub>2</sub>  | 1.0                                            | 1.0                                            |
| v <sub>3</sub>  | 1.0                                            | 1.0                                            |
| v <sub>4</sub>  | 1.0                                            | 1.0                                            |
| v <sub>5</sub>  | -1.0                                           | -1.0                                           |
| v <sub>6</sub>  | -1.0                                           | -1.0                                           |
| v <sub>7</sub>  | 1.0                                            | 1.0                                            |
| v <sub>8</sub>  | 1.0                                            | 1.0                                            |
| v <sub>9</sub>  | 1.0                                            | 1.0                                            |
| v <sub>10</sub> | 1.0                                            | 1.0                                            |
| v <sub>11</sub> | 1.0                                            | 1.0                                            |
| v <sub>12</sub> | 1.0                                            | 1.0                                            |
| v <sub>13</sub> | 1.0                                            | 1.0                                            |
| v <sub>14</sub> | -1.0                                           | -1.0                                           |
| v <sub>15</sub> | 1.0                                            | 1.0                                            |
| v <sub>16</sub> | -1.0                                           | -1.0                                           |
| v <sub>17</sub> | 1.0                                            | 1.0                                            |
| v <sub>18</sub> | -1.0                                           | -1.0                                           |
| v <sub>19</sub> | -1.0                                           | -1.0                                           |
| v <sub>20</sub> | -1.0                                           | 1.0                                            |
| v <sub>21</sub> | -1.0                                           | -1.0                                           |
| v <sub>22</sub> | -1.0                                           | -1.0                                           |
| v <sub>23</sub> | 1.0                                            | 1.0                                            |
| v <sub>24</sub> | 1.0                                            | 1.0                                            |
| v <sub>25</sub> | -1.0                                           | -1.0                                           |
| v <sub>26</sub> | -1.0                                           | -1.0                                           |
| v <sub>27</sub> | 1.0                                            | -1.0                                           |
| v <sub>28</sub> | -1.0                                           | -1.0                                           |
| v <sub>29</sub> | 1.0                                            | 1.0                                            |
| v <sub>30</sub> | 1.0                                            | 1.0                                            |
| v <sub>31</sub> | -1.0                                           | -1.0                                           |
| v <sub>32</sub> | -1.0                                           | 1.0                                            |
| v <sub>33</sub> | 1.0                                            | 1.0                                            |
| v <sub>34</sub> | 1.0                                            | 1.0                                            |
| v <sub>35</sub> | 1.0                                            | 1.0                                            |
| v <sub>36</sub> | -1.0                                           | -1.0                                           |
| v <sub>37</sub> | 1.0                                            | 1.0                                            |
| v <sub>38</sub> | -1.0                                           | 1.0                                            |
| v <sub>39</sub> | -1.0                                           | -1.0                                           |
| v <sub>40</sub> | -1.0                                           | -1.0                                           |
| v <sub>41</sub> | 1.0                                            | -1.0                                           |
| v <sub>42</sub> | -1.0                                           | -1.0                                           |
| v <sub>43</sub> | 1.0                                            | 1.0                                            |
| v <sub>44</sub> | -1.0                                           | -1.0                                           |
| v <sub>45</sub> | 1.0                                            | 1.0                                            |
| v <sub>46</sub> | -1.0                                           | 1.0                                            |
| v <sub>47</sub> | 1.0                                            | 1.0                                            |
| v <sub>48</sub> | 1.0                                            | 1.0                                            |
| v <sub>49</sub> | 1.0                                            | 1.0                                            |
| v <sub>50</sub> | 1.0                                            | 1.0                                            |
| v <sub>51</sub> | 1.0                                            | 1.0                                            |

Table S24: Vibrationally averaged HF and LDA parity violating potential for energy levels  $n$  in  $10^{-9} \text{ cm}^{-1}$  for  $\nu_9$  and  $\nu_{10}$  of  $\text{Cp}^{187}\text{Re}(\text{CH}_3)(\text{CO})(\text{NO})$  and  $\text{Cp}^{185}\text{Re}(\text{CH}_3)(\text{CO})(\text{NO})$ .

| Mode                                              | $n$              | HF           |              |                             | LDA          |              |                             |
|---------------------------------------------------|------------------|--------------|--------------|-----------------------------|--------------|--------------|-----------------------------|
|                                                   |                  | Perturbed 1D | Perturbed 2D | 2D effects (%) <sup>c</sup> | Perturbed 1D | Perturbed 2D | 2D effects (%) <sup>c</sup> |
| <b>Cp<sup>187</sup>Re(CH<sub>3</sub>)(CO)(NO)</b> |                  |              |              |                             |              |              |                             |
| $\nu_9$                                           | 0                | 1.5251       | 1.5877       | 4.10                        | 1.3547       | 1.3808       | 1.93                        |
|                                                   | 1                | 1.4397       | 1.6273       | 13.03                       | 1.3204       | 1.3987       | 5.93                        |
|                                                   | 2                | 1.3543       | 1.6670       | 23.09                       | 1.2861       | 1.4166       | 10.15                       |
|                                                   | 3                | 1.2689       | 1.7066       | 34.49                       | 1.2518       | 1.4345       | 14.60                       |
|                                                   | $1 \leftarrow 0$ | -0.0854      | 0.0396       | -146.4                      | -0.0343      | 0.0179       | -152.23                     |
| $\nu_{10}$                                        | 0                | 1.5765       | 1.5740       | -0.16                       | 1.3802       | 1.3595       | -1.50                       |
|                                                   | 1                | 1.5939       | 1.5863       | -0.48                       | 1.3969       | 1.3348       | -4.44                       |
|                                                   | 2                | 1.6113       | 1.5985       | -0.79                       | 1.4136       | 1.3102       | -7.32                       |
|                                                   | 3                | 1.6286       | 1.6108       | -1.09                       | 1.4303       | 1.2855       | -10.12                      |
|                                                   | $1 \leftarrow 0$ | 0.0174       | 0.0123       | -29.28                      | 0.0167       | -0.0247      | -247.58                     |
| <b>Cp<sup>185</sup>Re(CH<sub>3</sub>)(CO)(NO)</b> |                  |              |              |                             |              |              |                             |
| $\nu_9$                                           | 0                | 1.4981       | 1.5594       | 4.09                        | 1.3307       | 1.3564       | 1.93                        |
|                                                   | 1                | 1.4142       | 1.5979       | 12.99                       | 1.2970       | 1.3740       | 5.94                        |
|                                                   | 2                | 1.3303       | 1.6365       | 23.02                       | 1.2633       | 1.3917       | 10.16                       |
|                                                   | 3                | 1.2464       | 1.6751       | 34.39                       | 1.2296       | 1.4094       | 14.62                       |
|                                                   | $1 \leftarrow 0$ | -0.0839      | 0.0386       | -145.97                     | -0.0337      | 0.0177       | -152.43                     |
| $\nu_{10}$                                        | 0                | 1.5486       | 1.5460       | -0.17                       | 1.3558       | 1.3355       | -1.50                       |
|                                                   | 1                | 1.5657       | 1.5577       | -0.51                       | 1.3722       | 1.3113       | -4.44                       |
|                                                   | 2                | 1.5828       | 1.5694       | -0.84                       | 1.3886       | 1.2871       | -7.30                       |
|                                                   | 3                | 1.5998       | 1.5812       | -1.17                       | 1.4050       | 1.2630       | -10.11                      |
|                                                   | $1 \leftarrow 0$ | 0.0171       | 0.0117       | -31.22                      | 0.0164       | -0.0242      | -247.27                     |

<sup>c</sup> 2D effects = (Perturbed 2D-Perturbed 1D)/Perturbed 1D

**Table S25:** Anharmonic potential parameters  $\frac{\sqrt{h^3 c^3 \phi_j^2 \omega_j / E_h}}{N} \frac{\partial^3 V_{\text{ReO}}}{\partial q_i^2 \partial q_j}$  (where  $N = 2$  for  $i \neq j$  and  $N = 6$  for  $i = j$ ) for  $\text{Cp}^{187}\text{Re}(\text{CH}_3)(\text{CO})(\text{NO})$ . B3LYP/cc-pV5Z,cc-pwCVQZ-PP level harmonic force field was utilised for the anharmonic calculation at B3LYP level with (12s11p10d8f)[8s7p6d4f] contraction on Re atom and cc-pVDZ basis set for H, C, N and O atoms. Values are determined by the GAUSSIAN package.

| Mode            | VBO           |               |               |               |               |               |               |               |               |               |
|-----------------|---------------|---------------|---------------|---------------|---------------|---------------|---------------|---------------|---------------|---------------|
| V <sub>51</sub> | 0.602536E-12  | 0.932663E-11  | -0.364564E-10 | -0.204726E-10 | 0.960085E-11  | -0.130801E-10 | -0.435774E-10 | 0.112920E-09  | -0.292662E-09 | -0.292662E-09 |
|                 | -0.417420E-09 | 0.184705E-10  | 0.307491E-09  | -0.546888E-10 | -0.136714E-10 | 0.578607E-10  | -0.247228E-09 | 0.110329E-09  | -0.241626E-09 | -0.241626E-09 |
|                 | 0.136824E-09  | 0.257539E-09  | 0.690905E-11  | 0.188861E-09  | 0.670327E-12  | 0.266487E-09  | 0.335971E-10  | -0.867133E-10 | 0.153377E-09  | 0.153377E-09  |
|                 | 0.447041E-09  | -0.269975E-09 | 0.883111E-09  | -0.145755E-08 | 0.999396E-10  | -0.111667E-07 | -0.126589E-09 | 0.241407E-10  | -0.700580E-09 | -0.700580E-09 |
| V <sub>50</sub> | 0.265178E-09  | -0.797823E-10 | 0.382842E-09  | -0.430715E-09 | -0.363604E-10 | 0.488220E-09  | -0.159990E-08 | 0.412323E-08  | 0.507770E-09  | 0.507770E-09  |
|                 | 0.135669E-08  | -0.213158E-08 | 0.185174E-08  | -0.250535E-08 | 0.613839E-09  | 0.174258E-07  |               |               |               |               |
|                 | 0.221649E-10  | 0.123581E-10  | -0.179840E-10 | 0.298315E-11  | 0.130945E-10  | -0.170648E-11 | -0.203471E-10 | -0.195202E-09 | -0.132978E-09 | -0.132978E-09 |
|                 | 0.491458E-10  | 0.121681E-09  | 0.483011E-09  | -0.859935E-10 | 0.107976E-09  | 0.421369E-10  | -0.757076E-09 | 0.634534E-09  | -0.128168E-08 | -0.128168E-08 |
| V <sub>49</sub> | 0.107649E-08  | 0.131168E-09  | 0.841238E-10  | 0.123696E-09  | 0.257429E-09  | -0.106959E-09 | -0.217379E-09 | -0.662862E-09 | 0.151628E-09  | 0.151628E-09  |
|                 | -0.344543E-12 | -0.507179E-10 | 0.537508E-10  | 0.592330E-09  | 0.381198E-09  | -0.164602E-08 | -0.653246E-10 | 0.437922E-10  | -0.296564E-09 | -0.296564E-09 |
|                 | 0.343312E-09  | -0.100019E-09 | 0.351214E-10  | -0.138015E-09 | -0.104291E-09 | 0.899246E-08  | -0.489579E-08 | 0.101996E-08  | 0.192288E-09  | 0.192288E-09  |
|                 | -0.115399E-09 | -0.693138E-09 | 0.232407E-08  | -0.459529E-09 | 0.158437E-09  | 0.232556E-08  |               |               |               |               |
| V <sub>48</sub> | -0.121645E-11 | 0.290421E-10  | -0.138222E-11 | -0.765382E-11 | 0.170876E-10  | -0.238588E-10 | -0.222291E-10 | -0.156146E-09 | -0.428421E-10 | -0.428421E-10 |
|                 | -0.260387E-10 | 0.800064E-10  | 0.118535E-08  | -0.594439E-09 | 0.210605E-09  | -0.145626E-09 | -0.379145E-09 | 0.109544E-09  | -0.701007E-09 | -0.701007E-09 |
|                 | 0.104408E-08  | 0.135093E-09  | -0.486363E-10 | 0.172515E-09  | 0.124914E-10  | 0.218272E-09  | 0.170780E-09  | 0.204224E-09  | -0.818112E-10 | -0.818112E-10 |
|                 | 0.242991E-10  | 0.495308E-10  | 0.104999E-09  | -0.459767E-09 | -0.371088E-09 | -0.921421E-09 | -0.173134E-09 | -0.460436E-11 | -0.132028E-09 | -0.132028E-09 |
| V <sub>47</sub> | -0.156665E-09 | 0.281330E-11  | -0.543351E-11 | 0.513204E-10  | 0.573289E-10  | 0.384253E-08  | -0.168193E-07 | 0.345879E-09  | -0.316836E-10 | -0.316836E-10 |
|                 | 0.116604E-09  | 0.284603E-09  | -0.101897E-08 | -0.386470E-09 | -0.955854E-10 | 0.177503E-08  |               |               |               |               |
|                 | 0.291392E-11  | 0.788575E-11  | 0.250430E-10  | -0.160458E-10 | 0.773331E-11  | -0.118082E-10 | -0.264608E-10 | -0.160103E-09 | -0.416641E-10 | -0.416641E-10 |
|                 | 0.698488E-11  | 0.664241E-10  | 0.934880E-09  | -0.431310E-09 | 0.222636E-09  | -0.164249E-09 | -0.646040E-09 | 0.413798E-09  | -0.112169E-08 | -0.112169E-08 |
| V <sub>46</sub> | 0.152845E-08  | 0.289320E-09  | -0.73261E-11  | 0.104263E-09  | 0.112120E-09  | 0.126796E-09  | 0.297457E-10  | 0.202437E-09  | -0.353798E-10 | -0.353798E-10 |
|                 | 0.837983E-11  | 0.233342E-10  | 0.566923E-10  | -0.368439E-09 | -0.133176E-09 | -0.621964E-09 | -0.152575E-09 | -0.321180E-11 | -0.112763E-09 | -0.112763E-09 |
|                 | -0.389825E-10 | -0.418371E-10 | 0.113128E-10  | 0.548702E-10  | 0.140911E-10  | 0.824429E-08  | -0.144309E-07 | 0.505747E-09  | -0.775361E-10 | -0.775361E-10 |
|                 | 0.368269E-09  | -0.639926E-10 | -0.753391E-09 | -0.135949E-09 | 0.606962E-11  | 0.110389E-08  |               |               |               |               |
| V <sub>45</sub> | -0.195481E-10 | 0.100282E-10  | -0.342189E-11 | 0.492132E-11  | 0.200296E-10  | 0.574830E-11  | -0.252802E-10 | -0.318023E-12 | -0.408732E-10 | -0.408732E-10 |
|                 | -0.174914E-10 | 0.388128E-09  | 0.108311E-08  | 0.117602E-08  | -0.189645E-09 | 0.389678E-09  | -0.250214E-09 | 0.246308E-09  | -0.428011E-09 | -0.428011E-09 |
|                 | 0.246103E-09  | -0.529103E-09 | 0.756668E-09  | 0.111618E-09  | 0.330855E-09  | 0.854409E-10  | 0.162708E-09  | -0.598599E-09 | 0.137045E-10  | 0.137045E-10  |
|                 | 0.280731E-09  | 0.241510E-10  | 0.146256E-09  | 0.383392E-09  | -0.656170E-10 | -0.116571E-08 | 0.946955E-09  | -0.239109E-10 | 0.260924E-10  | 0.260924E-10  |
| V <sub>44</sub> | -0.268313E-11 | -0.585999E-10 | -0.914194E-10 | -0.122975E-08 | 0.136213E-09  | 0.406664E-08  | -0.652689E-08 | 0.281565E-07  | 0.916961E-09  | 0.916961E-09  |
|                 | -0.130712E-07 | 0.403104E-09  | 0.121373E-08  | -0.385380E-09 | 0.126657E-09  | 0.173354E-08  |               |               |               |               |
|                 | -0.189565E-09 | 0.142301E-10  | 0.259506E-09  | 0.242133E-09  | 0.197902E-09  | -0.816977E-09 | -0.748648E-09 | 0.202603E-09  | 0.108259E-08  | 0.108259E-08  |
|                 | 0.137661E-09  | -0.289979E-09 | -0.123993E-08 | -0.191424E-08 | 0.780728E-09  | -0.235192E-09 | -0.118963E-09 | -0.679720E-09 | -0.484978E-09 | -0.484978E-09 |
| V <sub>43</sub> | -0.886893E-09 | 0.403889E-08  | 0.444735E-08  | -0.514271E-09 | 0.203449E-08  | 0.846577E-09  | 0.673614E-09  | 0.408894E-09  | -0.366851E-09 | -0.366851E-09 |
|                 | 0.340960E-09  | -0.135760E-09 | -0.591457E-09 | -0.249867E-10 | -0.851635E-09 | -0.552690E-09 | -0.273018E-07 | -0.149441E-09 | -0.495115E-09 | -0.495115E-09 |
|                 | -0.582736E-09 | 0.966823E-11  | 0.133739E-09  | -0.442721E-09 | -0.213290E-08 | -0.146417E-08 | 0.591061E-09  | 0.478480E-06  | 0.239921E-07  | 0.239921E-07  |
|                 | 0.106220E-06  | -0.286382E-09 | -0.108346E-08 | 0.813657E-10  | 0.813657E-09  | 0.109278E-08  |               |               |               |               |
| V <sub>42</sub> | 0.414604E-10  | 0.262448E-09  | 0.225023E-09  | 0.134262E-09  | -0.178352E-09 | 0.858086E-09  | -0.100060E-08 | 0.371062E-09  | 0.845490E-09  | 0.845490E-09  |
|                 | 0.371476E-09  | 0.459778E-10  | -0.478209E-09 | -0.494868E-09 | 0.181631E-09  | -0.315299E-09 | 0.177488E-09  | -0.669907E-09 | -0.570807E-09 | -0.570807E-09 |
|                 | -0.187690E-09 | 0.125065E-10  | -0.286321E-08 | 0.704029E-09  | -0.667266E-09 | 0.278753E-09  | -0.573376E-09 | 0.284156E-09  | 0.166540E-09  | 0.166540E-09  |
|                 | 0.861249E-09  | 0.200651E-09  | -0.181199E-09 | -0.147983E-09 | 0.773908E-09  | -0.574622E-09 | -0.904597E-08 | 0.192056E-09  | 0.302609E-11  | 0.302609E-11  |
| V <sub>41</sub> | 0.272359E-09  | 0.935560E-10  | 0.358882E-09  | 0.157344E-08  | 0.628770E-08  | 0.377944E-09  | -0.716207E-10 | 0.182005E-06  | 0.585004E-07  | 0.585004E-07  |
|                 | 0.520671E-07  | -0.724129E-09 | -0.117003E-08 | 0.304822E-09  | 0.700990E-09  | 0.158501E-08  |               |               |               |               |
|                 | 0.261620E-10  | -0.112622E-09 | -0.232801E-09 | 0.120292E-09  | 0.113280E-10  | -0.186647E-09 | -0.176480E-09 | 0.179921E-08  | -0.228925E-09 | -0.228925E-09 |
|                 | 0.786767E-09  | -0.209531E-09 | -0.641839E-09 | 0.496860E-10  | -0.160842E-09 | 0.314642E-09  | -0.868131E-10 | -0.442542E-09 | 0.307975E-09  | 0.307975E-09  |
| V <sub>40</sub> | 0.406160E-09  | -0.989356E-10 | -0.106214E-09 | -0.921533E-09 | -0.429478E-10 | -0.482020E-09 | -0.185785E-09 | 0.135271E-09  | -0.715113E-09 | -0.715113E-09 |
|                 | -0.165716E-09 | -0.783242E-10 | -0.920664E-09 | 0.450298E-09  | 0.571500E-10  | 0.368646E-08  | 0.355311E-09  | -0.296826E-11 | 0.205638E-09  | 0.205638E-09  |
|                 | -0.290083E-09 | -0.461736E-10 | 0.486184E-09  | 0.736668E-10  | 0.770064E-11  | 0.193629E-08  | -0.285768E-08 | 0.130394E-08  | 0.115540E-10  | 0.115540E-10  |
|                 | 0.104311E-08  | -0.664628E-09 | 0.310944E-09  | -0.949557E-09 | 0.807421E-09  | 0.249280E-08  |               |               |               |               |

**Table S25:** Anharmonic potential parameters  $\frac{\sqrt{h^3 c^3 \phi_i^2 \phi_j / E_h}}{N} \frac{\partial^3 V_{\text{BO}}}{\partial q_i^2 \partial q_j}$  (where  $N = 2$  for  $i \neq j$  and  $N = 6$  for  $i = j$ ) for  $\text{Cp}^{187}\text{Re}(\text{CH}_3)(\text{CO})(\text{NO})$ . B3LYP/cc-pV5Z,cc-pwCVQZ-PP level harmonic force field was utilised for the anharmonic calculation at B3LYP level with (12s11p10d8f)[8s7p6d4f] contraction on Re atom and cc-pVDZ basis set for H, C, N and O atoms. Values are determined by the GAUSSIAN package. (continued).

| Mode            | VBO           |               |               |               |               |               |               |               |               |               |
|-----------------|---------------|---------------|---------------|---------------|---------------|---------------|---------------|---------------|---------------|---------------|
| V <sub>43</sub> | -0.716001E-10 | 0.824890E-10  | -0.800499E-10 | 0.978647E-10  | 0.208565E-09  | -0.278202E-09 | -0.384394E-09 | 0.649137E-08  | -0.125410E-09 | -0.118043E-08 |
|                 | -0.925205E-09 | 0.506702E-10  | -0.812395E-09 | 0.566080E-09  | -0.317977E-09 | -0.123094E-08 | -0.215928E-08 | -0.429252E-08 | -0.118043E-08 | -0.118043E-08 |
|                 | -0.517008E-09 | 0.541919E-09  | -0.222232E-09 | 0.256144E-08  | 0.133282E-08  | -0.100898E-08 | -0.116225E-08 | 0.158577E-08  | 0.913745E-09  | 0.913745E-09  |
|                 | 0.272862E-08  | -0.389562E-09 | 0.284928E-09  | -0.471302E-08 | 0.431494E-08  | -0.660420E-08 | 0.118727E-09  | 0.584680E-10  | 0.327141E-08  | 0.327141E-08  |
| V <sub>42</sub> | 0.201032E-08  | -0.626067E-09 | 0.177393E-08  | 0.207677E-10  | 0.897899E-10  | 0.142712E-08  | -0.211511E-08 | 0.423874E-09  | -0.495800E-09 | -0.495800E-09 |
|                 | 0.113489E-09  | -0.942689E-08 | -0.335997E-08 | 0.186183E-08  | 0.405892E-08  | 0.962318E-08  |               |               |               |               |
|                 | 0.136654E-09  | -0.223529E-10 | -0.193921E-09 | 0.750000E-10  | 0.145039E-09  | 0.639029E-10  | -0.169995E-09 | 0.720836E-08  | 0.143748E-09  | 0.143748E-09  |
|                 | -0.644956E-09 | -0.391102E-09 | -0.708061E-10 | -0.452273E-09 | 0.450718E-09  | 0.109794E-08  | 0.255327E-08  | 0.318304E-08  | 0.903546E-09  | 0.903546E-09  |
| V <sub>41</sub> | 0.514584E-09  | 0.701282E-09  | -0.278130E-09 | 0.587281E-09  | 0.384702E-10  | 0.130005E-08  | -0.121242E-08 | -0.224660E-08 | -0.140662E-08 | -0.140662E-08 |
|                 | -0.104922E-08 | 0.115500E-08  | -0.641103E-09 | 0.288528E-08  | -0.390283E-08 | -0.712048E-08 | 0.245740E-09  | 0.653373E-10  | -0.471506E-08 | -0.471506E-08 |
|                 | -0.243413E-08 | -0.133403E-09 | 0.106639E-08  | -0.758465E-09 | -0.115212E-09 | 0.108714E-08  | -0.175320E-08 | 0.267858E-08  | 0.561289E-09  | 0.561289E-09  |
|                 | 0.570720E-09  | 0.572154E-08  | 0.542949E-08  | -0.356168E-08 | 0.145103E-08  | 0.801672E-08  |               |               |               |               |
| V <sub>40</sub> | -0.982930E-10 | 0.921521E-10  | 0.450822E-09  | -0.120830E-09 | -0.139578E-09 | -0.320291E-09 | -0.175708E-09 | -0.142341E-10 | -0.742847E-10 | -0.742847E-10 |
|                 | -0.117379E-08 | -0.442748E-09 | 0.375956E-08  | -0.401005E-08 | 0.119519E-08  | -0.684489E-08 | -0.194249E-08 | 0.120361E-08  | -0.122472E-08 | -0.122472E-08 |
|                 | 0.507706E-08  | 0.730397E-09  | 0.326740E-09  | 0.342556E-09  | 0.560420E-09  | 0.398879E-09  | 0.343727E-09  | 0.285549E-09  | -0.856846E-10 | -0.856846E-10 |
|                 | 0.252950E-09  | 0.188653E-09  | -0.196414E-09 | 0.189463E-09  | 0.517326E-10  | 0.471289E-09  | -0.491001E-09 | 0.157294E-10  | 0.351365E-09  | 0.351365E-09  |
| V <sub>39</sub> | -0.108347E-09 | -0.407081E-10 | -0.107655E-09 | -0.670607E-09 | 0.589261E-09  | 0.126097E-07  | -0.978032E-07 | 0.574088E-08  | 0.773891E-09  | 0.773891E-09  |
|                 | -0.722758E-09 | -0.658375E-10 | 0.152504E-08  | -0.468831E-09 | 0.661176E-09  | 0.144897E-08  |               |               |               |               |
|                 | -0.155758E-09 | 0.153531E-09  | 0.407363E-09  | -0.242557E-09 | 0.713747E-09  | 0.210604E-09  | 0.140969E-09  | -0.140324E-08 | 0.518812E-09  | 0.518812E-09  |
|                 | -0.940045E-09 | -0.309997E-08 | -0.778126E-08 | 0.307475E-08  | -0.325498E-08 | 0.303853E-09  | -0.122010E-08 | 0.330528E-08  | -0.143222E-08 | -0.143222E-08 |
| V <sub>38</sub> | -0.298695E-08 | -0.498866E-09 | 0.130616E-08  | -0.937459E-09 | 0.120317E-08  | 0.568243E-09  | -0.436137E-10 | 0.285469E-09  | -0.312005E-10 | -0.312005E-10 |
|                 | 0.163220E-09  | 0.228025E-09  | 0.135329E-09  | -0.188953E-09 | -0.263863E-10 | -0.137880E-09 | 0.183105E-08  | 0.904869E-11  | 0.457335E-10  | 0.457335E-10  |
|                 | -0.223949E-09 | 0.172729E-09  | -0.461022E-11 | 0.208246E-09  | -0.434701E-09 | 0.190602E-08  | -0.220969E-07 | 0.101877E-08  | 0.327313E-09  | 0.327313E-09  |
|                 | 0.116736E-08  | -0.177598E-09 | 0.600463E-10  | -0.351130E-09 | 0.387522E-10  | 0.318628E-09  |               |               |               |               |
| V <sub>37</sub> | -0.772265E-10 | 0.617710E-10  | 0.470182E-09  | -0.482355E-09 | -0.327237E-09 | -0.272739E-09 | 0.281164E-09  | -0.121394E-08 | 0.218039E-10  | 0.218039E-10  |
|                 | -0.867671E-09 | -0.434740E-08 | -0.185991E-07 | -0.644266E-08 | 0.186908E-08  | -0.223584E-08 | -0.548407E-09 | 0.478472E-09  | -0.976399E-09 | -0.976399E-09 |
|                 | -0.208377E-09 | -0.123814E-08 | 0.386775E-09  | -0.259462E-09 | -0.184606E-09 | 0.382013E-09  | -0.610071E-09 | 0.346816E-10  | -0.443821E-09 | -0.443821E-09 |
|                 | 0.428453E-09  | 0.963027E-10  | 0.136880E-09  | 0.132972E-09  | -0.750384E-10 | 0.219751E-10  | 0.619950E-08  | -0.149046E-10 | -0.556080E-09 | -0.556080E-09 |
| V <sub>36</sub> | -0.101673E-09 | 0.187674E-09  | 0.108530E-09  | 0.783119E-09  | -0.608360E-09 | -0.870337E-09 | -0.162762E-07 | 0.240869E-08  | 0.230026E-09  | 0.230026E-09  |
|                 | 0.148330E-08  | 0.132256E-09  | 0.995212E-10  | -0.112940E-09 | 0.119646E-10  | 0.182643E-09  |               |               |               |               |
|                 | -0.195354E-09 | -0.234650E-09 | -0.258363E-09 | 0.249148E-09  | 0.406976E-09  | 0.667921E-09  | 0.185573E-09  | -0.201770E-10 | 0.958141E-09  | 0.958141E-09  |
|                 | -0.514825E-09 | -0.172695E-08 | 0.106272E-08  | -0.217713E-08 | 0.118063E-08  | 0.204229E-08  | -0.148222E-08 | 0.851984E-09  | -0.204580E-08 | -0.204580E-08 |
| V <sub>35</sub> | 0.218936E-08  | 0.250530E-09  | -0.543472E-10 | 0.258034E-09  | 0.727065E-09  | -0.267330E-10 | 0.644962E-09  | 0.307839E-09  | -0.445139E-09 | -0.445139E-09 |
|                 | 0.257036E-10  | 0.452325E-09  | -0.696499E-10 | -0.170419E-09 | -0.257054E-09 | 0.406454E-09  | -0.398866E-09 | 0.404826E-10  | -0.292920E-09 | -0.292920E-09 |
|                 | -0.484767E-09 | 0.224942E-09  | 0.325384E-10  | -0.929279E-09 | -0.266625E-09 | 0.600776E-08  | -0.103209E-06 | 0.117940E-07  | -0.637273E-09 | -0.637273E-09 |
|                 | 0.421043E-10  | -0.168363E-09 | 0.340396E-09  | 0.424065E-09  | 0.283251E-09  | 0.817396E-10  |               |               |               |               |
| V <sub>34</sub> | -0.402718E-09 | 0.199304E-09  | 0.354703E-09  | 0.185912E-09  | 0.276336E-10  | 0.463672E-09  | 0.842584E-09  | 0.179297E-08  | 0.244684E-08  | 0.244684E-08  |
|                 | -0.253519E-10 | -0.913202E-09 | 0.127310E-08  | -0.261190E-08 | -0.138225E-08 | 0.422569E-09  | -0.230930E-08 | 0.173531E-08  | -0.140099E-08 | -0.140099E-08 |
|                 | 0.336666E-08  | 0.187189E-08  | 0.102047E-09  | 0.801580E-10  | 0.876946E-10  | -0.383103E-09 | 0.100265E-08  | 0.747301E-09  | -0.797884E-09 | -0.797884E-09 |
|                 | 0.132374E-08  | -0.242565E-09 | -0.434158E-09 | -0.151617E-08 | -0.220100E-09 | -0.107923E-08 | -0.155220E-09 | -0.498432E-10 | 0.758994E-09  | 0.758994E-09  |
| V <sub>33</sub> | -0.100260E-08 | 0.709783E-09  | 0.140725E-08  | -0.104153E-09 | -0.143726E-08 | 0.344690E-07  | -0.525339E-07 | 0.511591E-08  | 0.198021E-08  | 0.198021E-08  |
|                 | 0.497637E-08  | 0.234441E-09  | 0.141264E-08  | -0.185317E-08 | -0.126107E-08 | 0.239006E-08  |               |               |               |               |
|                 | 0.2323230E-10 | 0.235851E-09  | 0.178635E-09  | -0.335918E-09 | 0.489083E-11  | 0.306437E-09  | 0.638255E-09  | 0.231047E-08  | -0.176040E-08 | -0.176040E-08 |
|                 | -0.106744E-08 | -0.100048E-08 | -0.689193E-09 | 0.267695E-09  | 0.121875E-08  | -0.169689E-08 | 0.144806E-08  | -0.196486E-08 | 0.318058E-08  | 0.318058E-08  |
| V <sub>32</sub> | -0.460881E-08 | 0.710597E-09  | -0.130211E-08 | 0.569393E-08  | 0.240844E-08  | -0.296600E-09 | 0.396100E-09  | -0.907448E-09 | 0.313869E-09  | 0.313869E-09  |
|                 | 0.173400E-09  | -0.385289E-09 | 0.428414E-08  | 0.705449E-09  | -0.940753E-10 | -0.779995E-08 | 0.692661E-11  | 0.323076E-09  | -0.242450E-08 | -0.242450E-08 |
|                 | 0.161093E-08  | 0.200041E-10  | -0.124657E-07 | 0.603925E-09  | 0.225314E-09  | 0.109492E-07  | -0.426380E-08 | 0.144484E-08  | 0.465912E-09  | 0.465912E-09  |
|                 | -0.530576E-09 | -0.243751E-08 | -0.248741E-08 | -0.292615E-08 | -0.119877E-08 | 0.228030E-09  |               |               |               |               |

**Table S25:** Anharmonic potential parameters  $\frac{\sqrt{h^3 c^3 \omega_j^2 \omega_l / E_h}}{N} \frac{\partial^3 V_{\text{ReO}}}{\partial q_i^2 \partial q_j}$  (where  $N = 2$  for  $i \neq j$  and  $N = 6$  for  $i = j$ ) for  $\text{Cp}^{187}\text{Re}(\text{CH}_3)(\text{CO})(\text{NO})$ . B3LYP/cc-pV5Z,cc-pwCVQZ-PP level harmonic force field was utilised for the anharmonic calculation at B3LYP level with (12s11p10d8f)[8s7p6d4f] contraction on Re atom and cc-pVDZ basis set for H, C, N and O atoms. Values are determined by the GAUSSIAN package. (continued).

| Mode            | VBO           |               |               |               |               |               |               |               |               |  |
|-----------------|---------------|---------------|---------------|---------------|---------------|---------------|---------------|---------------|---------------|--|
| V <sub>35</sub> | 0.930056E-10  | 0.657217E-09  | 0.654874E-09  | -0.218648E-09 | -0.200651E-09 | -0.224957E-09 | 0.146137E-10  | 0.221417E-08  | -0.280706E-09 |  |
|                 | 0.142501E-08  | -0.207801E-08 | -0.124068E-08 | 0.909925E-09  | 0.828168E-09  | -0.435504E-09 | 0.698704E-09  | -0.777218E-09 | 0.208374E-08  |  |
|                 | -0.284167E-08 | 0.264524E-09  | -0.816543E-10 | 0.455307E-08  | 0.148484E-08  | 0.146491E-08  | 0.132219E-08  | -0.681691E-09 | 0.135115E-08  |  |
|                 | 0.198779E-08  | 0.245791E-08  | -0.153528E-08 | -0.541887E-09 | 0.990239E-08  | -0.666995E-08 | -0.169594E-09 | -0.107029E-09 | -0.295448E-08 |  |
| V <sub>34</sub> | -0.330480E-09 | -0.678812E-08 | 0.787844E-08  | -0.265973E-09 | -0.223950E-09 | 0.159379E-07  | -0.112126E-07 | 0.774993E-09  | 0.298841E-09  |  |
|                 | 0.718675E-09  | 0.900337E-09  | -0.318785E-08 | 0.909872E-09  | 0.413938E-08  | 0.337424E-08  |               |               |               |  |
|                 | 0.192310E-09  | 0.450665E-09  | 0.345516E-09  | -0.104009E-08 | 0.433223E-09  | 0.830125E-10  | 0.196297E-09  | 0.102380E-08  | 0.112086E-08  |  |
|                 | -0.154854E-09 | -0.239325E-08 | 0.380781E-09  | -0.420875E-09 | 0.158355E-10  | 0.464361E-09  | 0.464826E-08  | -0.439483E-08 | 0.356828E-08  |  |
| V <sub>33</sub> | -0.100837E-07 | -0.117245E-08 | -0.341182E-09 | 0.444401E-08  | 0.282001E-09  | 0.690053E-09  | 0.734354E-09  | 0.236684E-09  | -0.772903E-09 |  |
|                 | 0.170985E-08  | -0.216440E-08 | -0.136897E-08 | -0.877169E-09 | -0.130303E-08 | -0.500000E-08 | -0.121707E-09 | -0.138442E-09 | -0.911446E-09 |  |
|                 | 0.105003E-09  | 0.726766E-08  | 0.439717E-08  | -0.293835E-09 | -0.539460E-09 | 0.205128E-07  | -0.898416E-08 | 0.374442E-08  | 0.176223E-08  |  |
|                 | 0.214428E-09  | -0.187818E-08 | 0.407672E-08  | 0.547438E-08  | 0.136467E-08  | 0.308629E-08  |               |               |               |  |
| V <sub>32</sub> | -0.510191E-10 | -0.117909E-08 | -0.680567E-09 | 0.120993E-08  | -0.879376E-09 | 0.175473E-09  | 0.718285E-10  | -0.196691E-08 | 0.380927E-09  |  |
|                 | -0.343678E-09 | 0.264006E-08  | -0.390788E-08 | -0.126587E-08 | -0.132284E-08 | -0.193857E-09 | 0.733699E-08  | -0.734766E-08 | 0.110476E-07  |  |
|                 | -0.162855E-08 | -0.136214E-08 | 0.423059E-10  | 0.131874E-08  | -0.490419E-09 | -0.326990E-09 | 0.420945E-09  | -0.424589E-09 | 0.133895E-09  |  |
|                 | -0.375729E-09 | 0.167986E-09  | -0.444674E-09 | 0.796893E-09  | 0.772789E-10  | -0.645637E-10 | -0.733552E-09 | 0.105549E-09  | -0.138122E-08 |  |
| V <sub>31</sub> | 0.114035E-08  | -0.241818E-09 | 0.459252E-09  | 0.812489E-09  | -0.859892E-09 | 0.456773E-07  | -0.281569E-07 | 0.641699E-08  | 0.343006E-08  |  |
|                 | 0.367967E-08  | -0.592383E-10 | 0.146438E-08  | 0.197368E-08  | -0.726031E-09 | 0.216243E-08  |               |               |               |  |
|                 | -0.281722E-09 | 0.727252E-09  | 0.154772E-08  | 0.119691E-08  | 0.450161E-09  | 0.219714E-08  | -0.908001E-09 | -0.319987E-09 | 0.199584E-08  |  |
|                 | 0.470661E-09  | -0.196423E-08 | -0.615143E-08 | -0.970171E-08 | 0.146038E-08  | 0.496057E-08  | 0.181460E-08  | -0.303504E-08 | -0.467205E-09 |  |
| V <sub>30</sub> | -0.747841E-09 | 0.210028E-08  | -0.72679E-08  | -0.178054E-08 | 0.658120E-09  | -0.712187E-09 | 0.124560E-08  | 0.652177E-09  | 0.776609E-10  |  |
|                 | -0.141033E-08 | 0.100354E-09  | -0.604851E-09 | 0.112316E-09  | -0.245446E-10 | -0.617728E-09 | -0.105000E-07 | -0.283777E-09 | -0.412337E-09 |  |
|                 | 0.200124E-08  | -0.727036E-09 | 0.171480E-08  | 0.302185E-07  | 0.619945E-07  | 0.219768E-08  | -0.280914E-08 | 0.503279E-06  | 0.282049E-06  |  |
|                 | 0.192879E-06  | -0.203425E-08 | 0.527200E-08  | -0.162426E-07 | 0.933391E-08  | 0.164465E-07  |               |               |               |  |
| V <sub>29</sub> | -0.764958E-10 | 0.131294E-09  | 0.794074E-09  | 0.673260E-09  | 0.201538E-09  | -0.844620E-09 | 0.276727E-09  | -0.497363E-09 | 0.138814E-08  |  |
|                 | 0.908017E-09  | -0.295294E-08 | -0.780919E-08 | -0.131118E-07 | 0.314290E-08  | 0.164057E-08  | 0.645172E-09  | -0.309401E-09 | -0.143585E-08 |  |
|                 | -0.550553E-09 | -0.568515E-09 | -0.241501E-08 | -0.476854E-10 | -0.170834E-08 | -0.140796E-08 | -0.459248E-09 | 0.739212E-09  | 0.222756E-10  |  |
|                 | -0.103363E-08 | -0.561124E-09 | -0.444481E-09 | -0.363206E-09 | 0.604371E-09  | 0.562858E-09  | -0.581972E-08 | 0.346731E-09  | -0.246143E-08 |  |
| V <sub>28</sub> | -0.194064E-08 | 0.696041E-09  | -0.211635E-09 | -0.169165E-07 | 0.538206E-07  | 0.216356E-08  | -0.207695E-08 | 0.526562E-06  | -0.197475E-06 |  |
|                 | 0.620245E-07  | 0.293287E-07  | 0.286326E-07  | 0.412790E-09  | -0.209088E-07 | 0.612143E-07  |               |               |               |  |
|                 | -0.625851E-09 | -0.358258E-09 | 0.948020E-10  | 0.368418E-09  | -0.461153E-10 | 0.367670E-10  | -0.521097E-09 | 0.117305E-08  | 0.898391E-09  |  |
|                 | -0.878028E-09 | -0.182834E-08 | 0.580012E-09  | 0.217775E-09  | 0.175027E-08  | 0.229979E-08  | -0.435380E-09 | -0.131757E-09 | -0.705147E-09 |  |
| V <sub>27</sub> | -0.108089E-08 | 0.109210E-08  | -0.365410E-09 | -0.15964E-08  | 0.187142E-08  | -0.186439E-08 | -0.225120E-08 | 0.350730E-08  | -0.238067E-08 |  |
|                 | -0.314229E-08 | 0.722072E-09  | -0.101941E-09 | 0.700776E-10  | -0.682971E-09 | -0.421837E-08 | -0.108285E-09 | -0.479757E-09 | -0.840072E-08 |  |
|                 | -0.309311E-08 | 0.192425E-08  | -0.105868E-08 | -0.646802E-09 | -0.214971E-08 | 0.357733E-08  | -0.217034E-08 | 0.181538E-07  | 0.100902E-07  |  |
|                 | -0.935652E-09 | 0.171360E-06  | 0.180024E-06  | -0.439705E-06 | 0.191351E-06  | 0.452302E-06  |               |               |               |  |
| V <sub>26</sub> | 0.395229E-10  | 0.370444E-09  | -0.320480E-09 | 0.761699E-10  | 0.677618E-09  | -0.277389E-09 | -0.404258E-09 | 0.644076E-09  | 0.119569E-09  |  |
|                 | -0.257229E-09 | 0.544912E-09  | -0.854916E-09 | -0.149710E-08 | -0.777787E-09 | 0.360694E-08  | 0.127245E-08  | 0.283283E-08  | 0.125971E-08  |  |
|                 | 0.162057E-08  | -0.115810E-10 | -0.137100E-08 | -0.385007E-09 | 0.490846E-09  | 0.379326E-10  | 0.195111E-09  | 0.109130E-08  | 0.981420E-09  |  |
|                 | -0.749088E-09 | -0.187360E-08 | 0.213624E-08  | -0.212551E-08 | 0.283769E-08  | 0.267576E-08  | -0.548685E-09 | 0.475390E-09  | -0.136461E-07 |  |
| V <sub>25</sub> | 0.158232E-08  | -0.399538E-09 | -0.950517E-09 | -0.476502E-08 | 0.476258E-08  | 0.153567E-08  | -0.439351E-08 | 0.619105E-07  | -0.158661E-07 |  |
|                 | -0.303640E-09 | 0.154137E-06  | 0.298371E-06  | 0.147100E-06  | -0.165553E-06 | 0.466210E-06  |               |               |               |  |
|                 | 0.299447E-09  | 0.235131E-09  | -0.221243E-10 | 0.963932E-10  | 0.112733E-09  | -0.376225E-09 | -0.718184E-09 | 0.521898E-09  | 0.748049E-09  |  |
|                 | 0.951969E-09  | 0.102861E-08  | -0.133172E-08 | 0.697805E-09  | 0.742743E-10  | -0.761880E-09 | -0.281723E-08 | -0.372552E-08 | -0.770579E-10 |  |
| V <sub>24</sub> | 0.785290E-09  | -0.933479E-10 | -0.385668E-09 | 0.175150E-08  | -0.144415E-08 | -0.749189E-10 | -0.118630E-08 | 0.192698E-08  | -0.359853E-08 |  |
|                 | -0.364858E-08 | 0.379167E-08  | -0.375697E-08 | 0.775021E-08  | -0.298433E-08 | 0.636320E-08  | 0.274762E-09  | 0.262482E-09  | 0.914656E-09  |  |
|                 | 0.311937E-08  | 0.165918E-08  | 0.970763E-09  | -0.331821E-09 | -0.465722E-09 | 0.547341E-09  | -0.370623E-08 | 0.500066E-08  | -0.186233E-08 |  |
|                 | -0.239498E-09 | -0.574703E-07 | 0.508367E-07  | 0.115439E-06  | -0.335112E-08 | 0.317815E-06  |               |               |               |  |

**Table S25:** Anharmonic potential parameters  $\frac{\sqrt{h^3 c^3 \phi_j^2 \omega_j / E_h}}{N} \frac{\partial^3 V_{\text{ReO}}}{\partial q_i^2 \partial q_j}$  (where  $N = 2$  for  $i \neq j$  and  $N = 6$  for  $i = j$ ) for  $\text{Cp}^{187}\text{Re}(\text{CH}_3)(\text{CO})(\text{NO})$ . B3LYP/cc-pV5Z,cc-pwCVQZ-PP level harmonic force field was utilised for the anharmonic calculation at B3LYP level with (12s11p10d8f)[8s7p6d4f] contraction on Re atom and cc-pVDZ basis set for H, C, N and O atoms. Values are determined by the GAUSSIAN package. (continued).

| Mode            | VBO           |               |               |               |               |               |               |               |               |               |
|-----------------|---------------|---------------|---------------|---------------|---------------|---------------|---------------|---------------|---------------|---------------|
| V <sub>27</sub> | 0.188774E-10  | -0.146570E-09 | -0.209166E-09 | -0.683959E-10 | 0.116198E-09  | -0.232676E-09 | -0.121589E-09 | 0.865865E-09  | 0.327299E-10  | 0.327299E-10  |
|                 | 0.250211E-09  | 0.487134E-09  | -0.432405E-09 | 0.557277E-09  | 0.507141E-09  | -0.155248E-08 | 0.448218E-08  | 0.314333E-09  | -0.160023E-08 | -0.160023E-08 |
|                 | 0.719416E-09  | -0.721290E-09 | 0.755050E-09  | -0.136156E-08 | -0.275224E-08 | 0.242717E-08  | -0.108748E-08 | 0.112028E-08  | 0.796670E-08  | 0.796670E-08  |
|                 | -0.477091E-09 | 0.242415E-08  | -0.247292E-08 | 0.790131E-08  | -0.312381E-08 | 0.885523E-08  | 0.260953E-09  | -0.152340E-09 | 0.193425E-08  | 0.193425E-08  |
| V <sub>26</sub> | 0.353767E-10  | -0.134470E-08 | 0.888932E-09  | -0.524843E-09 | 0.120418E-08  | 0.211089E-08  | -0.247571E-08 | 0.850911E-08  | -0.119438E-08 | -0.119438E-08 |
|                 | 0.112558E-08  | -0.114982E-06 | -0.406286E-07 | -0.338249E-07 | -0.112480E-06 | 0.267189E-06  |               |               |               |               |
|                 | 0.753899E-10  | 0.489697E-10  | 0.878084E-10  | -0.330296E-10 | -0.315962E-10 | -0.510047E-10 | -0.592146E-10 | -0.120837E-09 | 0.157411E-09  | 0.157411E-09  |
|                 | 0.297298E-09  | -0.137087E-09 | -0.408707E-09 | -0.153034E-09 | 0.287382E-09  | 0.345756E-09  | 0.215418E-09  | 0.407017E-09  | 0.109658E-08  | 0.109658E-08  |
| V <sub>25</sub> | 0.135820E-09  | -0.560301E-10 | -0.137313E-09 | -0.156069E-08 | -0.263355E-09 | -0.134839E-08 | 0.411975E-09  | -0.170401E-10 | -0.394587E-09 | -0.394587E-09 |
|                 | 0.120093E-08  | 0.856841E-09  | -0.341620E-08 | 0.289873E-08  | 0.136615E-09  | 0.191003E-07  | -0.291007E-10 | 0.154141E-09  | 0.638649E-09  | 0.638649E-09  |
|                 | -0.750425E-09 | -0.967936E-09 | -0.191645E-08 | 0.127008E-09  | -0.275115E-10 | 0.656548E-09  | -0.431679E-09 | 0.375769E-09  | -0.783232E-10 | -0.783232E-10 |
|                 | 0.120299E-09  | -0.167049E-07 | 0.106057E-07  | -0.312092E-07 | -0.294709E-07 | 0.586475E-07  |               |               |               |               |
| V <sub>24</sub> | -0.102808E-09 | -0.427202E-09 | -0.780639E-09 | -0.265484E-09 | -0.648723E-10 | 0.166447E-09  | 0.694939E-09  | -0.100033E-09 | 0.253052E-08  | 0.253052E-08  |
|                 | 0.930857E-09  | 0.194574E-09  | -0.540532E-09 | 0.416430E-09  | 0.489686E-10  | -0.388258E-08 | -0.836297E-09 | 0.102572E-08  | 0.487807E-09  | 0.487807E-09  |
|                 | -0.344606E-09 | -0.640310E-09 | -0.366574E-09 | -0.200556E-08 | 0.767450E-09  | 0.169087E-08  | 0.132829E-08  | -0.127447E-08 | 0.116591E-09  | 0.116591E-09  |
|                 | 0.444892E-09  | -0.224004E-08 | -0.117136E-07 | -0.445092E-08 | 0.251730E-08  | 0.880673E-08  | 0.298248E-09  | 0.111641E-09  | 0.802192E-08  | 0.802192E-08  |
| V <sub>23</sub> | 0.347758E-08  | -0.229030E-08 | 0.402760E-08  | -0.179000E-10 | 0.212990E-10  | 0.301318E-08  | -0.445365E-08 | 0.221805E-08  | -0.565583E-09 | -0.565583E-09 |
|                 | -0.696750E-09 | -0.343721E-06 | 0.198736E-08  | -0.257051E-06 | -0.332499E-06 | 0.428052E-06  |               |               |               |               |
|                 | 0.302465E-09  | 0.124967E-09  | 0.480121E-09  | 0.368639E-09  | -0.873739E-10 | -0.158500E-08 | -0.347077E-08 | 0.158940E-08  | -0.125127E-08 | -0.125127E-08 |
|                 | -0.786780E-09 | -0.191529E-09 | -0.599331E-09 | -0.839558E-09 | 0.444192E-09  | 0.152541E-08  | -0.259408E-09 | 0.931176E-10  | -0.266398E-11 | -0.266398E-11 |
| V <sub>22</sub> | -0.395806E-09 | 0.839933E-09  | 0.115508E-08  | -0.653780E-09 | -0.105443E-08 | 0.531254E-09  | 0.724324E-09  | -0.523788E-08 | 0.127239E-09  | 0.127239E-09  |
|                 | 0.692656E-10  | 0.157246E-09  | 0.106039E-07  | -0.370753E-08 | 0.100948E-08  | 0.841355E-08  | 0.449228E-09  | 0.109755E-09  | 0.109242E-07  | 0.109242E-07  |
|                 | -0.294710E-08 | -0.338030E-10 | -0.194200E-08 | 0.107298E-08  | -0.622636E-09 | 0.146026E-08  | -0.177711E-08 | 0.182162E-08  | -0.444173E-09 | -0.444173E-09 |
|                 | 0.428413E-08  | -0.937618E-07 | -0.268667E-06 | 0.151978E-06  | 0.465859E-06  | 0.535823E-06  |               |               |               |               |
| V <sub>21</sub> | 0.116106E-09  | -0.843025E-10 | 0.176791E-09  | 0.406340E-10  | -0.114169E-09 | -0.279840E-09 | -0.228631E-09 | -0.272155E-08 | 0.862282E-09  | 0.862282E-09  |
|                 | 0.993123E-09  | 0.497776E-09  | -0.129138E-08 | 0.117656E-08  | 0.959270E-09  | -0.187744E-08 | 0.108423E-08  | -0.354797E-08 | -0.175694E-08 | -0.175694E-08 |
|                 | 0.109777E-08  | -0.181784E-08 | 0.739366E-09  | -0.519900E-09 | 0.329240E-09  | -0.262194E-08 | -0.225531E-08 | -0.217846E-07 | -0.318032E-09 | -0.318032E-09 |
|                 | -0.631380E-08 | 0.310391E-08  | -0.174090E-07 | 0.499985E-07  | -0.310234E-08 | 0.478946E-07  | -0.123090E-09 | 0.546292E-09  | -0.531610E-07 | -0.531610E-07 |
| V <sub>20</sub> | 0.159179E-07  | -0.735161E-09 | 0.729547E-08  | -0.233368E-08 | -0.613575E-09 | -0.266108E-09 | 0.659932E-10  | 0.419202E-09  | -0.312746E-09 | -0.312746E-09 |
|                 | 0.357289E-09  | -0.348345E-07 | -0.811175E-07 | -0.319114E-07 | -0.516924E-07 | 0.217596E-06  |               |               |               |               |
|                 | -0.242662E-09 | -0.733111E-10 | -0.248042E-10 | 0.222803E-10  | 0.146113E-09  | 0.143392E-09  | 0.734846E-10  | -0.223744E-08 | 0.808904E-09  | 0.808904E-09  |
|                 | 0.423627E-09  | -0.308635E-09 | 0.333346E-09  | -0.504163E-09 | -0.379167E-09 | 0.126288E-08  | -0.928940E-09 | 0.189365E-08  | 0.982392E-09  | 0.982392E-09  |
| V <sub>19</sub> | -0.765872E-09 | 0.100393E-08  | -0.824619E-09 | 0.174336E-08  | 0.127023E-08  | 0.127023E-08  | -0.544071E-10 | 0.237290E-07  | -0.106788E-08 | -0.106788E-08 |
|                 | 0.411712E-09  | 0.463788E-09  | -0.167497E-08 | -0.241379E-07 | -0.331468E-08 | 0.516972E-07  | 0.451925E-09  | -0.206151E-09 | 0.302693E-07  | 0.302693E-07  |
|                 | -0.177688E-07 | 0.761853E-09  | 0.548350E-08  | 0.748643E-09  | -0.642770E-10 | 0.853416E-09  | -0.931659E-09 | 0.532224E-09  | 0.120333E-09  | 0.120333E-09  |
|                 | -0.496918E-09 | 0.351325E-07  | 0.173363E-06  | -0.420419E-07 | 0.134948E-07  | 0.210516E-06  |               |               |               |               |
| V <sub>18</sub> | -0.152199E-09 | -0.143251E-09 | -0.784441E-10 | -0.212319E-10 | 0.523303E-10  | 0.644132E-10  | 0.173764E-09  | -0.210418E-08 | 0.189776E-08  | 0.189776E-08  |
|                 | 0.590767E-09  | -0.716508E-10 | -0.649701E-10 | 0.299618E-09  | 0.449288E-09  | -0.679830E-09 | 0.255079E-09  | 0.340835E-09  | -0.551428E-09 | -0.551428E-09 |
|                 | 0.423818E-11  | -0.637567E-09 | 0.180705E-09  | 0.364761E-09  | 0.997360E-10  | -0.218363E-08 | 0.228851E-08  | -0.586249E-08 | 0.669378E-09  | 0.669378E-09  |
|                 | -0.206790E-08 | -0.102874E-07 | -0.349357E-07 | 0.340770E-08  | 0.103670E-08  | 0.424661E-07  | 0.415709E-09  | 0.859390E-10  | -0.672639E-08 | -0.672639E-08 |
| V <sub>17</sub> | 0.105042E-07  | 0.144236E-07  | 0.302036E-07  | -0.239881E-08 | -0.341735E-09 | 0.413353E-09  | -0.833528E-10 | 0.256215E-09  | -0.138550E-09 | -0.138550E-09 |
|                 | -0.309934E-09 | -0.100594E-06 | 0.165296E-07  | -0.154248E-06 | -0.144466E-06 | 0.226990E-06  |               |               |               |               |
|                 | 0.277940E-09  | 0.106951E-09  | 0.122791E-09  | 0.686183E-10  | -0.613549E-10 | -0.362514E-09 | -0.652422E-09 | -0.101861E-08 | -0.119557E-08 | -0.119557E-08 |
|                 | -0.587884E-10 | 0.386161E-09  | -0.302282E-10 | -0.714450E-10 | 0.119727E-09  | 0.737224E-09  | 0.580773E-09  | -0.280842E-10 | 0.262983E-09  | 0.262983E-09  |
| V <sub>16</sub> | 0.709905E-09  | 0.660544E-10  | 0.264813E-09  | -0.454401E-09 | -0.233945E-08 | 0.234935E-08  | -0.102362E-08 | -0.333723E-08 | 0.460747E-09  | 0.460747E-09  |
|                 | 0.257448E-09  | 0.732466E-08  | 0.329339E-07  | -0.285176E-09 | 0.142337E-08  | 0.422036E-07  | -0.374046E-09 | 0.319295E-09  | 0.134176E-07  | 0.134176E-07  |
|                 | -0.209845E-08 | -0.132373E-07 | -0.351092E-07 | 0.218236E-08  | 0.564997E-09  | -0.251792E-10 | -0.613489E-09 | 0.397532E-09  | -0.539242E-09 | -0.539242E-09 |
|                 | 0.104046E-08  | 0.457862E-08  | -0.120708E-07 | 0.963579E-07  | 0.192570E-06  | 0.290739E-06  |               |               |               |               |

**Table S25:** Anharmonic potential parameters  $\frac{\sqrt{h^3} \epsilon^2 \phi_i^2 \phi_j / E_h^3}{N} \frac{\partial^3 V_{\text{ReO}}}{\partial q_i^2 \partial q_j}$  (where  $N = 2$  for  $i \neq j$  and  $N = 6$  for  $i = j$ ) for  $\text{Cp}^{187}\text{Re}(\text{CH}_3)(\text{CO})(\text{NO})$ . B3LYP/cc-pV5Z,cc-pwCVQZ-PP level harmonic force field was utilised for the anharmonic calculation at B3LYP level with (12s11p10d8f)[8s7p6d4f] contraction on Re atom and cc-pVDZ basis set for H, C, N and O atoms. Values are determined by the GAUSSIAN package. (continued).

| Mode            | VBO           |               |               |               |               |               |               |               |               |               |
|-----------------|---------------|---------------|---------------|---------------|---------------|---------------|---------------|---------------|---------------|---------------|
| V <sub>19</sub> | -0.684374E-10 | -0.574680E-10 | 0.157505E-09  | 0.459794E-10  | 0.953801E-11  | -0.152586E-09 | -0.329054E-09 | -0.421518E-08 | 0.750393E-09  | -0.750333E-10 |
|                 | 0.937429E-09  | 0.896415E-10  | -0.307578E-09 | 0.170051E-09  | 0.325228E-09  | 0.148578E-09  | -0.358494E-09 | -0.634314E-09 | -0.750333E-10 | -0.158273E-08 |
|                 | 0.307366E-09  | -0.102842E-08 | 0.587124E-10  | -0.515694E-08 | -0.181754E-08 | -0.178563E-08 | -0.339163E-09 | 0.395324E-08  | -0.158273E-08 | -0.158273E-08 |
|                 | -0.487530E-08 | 0.182276E-08  | -0.407550E-08 | 0.115215E-07  | -0.181825E-08 | 0.412332E-07  | -0.772434E-10 | -0.117049E-09 | 0.916354E-08  | -0.697002E-10 |
| V <sub>18</sub> | -0.565195E-08 | 0.103129E-08  | -0.884426E-08 | 0.967416E-09  | 0.166612E-10  | 0.606965E-10  | -0.236380E-10 | 0.690717E-10  | -0.697002E-10 | -0.697002E-10 |
|                 | -0.790793E-11 | -0.145207E-08 | 0.807700E-08  | -0.426885E-08 | 0.105364E-08  | 0.424050E-07  |               |               |               |               |
|                 | -0.122437E-09 | 0.525033E-10  | 0.771038E-09  | 0.483330E-09  | 0.437212E-09  | 0.995886E-09  | -0.712004E-09 | -0.131337E-08 | 0.867636E-09  | 0.867636E-09  |
|                 | 0.541101E-09  | -0.507397E-08 | -0.146944E-07 | -0.244422E-07 | 0.561368E-08  | -0.231826E-08 | 0.584014E-09  | -0.926254E-09 | -0.178623E-09 | -0.178623E-09 |
| V <sub>17</sub> | -0.874130E-09 | 0.313041E-08  | -0.374199E-08 | 0.346673E-09  | -0.178246E-08 | 0.178010E-08  | -0.248843E-08 | -0.240330E-09 | -0.541781E-09 | -0.541781E-09 |
|                 | 0.312826E-09  | 0.293854E-09  | 0.297465E-08  | -0.239720E-09 | 0.388162E-09  | 0.998598E-09  | 0.630541E-07  | -0.397789E-09 | -0.810016E-09 | -0.810016E-09 |
|                 | 0.199420E-08  | -0.548785E-10 | 0.135146E-08  | 0.407883E-08  | -0.952623E-08 | 0.706068E-08  | -0.711713E-08 | 0.526632E-06  | 0.490094E-07  | 0.490094E-07  |
|                 | 0.105419E-06  | -0.408130E-09 | -0.521973E-09 | 0.645322E-11  | 0.559869E-09  | 0.197504E-09  | -0.155761E-09 | -0.183853E-08 | 0.341166E-09  | 0.341166E-09  |
| V <sub>16</sub> | 0.224364E-10  | -0.365124E-10 | -0.728512E-11 | 0.127109E-10  | 0.165238E-10  | -0.101774E-09 | -0.155761E-09 | -0.183853E-08 | 0.341166E-09  | 0.341166E-09  |
|                 | 0.251750E-09  | 0.148399E-09  | -0.129825E-09 | 0.171188E-10  | 0.562894E-10  | -0.617944E-10 | 0.767634E-10  | 0.344173E-09  | 0.233439E-10  | 0.233439E-10  |
|                 | 0.892858E-12  | -0.132007E-10 | -0.377386E-09 | 0.241695E-08  | 0.134398E-08  | 0.231282E-09  | 0.608087E-09  | -0.145743E-08 | -0.194115E-09 | -0.194115E-09 |
|                 | -0.587843E-09 | 0.690350E-09  | -0.288372E-08 | 0.263444E-08  | 0.118596E-09  | 0.234563E-07  | 0.576667E-10  | 0.780608E-10  | 0.399080E-09  | 0.399080E-09  |
| V <sub>15</sub> | -0.703587E-10 | 0.117069E-09  | -0.609705E-09 | -0.223438E-09 | -0.455063E-10 | 0.151911E-09  | -0.378073E-09 | 0.244441E-09  | -0.470874E-09 | -0.470874E-09 |
|                 | 0.347378E-09  | -0.544653E-07 | 0.262859E-07  | -0.554675E-07 | -0.425609E-08 | 0.399407E-06  |               |               |               |               |
|                 | -0.107497E-09 | -0.136977E-09 | 0.343840E-10  | -0.685030E-10 | 0.555340E-10  | -0.418783E-09 | -0.153728E-09 | -0.664995E-08 | 0.241612E-08  | 0.241612E-08  |
|                 | 0.454786E-08  | 0.531824E-09  | 0.135621E-09  | 0.151626E-10  | -0.669427E-09 | 0.358842E-09  | -0.124389E-08 | 0.138941E-08  | 0.127719E-08  | 0.127719E-08  |
| V <sub>14</sub> | 0.142902E-08  | -0.403044E-08 | -0.260007E-08 | -0.636302E-08 | -0.418856E-08 | -0.502676E-08 | 0.209025E-08  | 0.343486E-08  | -0.674757E-08 | -0.674757E-08 |
|                 | -0.590476E-08 | 0.653623E-07  | -0.901025E-07 | 0.339225E-08  | 0.712302E-08  | 0.166969E-06  | 0.151408E-08  | 0.133560E-08  | 0.446320E-08  | 0.446320E-08  |
|                 | -0.266850E-07 | -0.585672E-07 | 0.108997E-06  | -0.826130E-08 | -0.244325E-08 | -0.102776E-08 | 0.305430E-08  | 0.531236E-09  | -0.560977E-09 | -0.560977E-09 |
|                 | -0.246029E-09 | -0.878680E-08 | 0.331160E-07  | 0.210501E-07  | -0.184230E-06 | 0.224254E-06  | -0.226175E-09 | -0.420747E-08 | 0.953048E-09  | 0.953048E-09  |
| V <sub>13</sub> | -0.914490E-09 | 0.137556E-09  | 0.775008E-09  | 0.180603E-09  | 0.189697E-08  | -0.245615E-09 | 0.913818E-09  | -0.918612E-09 | -0.186673E-08 | -0.186673E-08 |
|                 | 0.702083E-09  | 0.602482E-11  | 0.339118E-08  | -0.567130E-08 | -0.810156E-08 | -0.101834E-08 | -0.549770E-08 | 0.162706E-09  | 0.244177E-08  | 0.244177E-08  |
|                 | -0.854919E-08 | -0.565986E-07 | 0.417706E-07  | 0.374346E-07  | -0.768678E-08 | 0.177857E-06  | -0.151669E-08 | -0.145904E-08 | -0.588453E-08 | -0.588453E-08 |
|                 | 0.760386E-08  | 0.625723E-07  | -0.965514E-07 | 0.746949E-08  | 0.189340E-08  | -0.202254E-08 | 0.203158E-08  | -0.596235E-09 | 0.279997E-09  | 0.279997E-09  |
| V <sub>12</sub> | 0.105966E-08  | -0.122059E-07 | 0.713830E-07  | -0.105871E-06 | 0.115997E-06  | 0.200084E-06  | -0.839913E-09 | -0.495706E-08 | -0.136543E-08 | -0.136543E-08 |
|                 | 0.634224E-09  | 0.724861E-10  | 0.285837E-09  | -0.374357E-10 | -0.450794E-09 | -0.625632E-09 | 0.330739E-08  | -0.662433E-09 | -0.286632E-09 | -0.286632E-09 |
|                 | 0.404524E-09  | 0.814376E-09  | -0.827533E-09 | 0.657965E-09  | 0.104051E-08  | -0.959416E-09 | -0.750258E-08 | -0.282103E-07 | 0.274846E-08  | 0.274846E-08  |
|                 | -0.138331E-08 | 0.479051E-09  | -0.255940E-08 | 0.219243E-09  | -0.208397E-08 | 0.731400E-08  | 0.683395E-08  | -0.352575E-08 | -0.352575E-08 | -0.352575E-08 |
| V <sub>11</sub> | -0.307334E-08 | -0.495055E-08 | -0.633488E-08 | -0.147589E-07 | -0.108277E-07 | 0.110753E-06  | 0.895436E-09  | -0.771718E-09 | 0.744764E-07  | 0.744764E-07  |
|                 | -0.663006E-07 | 0.128646E-07  | -0.831289E-09 | 0.342428E-08  | -0.794700E-09 | 0.122965E-08  | -0.543420E-09 | 0.212821E-08  | -0.161373E-09 | -0.161373E-09 |
|                 | -0.135571E-08 | -0.218413E-07 | 0.181603E-06  | -0.505554E-07 | 0.765485E-08  | 0.231129E-06  |               |               |               |               |
|                 | 0.161050E-09  | 0.225297E-09  | 0.467618E-09  | 0.503723E-09  | 0.348246E-09  | -0.147826E-08 | 0.332012E-09  | 0.108671E-08  | 0.239519E-09  | 0.239519E-09  |
| V <sub>10</sub> | 0.827778E-11  | 0.991437E-10  | -0.166541E-08 | -0.268591E-08 | 0.940302E-09  | 0.515174E-09  | 0.516668E-09  | -0.126578E-08 | 0.577928E-10  | 0.577928E-10  |
|                 | -0.988264E-09 | 0.136093E-07  | -0.834611E-08 | -0.278742E-08 | -0.239448E-08 | 0.525477E-09  | -0.125542E-08 | -0.120640E-09 | -0.495935E-09 | -0.495935E-09 |
|                 | -0.145915E-08 | 0.211182E-09  | 0.215956E-10  | 0.830787E-09  | -0.266736E-09 | 0.419808E-09  | 0.347417E-07  | -0.520697E-10 | -0.320994E-08 | -0.320994E-08 |
|                 | 0.504337E-09  | -0.849644E-09 | 0.876177E-08  | 0.377317E-07  | 0.177867E-07  | -0.255414E-09 | 0.828979E-09  | 0.349170E-06  | 0.546114E-07  | 0.546114E-07  |
| V <sub>9</sub>  | -0.152224E-06 | -0.430276E-09 | 0.205844E-09  | 0.277263E-09  | 0.11270E-08   | 0.164632E-08  |               |               |               |               |

**Table S25:** Anharmonic potential parameters  $\frac{\sqrt{h^3 c^3 \phi_i^2 \phi_j / E_h^3}}{N} \frac{\partial^3 V_{\text{BO}}}{\partial q_i^2 \partial q_j}$  (where  $N = 2$  for  $i \neq j$  and  $N = 6$  for  $i = j$ ) for  $\text{Cp}^{187}\text{Re}(\text{CH}_3)(\text{CO})(\text{NO})$ . B3LYP/cc-pV5Z,cc-pwCVQZ-PP level harmonic force field was utilised for the anharmonic calculation at B3LYP level with (12s11p10d8f)[8s7p6d4f] contraction on Re atom and cc-pVDZ basis set for H, C, N and O atoms. Values are determined by the GAUSSIAN package. (continued).

| Mode            | VBO           |               |               |               |               |               |               |               |               |               |
|-----------------|---------------|---------------|---------------|---------------|---------------|---------------|---------------|---------------|---------------|---------------|
| V <sub>11</sub> | -0.274397E-09 | 0.214886E-09  | 0.593144E-09  | 0.636707E-09  | 0.228214E-10  | 0.142715E-08  | -0.170227E-08 | 0.797758E-09  | 0.849900E-09  | -0.976977E-09 |
|                 | 0.196603E-09  | -0.838809E-09 | -0.197763E-08 | -0.374584E-08 | 0.119449E-08  | 0.160617E-08  | 0.797858E-09  | -0.121030E-08 | -0.315465E-09 | -0.170292E-08 |
|                 | -0.289887E-09 | -0.105534E-07 | 0.671723E-08  | 0.226188E-08  | 0.141219E-08  | 0.718296E-09  | -0.426329E-09 | 0.108954E-08  | -0.315465E-09 | -0.170292E-08 |
|                 | 0.336169E-08  | -0.214381E-09 | 0.880962E-09  | -0.769534E-09 | 0.747028E-10  | 0.277858E-09  | 0.358904E-07  | -0.122146E-09 | 0.170292E-08  | -0.458649E-08 |
| V <sub>10</sub> | 0.383958E-09  | 0.951698E-09  | -0.801776E-08 | -0.105333E-06 | -0.110781E-07 | 0.313004E-09  | 0.101980E-09  | 0.271190E-06  | -0.458649E-08 | -0.170292E-08 |
|                 | 0.281094E-06  | 0.185581E-09  | 0.109036E-08  | -0.411948E-09 | -0.625197E-09 | -0.151409E-09 |               |               |               |               |
|                 | -0.450842E-09 | 0.724198E-09  | 0.201694E-08  | -0.659311E-09 | -0.346146E-08 | 0.163339E-08  | 0.450085E-08  | 0.352401E-08  | 0.329084E-08  | -0.458649E-08 |
|                 | -0.180605E-08 | -0.117022E-07 | -0.680651E-08 | 0.789221E-08  | 0.254898E-08  | -0.365464E-08 | 0.641861E-07  | -0.591729E-07 | 0.107760E-06  | -0.686197E-08 |
| V <sub>9</sub>  | -0.104688E-06 | -0.121254E-07 | -0.141413E-08 | -0.445286E-08 | -0.994767E-08 | -0.284647E-08 | 0.394397E-08  | 0.923218E-09  | -0.686197E-08 | -0.458649E-08 |
|                 | 0.204952E-08  | 0.206145E-08  | 0.105431E-08  | -0.246505E-08 | -0.228242E-08 | -0.481540E-09 | 0.200925E-07  | 0.163380E-09  | 0.546003E-08  | -0.458649E-08 |
|                 | -0.912659E-08 | 0.574470E-08  | 0.234388E-08  | -0.153430E-08 | 0.279091E-08  | -0.332453E-06 | 0.168326E-06  | -0.426285E-08 | 0.473561E-09  | -0.458649E-08 |
|                 | -0.101352E-08 | -0.254288E-09 | 0.616941E-09  | -0.594954E-09 | -0.258068E-09 | 0.535983E-09  |               |               |               |               |
| V <sub>8</sub>  | 0.570080E-09  | -0.483822E-09 | 0.250730E-08  | -0.313692E-09 | 0.350478E-08  | 0.239128E-08  | 0.232664E-08  | 0.457353E-08  | -0.155620E-08 | -0.458649E-08 |
|                 | 0.196029E-08  | 0.420090E-08  | -0.812499E-07 | 0.464442E-07  | -0.168944E-07 | 0.982716E-08  | 0.179689E-09  | 0.123741E-07  | 0.285465E-08  | -0.458649E-08 |
|                 | -0.229567E-07 | -0.220422E-08 | -0.298900E-08 | -0.111056E-07 | -0.715818E-08 | 0.415206E-08  | -0.310120E-08 | 0.307046E-08  | 0.770163E-08  | -0.458649E-08 |
|                 | 0.525102E-08  | -0.455590E-08 | 0.524643E-08  | -0.533926E-08 | 0.225585E-08  | -0.209353E-08 | 0.195275E-07  | -0.365756E-09 | 0.976970E-08  | -0.458649E-08 |
| V <sub>7</sub>  | 0.556821E-08  | -0.253208E-08 | -0.202116E-08 | -0.313895E-09 | -0.386023E-08 | 0.168202E-06  | 0.453374E-06  | -0.640071E-08 | -0.339600E-08 | -0.458649E-08 |
|                 | -0.363261E-08 | 0.774346E-09  | -0.481983E-09 | -0.753059E-09 | -0.824634E-09 | 0.327068E-09  |               |               |               |               |
|                 | 0.233777E-09  | 0.882342E-09  | 0.102331E-08  | 0.944136E-09  | 0.480391E-09  | -0.502983E-09 | -0.112581E-08 | 0.169252E-08  | -0.339481E-08 | -0.458649E-08 |
|                 | -0.997376E-09 | 0.496951E-08  | 0.883228E-08  | 0.182558E-07  | -0.306724E-08 | 0.114399E-07  | 0.690130E-09  | -0.339395E-08 | -0.148783E-08 | -0.458649E-08 |
| V <sub>6</sub>  | 0.876576E-09  | -0.132290E-07 | 0.767268E-08  | -0.650607E-08 | 0.171697E-08  | -0.685719E-08 | 0.654696E-08  | 0.814160E-09  | 0.318907E-08  | -0.458649E-08 |
|                 | -0.939184E-08 | -0.396747E-09 | -0.518302E-08 | 0.880794E-09  | 0.910983E-08  | -0.317338E-08 | -0.120275E-06 | 0.695504E-09  | -0.730848E-09 | -0.458649E-08 |
|                 | -0.327618E-11 | 0.138731E-08  | 0.149607E-08  | -0.588957E-08 | 0.222946E-07  | 0.134433E-07  | -0.202723E-07 | -0.150763E-05 | 0.451221E-06  | -0.458649E-08 |
|                 | 0.740306E-06  | 0.479903E-08  | 0.914109E-08  | -0.325007E-08 | -0.654218E-08 | -0.888285E-09 |               |               |               |               |
| V <sub>5</sub>  | 0.212351E-09  | 0.215173E-08  | 0.198641E-08  | 0.168926E-08  | -0.413720E-09 | -0.819658E-09 | -0.151155E-08 | 0.257127E-08  | -0.439866E-08 | -0.458649E-08 |
|                 | -0.144815E-08 | 0.666975E-08  | 0.160547E-07  | 0.321125E-07  | -0.873478E-08 | 0.192599E-07  | 0.652556E-09  | -0.497480E-08 | -0.382231E-08 | -0.458649E-08 |
|                 | 0.125954E-08  | -0.321439E-07 | 0.145388E-07  | -0.603122E-08 | 0.168411E-08  | -0.123440E-07 | 0.114622E-07  | 0.242436E-08  | 0.345030E-08  | -0.458649E-08 |
|                 | -0.978550E-08 | -0.162115E-08 | -0.986759E-08 | 0.655858E-09  | -0.866316E-09 | -0.526139E-08 | -0.371186E-06 | 0.100452E-08  | 0.571317E-08  | -0.458649E-08 |
| V <sub>4</sub>  | -0.527798E-08 | 0.497260E-08  | -0.227109E-07 | -0.317596E-06 | 0.113990E-09  | 0.101372E-07  | -0.208901E-07 | -0.508561E-05 | -0.296227E-06 | -0.458649E-08 |
|                 | 0.242181E-05  | 0.826454E-08  | 0.187620E-07  | -0.812104E-08 | -0.132547E-07 | -0.546509E-08 |               |               |               |               |
|                 | -0.250223E-09 | 0.924312E-09  | 0.387475E-09  | 0.217309E-09  | -0.150600E-08 | -0.219702E-08 | -0.510333E-08 | -0.125392E-08 | 0.199917E-08  | -0.458649E-08 |
|                 | -0.199626E-09 | 0.23847E-08   | 0.940987E-08  | 0.223790E-07  | -0.839227E-08 | 0.120139E-07  | 0.215794E-08  | -0.349489E-08 | -0.173826E-08 | -0.458649E-08 |
| V <sub>3</sub>  | 0.302396E-08  | 0.605954E-08  | -0.134650E-08 | -0.903487E-09 | 0.194437E-08  | -0.641789E-08 | 0.664853E-08  | 0.219802E-08  | 0.239868E-08  | -0.458649E-08 |
|                 | -0.744193E-08 | -0.109287E-08 | -0.812737E-08 | 0.144599E-08  | -0.911898E-09 | -0.355666E-09 | -0.365204E-06 | 0.618837E-09  | -0.498846E-08 | -0.458649E-08 |
|                 | 0.154004E-09  | -0.263721E-08 | 0.220564E-07  | 0.318178E-06  | 0.125704E-07  | 0.120799E-07  | -0.313788E-07 | -0.350447E-05 | -0.654922E-06 | -0.458649E-08 |
|                 | -0.195870E-05 | -0.711137E-08 | -0.211243E-07 | 0.110149E-07  | 0.164888E-07  | 0.859264E-08  |               |               |               |               |
| V <sub>2</sub>  | -0.369675E-10 | 0.551830E-09  | 0.132980E-09  | 0.181596E-09  | 0.253344E-09  | -0.416851E-09 | -0.686543E-09 | 0.101939E-08  | -0.132261E-08 | -0.458649E-08 |
|                 | 0.118828E-08  | 0.117227E-08  | 0.876304E-09  | 0.196597E-09  | -0.225516E-08 | 0.812982E-09  | -0.143383E-08 | -0.152077E-08 | -0.108379E-08 | -0.458649E-08 |
|                 | 0.876430E-09  | -0.458142E-09 | -0.853495E-09 | -0.910414E-09 | 0.385973E-08  | 0.543468E-09  | -0.607038E-09 | -0.482916E-09 | -0.812389E-08 | -0.458649E-08 |
|                 | -0.338643E-08 | -0.156573E-07 | -0.242928E-07 | 0.127221E-07  | -0.736738E-08 | 0.108831E-06  | 0.834789E-09  | -0.943145E-09 | 0.218940E-07  | -0.458649E-08 |
| V <sub>1</sub>  | 0.136916E-07  | 0.682620E-07  | 0.455435E-07  | -0.195387E-08 | -0.979664E-09 | 0.205114E-08  | -0.973413E-09 | -0.361158E-09 | 0.117713E-09  | -0.458649E-08 |
|                 | 0.430623E-08  | 0.116309E-05  | -0.904416E-06 | 0.378124E-05  | 0.631233E-06  | -0.289817E-05 |               |               |               |               |
|                 | -0.332143E-09 | 0.238057E-09  | 0.397936E-10  | 0.499410E-10  | -0.118068E-09 | -0.739634E-09 | -0.138895E-08 | 0.271524E-08  | 0.324935E-08  | -0.458649E-08 |
|                 | 0.117197E-09  | -0.769587E-09 | 0.908688E-09  | 0.151157E-08  | -0.733657E-09 | -0.273647E-08 | -0.148565E-08 | 0.193162E-09  | -0.232617E-08 | -0.458649E-08 |
| V <sub>0</sub>  | -0.951605E-09 | -0.412848E-08 | 0.388177E-08  | 0.210420E-08  | -0.21641E-08  | -0.495373E-08 | 0.293799E-08  | 0.176237E-10  | -0.392680E-08 | -0.458649E-08 |
|                 | -0.450353E-09 | 0.148760E-07  | 0.266368E-08  | 0.127525E-07  | 0.130803E-08  | 0.109728E-06  | 0.55575E-08   | 0.214120E-08  | 0.611876E-08  | -0.458649E-08 |
|                 | -0.364958E-08 | -0.495951E-07 | -0.396099E-07 | 0.227052E-08  | 0.161571E-08  | 0.327102E-09  | -0.398200E-08 | 0.118921E-08  | 0.749124E-08  | -0.458649E-08 |
|                 | -0.108839E-07 | -0.485703E-07 | -0.371325E-06 | -0.221010E-05 | -0.845627E-06 | -0.411657E-05 |               |               |               |               |

**Table S25:** Anharmonic potential parameters  $\frac{\sqrt{\mu^3} \epsilon^3 \omega_0^2 \omega_j / E_h^3}{N} \frac{\partial^3 V_{802}}{\partial q_i^2 \partial q_j}$  (where  $N = 2$  for  $i \neq j$  and  $N = 6$  for  $i = j$ ) for  $\text{Cp}^{187}\text{Re}(\text{CH}_3)(\text{CO})(\text{NO})$ , B3LYP/cc-pV5Z,cc-pwCVQZ-PP level harmonic force field was utilised for the anharmonic calculation at B3LYP level with (12s11p10d8f)[8s7p6d4f] contraction on Re atom and cc-pVDZ basis set for H, C, N and O atoms. Values are determined by the GAUSSIAN package. (continued).

| Mode           | VBO           |               |               |               |               |               |               |               |               |  |  |  |
|----------------|---------------|---------------|---------------|---------------|---------------|---------------|---------------|---------------|---------------|--|--|--|
| v <sub>3</sub> | 0.224805E-11  | 0.353717E-09  | -0.106103E-09 | -0.123928E-09 | 0.790779E-10  | -0.353892E-09 | -0.489867E-09 | 0.122636E-08  | 0.836484E-09  |  |  |  |
|                | 0.873170E-09  | 0.531461E-09  | 0.793585E-09  | 0.697154E-09  | -0.122840E-08 | -0.190807E-08 | -0.102818E-08 | 0.132270E-08  | -0.217837E-09 |  |  |  |
|                | 0.707597E-09  | -0.196571E-08 | 0.217306E-08  | -0.187125E-08 | -0.260260E-10 | -0.423187E-08 | -0.676183E-10 | 0.149288E-08  | -0.252365E-08 |  |  |  |
|                | -0.267790E-09 | -0.548463E-08 | -0.436104E-08 | 0.114226E-07  | -0.485541E-09 | 0.117617E-06  | 0.271526E-08  | 0.220230E-09  | 0.240765E-08  |  |  |  |
|                | 0.223308E-07  | 0.170338E-07  | -0.229857E-07 | 0.293013E-08  | 0.679302E-09  | -0.822233E-09 | -0.172473E-08 | -0.263063E-08 | 0.133658E-08  |  |  |  |
| v <sub>2</sub> | 0.543957E-08  | 0.250559E-06  | -0.283226E-05 | 0.367711E-06  | -0.107307E-05 | -0.343444E-05 |               |               |               |  |  |  |
|                | 0.467984E-09  | -0.657830E-10 | 0.417777E-09  | 0.488149E-09  | -0.995846E-10 | -0.603035E-09 | -0.181194E-08 | 0.184003E-08  | 0.125913E-08  |  |  |  |
|                | 0.435101E-09  | 0.128160E-08  | 0.938880E-09  | 0.863540E-09  | 0.481165E-09  | -0.105965E-08 | 0.188227E-08  | -0.163092E-08 | -0.386854E-08 |  |  |  |
|                | -0.641107E-09 | -0.255945E-08 | 0.115832E-08  | 0.612282E-08  | 0.657432E-08  | -0.637526E-08 | 0.209424E-08  | -0.268933E-08 | -0.581230E-08 |  |  |  |
|                | -0.256316E-08 | 0.788869E-08  | -0.123949E-07 | 0.164934E-07  | 0.588159E-08  | 0.117789E-06  | 0.426255E-08  | -0.535887E-09 | 0.200002E-07  |  |  |  |
| v <sub>1</sub> | -0.362254E-07 | -0.949871E-08 | 0.810092E-08  | -0.824979E-09 | -0.192822E-08 | 0.212384E-05  | 0.318456E-09  | 0.187025E-08  | 0.826550E-08  |  |  |  |
|                | -0.131205E-07 | -0.132874E-05 | 0.260468E-05  | 0.345586E-06  | 0.385283E-06  | -0.428577E-05 |               |               |               |  |  |  |
|                | 0.117168E-09  | 0.132948E-09  | 0.278469E-09  | 0.217070E-09  | -0.107121E-09 | -0.626393E-09 | -0.147526E-08 | 0.113887E-08  | 0.160342E-08  |  |  |  |
|                | 0.722995E-09  | 0.425641E-09  | 0.793705E-09  | 0.995995E-09  | -0.278400E-09 | -0.165970E-08 | 0.981083E-10  | -0.860128E-09 | -0.259917E-08 |  |  |  |
|                | -0.508305E-09 | -0.302347E-08 | 0.207011E-08  | 0.132568E-08  | 0.257264E-08  | -0.510534E-08 | 0.186827E-08  | -0.108239E-08 | -0.510321E-08 |  |  |  |
| v <sub>1</sub> | -0.239372E-08 | 0.102591E-07  | -0.524670E-08 | 0.155463E-07  | 0.294806E-08  | 0.123739E-06  | 0.407242E-08  | 0.661744E-09  | 0.137284E-07  |  |  |  |
|                | -0.131944E-07 | -0.225476E-07 | -0.148752E-07 | 0.981406E-09  | -0.116130E-09 | 0.616262E-09  | -0.946640E-09 | 0.985913E-09  | 0.686697E-08  |  |  |  |
|                | -0.976467E-08 | -0.273271E-06 | 0.394032E-06  | -0.419210E-06 | 0.463261E-07  | -0.134743E-05 |               |               |               |  |  |  |

**Table S26:** Anharmonic potential parameters  $\frac{\sqrt{h^3 c^3 \theta_1^2 \theta_2 / E_h^3}}{N} \frac{\partial^3 V_{\text{ReO}}}{\partial q_i^2 \partial q_j}$  (where  $N = 2$  for  $i \neq j$  and  $N = 6$  for  $i = j$ ) for  $\text{Cp}^{85}\text{Re}(\text{CH}_3)(\text{CO})(\text{NO})$ . B3LYP/cc-pV5Z,cc-pwCVQZ-PP level harmonic force field was utilised for the anharmonic calculation at B3LYP level with (12s11p10d8f)[8s7p6d4f] contraction on Re atom and cc-pVDZ basis set for H, C, N and O atoms. Values are determined by the GAUSSIAN package.

| Mode            | VBO           |               |               |               |               |               |               |               |               |  |
|-----------------|---------------|---------------|---------------|---------------|---------------|---------------|---------------|---------------|---------------|--|
| V <sub>51</sub> | 0.607590E-12  | 0.932772E-11  | -0.363741E-10 | -0.208616E-10 | 0.962783E-11  | -0.129727E-10 | -0.435948E-10 | 0.112599E-09  | -0.292901E-09 |  |
|                 | -0.417441E-09 | 0.171769E-10  | 0.307222E-09  | -0.582226E-10 | -0.137027E-10 | 0.587046E-10  | -0.244520E-09 | 0.109121E-09  | -0.243622E-09 |  |
|                 | 0.139613E-09  | 0.258229E-09  | 0.685445E-11  | 0.188412E-09  | 0.571214E-12  | 0.266493E-09  | 0.333439E-10  | -0.867017E-10 | 0.153282E-09  |  |
|                 | 0.447010E-09  | -0.270016E-09 | 0.883021E-09  | -0.145749E-08 | 0.100014E-09  | -0.111667E-07 | -0.126494E-09 | 0.241381E-10  | -0.700538E-09 |  |
| V <sub>50</sub> | 0.265258E-09  | -0.797605E-10 | 0.382893E-09  | -0.430729E-09 | -0.363863E-10 | 0.488642E-09  | -0.159970E-08 | 0.412348E-08  | 0.507790E-09  |  |
|                 | 0.135669E-08  | -0.213155E-08 | 0.185170E-08  | -0.250531E-08 | 0.613931E-09  | 0.174258E-07  |               |               |               |  |
|                 | 0.222374E-10  | 0.124003E-10  | -0.179661E-10 | 0.280192E-11  | 0.132247E-10  | -0.164672E-11 | -0.202312E-10 | -0.196440E-09 | -0.133400E-09 |  |
|                 | 0.493875E-10  | 0.120917E-09  | 0.484627E-09  | -0.926103E-10 | 0.107146E-09  | 0.436757E-10  | -0.742148E-09 | 0.624496E-09  | -0.128695E-08 |  |
| V <sub>49</sub> | 0.108782E-08  | 0.132605E-09  | 0.842251E-10  | 0.123182E-09  | 0.257846E-09  | -0.106491E-09 | -0.217130E-09 | -0.663772E-09 | 0.151466E-09  |  |
|                 | -0.409818E-12 | -0.504403E-10 | 0.536290E-10  | 0.593408E-09  | 0.380567E-09  | -0.164769E-08 | -0.649497E-10 | 0.438658E-10  | -0.297164E-09 |  |
|                 | 0.343282E-09  | -0.100069E-09 | 0.351301E-10  | -0.138987E-09 | -0.104643E-09 | 0.899355E-08  | -0.490504E-08 | 0.102689E-08  | 0.193038E-09  |  |
|                 | -0.117281E-09 | -0.691148E-09 | 0.232677E-08  | -0.460546E-09 | 0.158205E-09  | 0.232823E-08  |               |               |               |  |
| V <sub>48</sub> | -0.117254E-11 | 0.289827E-10  | -0.128629E-11 | -0.799071E-11 | 0.170594E-10  | -0.237451E-10 | -0.222870E-10 | -0.157058E-09 | -0.427624E-10 |  |
|                 | -0.265730E-10 | 0.745105E-10  | 0.117965E-08  | -0.609731E-09 | 0.211320E-09  | -0.147192E-09 | -0.372741E-09 | 0.102631E-09  | -0.698105E-09 |  |
|                 | 0.105570E-08  | 0.137100E-09  | -0.490915E-10 | 0.171230E-09  | 0.120977E-10  | 0.215790E-09  | 0.167756E-09  | 0.200965E-09  | -0.815654E-10 |  |
|                 | 0.234052E-10  | 0.493083E-10  | 0.103509E-09  | -0.453751E-09 | -0.366895E-09 | -0.910394E-09 | -0.173773E-09 | -0.455583E-11 | -0.132111E-09 |  |
| V <sub>47</sub> | -0.154875E-09 | 0.268535E-11  | -0.586934E-11 | 0.509060E-10  | 0.570371E-10  | 0.386161E-08  | -0.168510E-07 | 0.343430E-09  | -0.302000E-10 |  |
|                 | 0.114672E-09  | 0.280083E-10  | -0.100749E-08 | -0.381964E-09 | -0.945656E-10 | 0.175480E-08  |               |               |               |  |
|                 | 0.289835E-11  | 0.793310E-11  | 0.253047E-10  | -0.158232E-10 | 0.782317E-11  | -0.118334E-10 | -0.266527E-10 | -0.162163E-09 | -0.423548E-10 |  |
|                 | 0.702959E-11  | 0.639227E-10  | 0.932286E-09  | -0.443231E-09 | 0.221626E-09  | -0.162385E-09 | -0.632994E-09 | 0.403716E-09  | -0.112191E-08 |  |
| V <sub>46</sub> | 0.153801E-08  | 0.290925E-09  | -0.752140E-11 | 0.104922E-09  | 0.121417E-09  | 0.219302E-09  | 0.313589E-10  | 0.208049E-09  | -0.359367E-10 |  |
|                 | 0.947050E-11  | 0.234438E-10  | 0.587900E-10  | -0.378087E-09 | -0.136397E-09 | -0.636313E-09 | -0.152363E-09 | -0.327284E-11 | -0.112313E-09 |  |
|                 | -0.409194E-10 | -0.420290E-10 | 0.116588E-10  | 0.558016E-10  | 0.145976E-10  | 0.824440E-08  | -0.144371E-07 | 0.512097E-09  | -0.797327E-10 |  |
|                 | 0.373165E-09  | -0.650365E-10 | -0.770387E-09 | -0.140330E-09 | 0.569419E-11  | 0.112997E-08  |               |               |               |  |
| V <sub>45</sub> | -0.195308E-10 | 0.101019E-10  | -0.355628E-11 | 0.481581E-11  | 0.200793E-10  | 0.560797E-11  | -0.254063E-10 | -0.544092E-12 | -0.406611E-10 |  |
|                 | -0.165946E-10 | 0.385651E-09  | 0.110111E-08  | 0.116120E-08  | -0.191071E-09 | 0.393912E-09  | -0.243925E-09 | 0.241361E-09  | -0.431469E-09 |  |
|                 | 0.250160E-09  | -0.529916E-09 | 0.757343E-09  | 0.112264E-09  | 0.332227E-09  | 0.860976E-10  | 0.163270E-09  | -0.601506E-10 | 0.139305E-10  |  |
|                 | 0.280580E-10  | 0.240697E-10  | 0.146305E-09  | 0.386161E-09  | -0.662749E-10 | -0.117231E-08 | 0.944971E-09  | -0.239063E-10 | 0.245919E-10  |  |
| V <sub>44</sub> | -0.227685E-11 | -0.585962E-10 | -0.906795E-10 | -0.122659E-08 | 0.136771E-09  | 0.407644E-08  | -0.652930E-08 | 0.281882E-07  | 0.921252E-09  |  |
|                 | -0.130836E-07 | 0.405845E-09  | 0.122153E-08  | -0.388256E-09 | 0.126924E-09  | 0.174310E-08  |               |               |               |  |
|                 | -0.189690E-09 | 0.141943E-10  | 0.257771E-09  | 0.244363E-09  | 0.198112E-09  | -0.816194E-09 | -0.757523E-09 | 0.202069E-09  | 0.108208E-08  |  |
|                 | 0.137528E-09  | -0.287373E-09 | -0.126896E-08 | -0.190512E-08 | 0.784212E-09  | -0.241422E-09 | -0.113680E-09 | -0.685025E-09 | -0.480778E-09 |  |
| V <sub>43</sub> | -0.887772E-09 | 0.403834E-08  | 0.444053E-08  | -0.514776E-09 | 0.203936E-08  | 0.848337E-09  | 0.672994E-09  | 0.409668E-09  | -0.366467E-09 |  |
|                 | 0.339799E-09  | -0.135175E-09 | -0.593097E-09 | -0.247162E-10 | -0.850894E-09 | -0.553653E-09 | -0.273645E-07 | -0.149042E-09 | -0.496436E-09 |  |
|                 | -0.582692E-09 | 0.100434E-10  | 0.133653E-09  | -0.453371E-09 | -0.211281E-08 | -0.146714E-08 | 0.597529E-09  | 0.479508E-06  | 0.241902E-07  |  |
|                 | 0.106460E-06  | -0.286286E-09 | -0.108437E-08 | 0.812155E-10  | 0.814480E-09  | 0.109332E-08  |               |               |               |  |
| V <sub>42</sub> | 0.415061E-10  | 0.262151E-09  | 0.224288E-09  | 0.135860E-09  | -0.178392E-09 | 0.861066E-09  | -0.100028E-08 | 0.370009E-09  | 0.842649E-09  |  |
|                 | 0.369763E-09  | 0.483665E-10  | -0.480692E-09 | -0.481329E-09 | 0.180166E-09  | -0.318167E-09 | 0.174134E-09  | -0.677512E-09 | -0.562506E-09 |  |
|                 | -0.185922E-09 | 0.145577E-10  | -0.285944E-08 | 0.703782E-09  | -0.670275E-09 | 0.278437E-09  | -0.573660E-09 | 0.284817E-09  | 0.165828E-09  |  |
|                 | 0.863863E-09  | 0.200054E-09  | -0.179396E-09 | -0.150723E-09 | 0.773156E-09  | -0.577278E-09 | -0.898229E-08 | 0.191596E-09  | 0.430925E-11  |  |
| V <sub>41</sub> | 0.272261E-09  | 0.933323E-10  | 0.359154E-09  | 0.158128E-08  | 0.626720E-08  | 0.378836E-09  | -0.771374E-10 | 0.180948E-06  | 0.582999E-07  |  |
|                 | 0.518370E-07  | -0.726105E-09 | -0.117412E-08 | 0.305277E-09  | 0.702412E-09  | 0.159364E-08  |               |               |               |  |
|                 | 0.265525E-10  | -0.113471E-09 | -0.235877E-09 | 0.118682E-09  | 0.100276E-10  | -0.188085E-09 | -0.179531E-09 | 0.180549E-08  | -0.227464E-09 |  |
|                 | 0.791946E-09  | -0.207072E-09 | -0.635411E-09 | 0.575173E-10  | -0.158767E-09 | 0.315888E-09  | -0.941099E-10 | -0.438724E-09 | 0.312510E-09  |  |
| V <sub>40</sub> | 0.416801E-09  | -0.978576E-10 | -0.107589E-09 | -0.925924E-09 | -0.427871E-10 | -0.482850E-09 | -0.185861E-09 | 0.135718E-09  | -0.715934E-09 |  |
|                 | -0.166670E-09 | -0.793468E-10 | -0.920721E-09 | 0.451932E-09  | 0.569177E-10  | 0.369437E-08  | 0.356902E-09  | -0.296362E-11 | 0.206344E-09  |  |
|                 | -0.290729E-09 | -0.460727E-10 | 0.486156E-09  | 0.758867E-10  | 0.743654E-11  | 0.195080E-08  | -0.287463E-08 | 0.131747E-08  | 0.124716E-10  |  |
|                 | 0.105470E-08  | -0.664622E-09 | 0.310891E-09  | -0.952384E-09 | 0.813227E-09  | 0.250035E-08  |               |               |               |  |

**Table S26:** Anharmonic potential parameters  $\frac{\sqrt{h^3 c^3 \omega_j^2 \omega_l / E_h}}{N} \frac{\partial^3 V_{\text{BO}}}{\partial q_i^2 \partial q_j}$  (where  $N = 2$  for  $i \neq j$  and  $N = 6$  for  $i = j$ ) for  $\text{Cp}^{85}\text{Re}(\text{CH}_3)(\text{CO})(\text{NO})$ . B3LYP/cc-pV5Z,cc-pwCVQZ-PP level harmonic force field was utilised for the anharmonic calculation at B3LYP level with (12s11p10d8f)[8s7p6d4f] contraction on Re atom and cc-pVDZ basis set for H, C, N and O atoms. Values are determined by the GAUSSIAN package. (continued).

| Mode            | VBO           |               |               |               |               |               |               |               |               |               |
|-----------------|---------------|---------------|---------------|---------------|---------------|---------------|---------------|---------------|---------------|---------------|
| V <sub>43</sub> | -0.715011E-10 | 0.820583E-10  | -0.816839E-10 | 0.973311E-10  | 0.208604E-09  | -0.278423E-09 | -0.387133E-09 | 0.650117E-08  | -0.127514E-09 | -0.127514E-09 |
|                 | -0.929814E-09 | 0.535540E-10  | -0.799615E-09 | 0.581246E-09  | -0.317568E-09 | -0.123106E-08 | -0.219691E-08 | -0.428531E-08 | -0.115310E-08 | -0.115310E-08 |
|                 | -0.500282E-09 | 0.546707E-09  | -0.223624E-09 | 0.256068E-08  | 0.133036E-08  | -0.100924E-08 | -0.115881E-08 | 0.158314E-08  | 0.912282E-09  | 0.912282E-09  |
|                 | 0.272893E-08  | -0.389728E-09 | 0.282192E-09  | -0.471066E-08 | 0.431212E-08  | -0.659534E-08 | 0.119641E-09  | 0.585967E-10  | 0.327198E-08  | 0.327198E-08  |
| V <sub>42</sub> | 0.200862E-08  | -0.626582E-09 | 0.177439E-08  | 0.205400E-10  | 0.890413E-10  | 0.143263E-08  | -0.211668E-08 | 0.424240E-09  | -0.495435E-09 | -0.495435E-09 |
|                 | 0.111663E-09  | -0.941731E-08 | -0.335773E-08 | 0.185768E-08  | 0.405435E-08  | 0.961077E-08  |               |               |               |               |
|                 | -0.137006E-09 | -0.228965E-10 | -0.195166E-09 | 0.728485E-10  | 0.143682E-09  | 0.627155E-10  | -0.173301E-09 | 0.721861E-08  | 0.141298E-09  | 0.141298E-09  |
|                 | -0.649288E-09 | -0.392956E-09 | -0.686638E-10 | -0.452009E-09 | 0.455755E-09  | 0.110463E-08  | 0.257607E-08  | 0.317267E-08  | 0.878368E-09  | 0.878368E-09  |
| V <sub>41</sub> | 0.520704E-09  | 0.706511E-09  | -0.278687E-09 | 0.584743E-09  | 0.377354E-10  | 0.129811E-08  | 0.120774E-08  | -0.224535E-08 | -0.140535E-08 | -0.140535E-08 |
|                 | -0.104942E-08 | 0.115796E-08  | -0.643810E-09 | 0.288481E-08  | -0.389642E-08 | -0.711118E-08 | 0.245735E-09  | 0.656724E-10  | -0.471327E-08 | -0.471327E-08 |
|                 | -0.243095E-08 | -0.135192E-09 | 0.106614E-08  | -0.759480E-09 | -0.116203E-09 | 0.109089E-08  | -0.176696E-08 | 0.268862E-08  | 0.562260E-09  | 0.562260E-09  |
|                 | 0.569550E-09  | 0.571394E-08  | 0.543171E-08  | -0.355382E-08 | 0.144932E-08  | 0.800775E-08  |               |               |               |               |
| V <sub>40</sub> | -0.984158E-10 | 0.925370E-10  | 0.447678E-09  | -0.106660E-09 | -0.133277E-09 | -0.321708E-09 | -0.177914E-09 | -0.207156E-10 | -0.805908E-10 | -0.805908E-10 |
|                 | -0.111708E-08 | -0.461464E-09 | 0.372183E-08  | -0.403316E-08 | 0.120226E-08  | -0.695099E-09 | -0.191629E-08 | 0.120040E-08  | -0.121427E-08 | -0.121427E-08 |
|                 | 0.511710E-08  | 0.738868E-09  | 0.325928E-09  | 0.340218E-09  | 0.561836E-09  | 0.405570E-09  | 0.342176E-09  | 0.288864E-09  | -0.843164E-10 | -0.843164E-10 |
|                 | 0.254245E-09  | 0.189701E-09  | -0.194902E-09 | -0.191439E-09 | 0.522624E-10  | 0.473510E-09  | -0.495619E-09 | 0.159546E-10  | 0.354728E-09  | 0.354728E-09  |
| V <sub>39</sub> | -0.107568E-09 | -0.416975E-10 | -0.109085E-09 | -0.672088E-09 | 0.585679E-09  | 0.127004E-07  | -0.977508E-07 | 0.575175E-08  | 0.773673E-09  | 0.773673E-09  |
|                 | -0.729610E-09 | -0.665246E-10 | 0.151799E-08  | -0.461001E-09 | 0.658321E-09  | 0.144195E-08  |               |               |               |               |
|                 | -0.154942E-09 | 0.152319E-09  | 0.413292E-09  | -0.238337E-09 | 0.702011E-09  | 0.208065E-09  | 0.145585E-09  | -0.139375E-08 | 0.508777E-09  | 0.508777E-09  |
|                 | -0.913429E-09 | -0.304122E-08 | -0.776405E-08 | 0.287293E-08  | -0.312429E-08 | 0.259705E-09  | -0.119215E-08 | 0.328680E-08  | -0.151356E-08 | -0.151356E-08 |
| V <sub>38</sub> | -0.233989E-09 | -0.295525E-08 | -0.520382E-09 | -0.130725E-08 | 0.119238E-08  | 0.574261E-09  | -0.584708E-10 | 0.281492E-09  | -0.259252E-10 | -0.259252E-10 |
|                 | -0.419798E-09 | 0.100059E-08  | 0.136568E-09  | 0.139826E-09  | -0.221090E-10 | -0.142785E-09 | 0.192883E-08  | 0.923387E-11  | 0.406635E-10  | 0.406635E-10  |
|                 | -0.116266E-09 | 0.189994E-09  | 0.111195E-09  | 0.673027E-11  | 0.216321E-09  | 0.187289E-08  | -0.217919E-07 | 0.104880E-08  | 0.349957E-09  | 0.349957E-09  |
|                 | 0.143491E-08  | 0.133379E-09  | 0.107046E-09  | -0.120870E-09 | 0.169911E-10  | 0.180584E-09  | -0.167140E-07 | 0.238746E-08  | 0.210736E-09  | 0.210736E-09  |
| V <sub>37</sub> | -0.195042E-09 | -0.235604E-09 | -0.263021E-09 | 0.247112E-09  | 0.409233E-09  | 0.667612E-09  | 0.184455E-09  | -0.223794E-10 | 0.957970E-09  | 0.957970E-09  |
|                 | -0.514157E-09 | -0.173276E-08 | 0.101502E-08  | -0.219183E-08 | 0.118277E-08  | 0.204325E-08  | -0.145617E-08 | 0.835716E-09  | -0.205414E-08 | -0.205414E-08 |
|                 | 0.220842E-08  | 0.252830E-09  | -0.542331E-10 | 0.256970E-08  | 0.728010E-09  | -0.266223E-10 | 0.644851E-09  | 0.307491E-09  | -0.444569E-09 | -0.444569E-09 |
|                 | 0.254331E-10  | 0.452583E-09  | -0.696349E-10 | -0.169476E-09 | -0.256929E-09 | 0.406814E-09  | -0.397271E-09 | 0.406291E-10  | -0.294364E-09 | -0.294364E-09 |
| V <sub>36</sub> | -0.484444E-09 | 0.224069E-09  | 0.334418E-10  | -0.929838E-09 | -0.265568E-09 | 0.597099E-08  | -0.103210E-06 | 0.117954E-07  | -0.648984E-09 | -0.648984E-09 |
|                 | 0.414490E-10  | -0.168031E-09 | 0.340505E-09  | 0.423954E-09  | 0.284016E-09  | 0.821034E-10  |               |               |               |               |
|                 | -0.404079E-09 | 0.197795E-09  | 0.351855E-09  | 0.188327E-09  | 0.325954E-10  | 0.457504E-09  | 0.832890E-09  | 0.179974E-08  | 0.245131E-08  | 0.245131E-08  |
|                 | -0.271134E-10 | -0.931106E-09 | 0.123052E-08  | -0.264627E-08 | -0.139009E-08 | 0.422400E-09  | -0.227280E-08 | 0.172897E-08  | -0.141200E-08 | -0.141200E-08 |
| V <sub>35</sub> | 0.338094E-08  | 0.187316E-08  | 0.990817E-10  | 0.817885E-10  | 0.886918E-10  | -0.380644E-09 | 0.100380E-08  | 0.746594E-09  | -0.797399E-09 | -0.797399E-09 |
|                 | 0.133274E-08  | -0.245938E-09 | -0.436332E-09 | -0.151975E-08 | -0.216862E-09 | -0.108769E-08 | -0.143654E-09 | -0.504785E-10 | 0.761914E-09  | 0.761914E-09  |
|                 | -0.999134E-09 | 0.717713E-09  | 0.141515E-08  | -0.108990E-09 | -0.144457E-08 | 0.343807E-07  | -0.524102E-07 | 0.513013E-08  | 0.198249E-08  | 0.198249E-08  |
|                 | 0.499535E-08  | 0.243964E-09  | 0.141388E-08  | -0.186533E-08 | -0.127103E-08 | 0.240122E-08  |               |               |               |               |
| V <sub>34</sub> | 0.208998E-10  | 0.222045E-09  | 0.167967E-09  | -0.326059E-09 | 0.493125E-11  | 0.305352E-09  | 0.634929E-09  | 0.234506E-08  | -0.177289E-08 | -0.177289E-08 |
|                 | -0.109283E-08 | -0.974688E-09 | -0.718072E-09 | 0.283096E-09  | 0.120184E-08  | -0.168872E-08 | 0.140140E-08  | -0.189774E-08 | 0.307927E-08  | 0.307927E-08  |
|                 | -0.446441E-08 | 0.753928E-09  | -0.131240E-08 | 0.573967E-08  | 0.243106E-08  | -0.289440E-09 | 0.409884E-09  | -0.915008E-09 | 0.314989E-09  | 0.314989E-09  |
|                 | 0.184333E-09  | -0.360831E-09 | 0.433781E-08  | 0.695310E-09  | -0.950864E-10 | -0.789311E-08 | 0.132587E-10  | 0.325354E-09  | -0.244533E-08 | -0.244533E-08 |
| V <sub>33</sub> | 0.159779E-08  | -0.583274E-10 | 0.125957E-07  | 0.610425E-09  | 0.228676E-09  | 0.106560E-07  | -0.417545E-08 | 0.143065E-08  | 0.459838E-09  | 0.459838E-09  |
|                 | -0.530946E-09 | -0.244794E-08 | -0.245986E-08 | -0.293502E-08 | -0.119619E-08 | 0.219042E-09  |               |               |               |               |

**Table S26:** Anharmonic potential parameters  $\frac{\sqrt{h^3 c \phi_j^2 \omega_j / E_h}}{N} \frac{\partial^3 V_{\text{ReO}}}{\partial q_i^2 \partial q_j}$  (where  $N = 2$  for  $i \neq j$  and  $N = 6$  for  $i = j$ ) for  $\text{Cp}^{85}\text{Re}(\text{CH}_3)(\text{CO})(\text{NO})$ . B3LYP/cc-pV5Z,cc-pwCVQZ-PP level harmonic force field was utilised for the anharmonic calculation at B3LYP level with (12s11p10d8f)[8s7p6d4f] contraction on Re atom and cc-pVDZ basis set for H, C, N and O atoms. Values are determined by the GAUSSIAN package. (continued).

| Mode            | VBO           |               |               |               |               |               |               |               |               |  |
|-----------------|---------------|---------------|---------------|---------------|---------------|---------------|---------------|---------------|---------------|--|
| V <sub>35</sub> | 0.929619E-10  | 0.652619E-09  | 0.655737E-09  | -0.202781E-09 | -0.202883E-09 | -0.233247E-09 | 0.391038E-11  | 0.222306E-08  | -0.221462E-09 |  |
|                 | 0.141450E-08  | -0.203711E-08 | -0.125040E-08 | 0.934704E-09  | 0.845202E-09  | -0.434494E-09 | 0.619255E-09  | -0.752718E-09 | -0.22104E-08  |  |
|                 | -0.277781E-08 | 0.256738E-09  | -0.713993E-10 | 0.457284E-08  | 0.150136E-08  | 0.149097E-08  | 0.129876E-08  | -0.671869E-09 | 0.133997E-08  |  |
|                 | 0.200153E-08  | 0.242048E-08  | -0.162844E-08 | -0.533031E-09 | 0.987036E-09  | -0.668495E-08 | -0.169129E-09 | -0.110240E-09 | -0.296203E-08 |  |
| V <sub>34</sub> | -0.304127E-09 | -0.662716E-08 | 0.815351E-08  | -0.273338E-09 | -0.234184E-09 | 0.159555E-07  | -0.112275E-07 | 0.795927E-09  | 0.304608E-09  |  |
|                 | 0.752182E-09  | 0.872171E-09  | -0.336043E-08 | 0.893024E-09  | 0.419021E-08  | 0.336320E-08  |               |               |               |  |
|                 | 0.191585E-09  | 0.474579E-09  | 0.379532E-09  | -0.106234E-08 | 0.435248E-09  | 0.914870E-10  | 0.212883E-09  | 0.100155E-08  | 0.108633E-08  |  |
|                 | -0.127020E-09 | -0.248198E-08 | 0.377825E-09  | -0.403131E-09 | 0.452328E-10  | 0.423335E-09  | 0.455574E-08  | -0.430692E-08 | 0.358778E-08  |  |
| V <sub>33</sub> | -0.102574E-07 | -0.118414E-08 | -0.342145E-09 | 0.438679E-08  | 0.239954E-09  | 0.677749E-09  | 0.736505E-09  | 0.229592E-09  | -0.755407E-09 |  |
|                 | 0.166956E-08  | -0.214414E-08 | -0.133050E-08 | -0.865647E-09 | -0.129836E-08 | -0.489051E-08 | -0.127745E-09 | -0.136625E-09 | -0.891688E-09 |  |
|                 | 0.969808E-10  | 0.718192E-08  | 0.425319E-08  | -0.291474E-09 | -0.536413E-09 | 0.209518E-07  | -0.921687E-08 | 0.375152E-08  | 0.174749E-08  |  |
|                 | 0.173973E-09  | -0.186195E-08 | 0.428291E-08  | 0.555615E-08  | 0.131825E-08  | 0.315908E-08  |               |               |               |  |
| V <sub>32</sub> | -0.505922E-10 | -0.118278E-08 | -0.697395E-09 | 0.121235E-08  | -0.888680E-09 | -0.174725E-09 | 0.768502E-10  | -0.197257E-08 | 0.374656E-09  |  |
|                 | -0.339267E-09 | 0.265531E-08  | -0.390213E-08 | 0.130986E-08  | -0.132984E-08 | -0.206600E-09 | 0.732216E-08  | -0.737544E-08 | 0.113299E-07  |  |
|                 | -0.173516E-08 | -0.141581E-08 | 0.388224E-10  | 0.132908E-08  | -0.511562E-09 | -0.339081E-09 | 0.430879E-09  | -0.420197E-09 | 0.137201E-09  |  |
|                 | -0.371929E-09 | 0.161681E-09  | -0.440187E-09 | 0.791565E-09  | 0.792446E-10  | -0.584626E-10 | -0.732524E-09 | 0.104738E-09  | -0.137093E-08 |  |
| V <sub>31</sub> | 0.113543E-08  | -0.241964E-09 | 0.448962E-09  | 0.821880E-09  | -0.872165E-09 | 0.455304E-07  | -0.280043E-07 | 0.653419E-08  | 0.350231E-08  |  |
|                 | 0.373605E-08  | -0.500751E-10 | 0.142920E-08  | 0.192978E-08  | -0.724228E-09 | 0.213848E-08  |               |               |               |  |
|                 | -0.282023E-09 | 0.724323E-09  | 0.153912E-08  | 0.121153E-08  | 0.448896E-09  | 0.219852E-08  | -0.907157E-09 | -0.316920E-09 | 0.199166E-08  |  |
|                 | 0.467536E-09  | -0.195118E-08 | -0.628435E-08 | -0.963208E-08 | 0.147205E-08  | 0.492796E-08  | 0.179454E-08  | -0.305840E-08 | -0.420028E-09 |  |
| V <sub>30</sub> | -0.761240E-09 | 0.209820E-08  | 0.372391E-08  | -0.178182E-08 | 0.662952E-09  | -0.710839E-09 | 0.124406E-08  | 0.651831E-09  | 0.781802E-10  |  |
|                 | -0.538783E-09 | -0.569588E-09 | -0.241247E-08 | -0.464203E-10 | -0.171260E-08 | -0.140619E-08 | -0.460438E-09 | 0.740573E-09  | 0.217532E-10  |  |
|                 | -0.103454E-08 | -0.563516E-09 | -0.443018E-09 | -0.366478E-09 | 0.605847E-09  | 0.564010E-09  | -0.581526E-08 | 0.346951E-09  | -0.247454E-08 |  |
|                 | -0.193958E-08 | 0.694813E-09  | -0.210781E-09 | -0.168863E-07 | 0.537795E-07  | 0.216311E-08  | -0.207754E-08 | 0.526112E-06  | -0.197329E-06 |  |
| V <sub>29</sub> | 0.620354E-07  | 0.294873E-07  | 0.288827E-07  | 0.447491E-09  | -0.209809E-07 | 0.615776E-07  |               |               |               |  |
|                 | -0.625248E-09 | -0.357930E-09 | 0.908468E-10  | 0.368691E-09  | -0.456250E-10 | 0.377075E-10  | -0.522682E-09 | 0.117359E-08  | 0.898507E-09  |  |
|                 | -0.877188E-09 | -0.182892E-08 | 0.570115E-09  | 0.209567E-09  | 0.174950E-08  | 0.229786E-08  | -0.432143E-09 | -0.138799E-09 | -0.715666E-09 |  |
|                 | -0.107165E-08 | 0.109642E-08  | -0.365653E-09 | -0.116017E-08 | 0.186975E-08  | -0.186420E-08 | -0.224721E-08 | 0.350624E-08  | -0.238207E-08 |  |
| V <sub>28</sub> | -0.314139E-08 | 0.721180E-09  | -0.103654E-09 | 0.719691E-10  | -0.683029E-09 | -0.422053E-08 | -0.110702E-09 | -0.478784E-09 | -0.838642E-08 |  |
|                 | -0.308945E-08 | 0.192090E-08  | -0.105782E-08 | -0.644011E-09 | -0.215978E-08 | 0.357672E-08  | -0.217489E-08 | 0.182321E-07  | 0.101389E-07  |  |
|                 | 0.918231E-09  | 0.171135E-06  | 0.179856E-06  | -0.439023E-06 | 0.190843E-06  | 0.452287E-06  |               |               |               |  |
|                 | 0.385128E-10  | 0.369870E-09  | -0.319806E-09 | 0.743292E-10  | 0.671722E-09  | -0.277159E-09 | -0.404884E-09 | 0.642572E-09  | 0.120202E-09  |  |
| V <sub>27</sub> | -0.255728E-09 | 0.541566E-09  | -0.875619E-09 | -0.150300E-08 | -0.771134E-09 | 0.360776E-08  | 0.129658E-08  | 0.282921E-08  | 0.124426E-08  |  |
|                 | 0.160835E-08  | -0.117182E-10 | -0.137665E-08 | -0.389913E-09 | 0.489628E-09  | 0.318542E-10  | 0.194972E-09  | 0.109231E-08  | 0.981498E-09  |  |
|                 | -0.745379E-09 | -0.187184E-08 | 0.213522E-08  | -0.212192E-08 | 0.283674E-08  | 0.267988E-08  | -0.555154E-09 | 0.474703E-09  | -0.136426E-07 |  |
|                 | 0.157637E-08  | -0.395838E-09 | -0.952872E-09 | -0.479395E-08 | 0.479107E-08  | 0.154141E-08  | -0.439000E-08 | 0.622880E-07  | -0.159531E-07 |  |
| V <sub>26</sub> | -0.306000E-08 | 0.154234E-06  | 0.298150E-06  | 0.146437E-06  | -0.165012E-06 | 0.465711E-06  |               |               |               |  |
|                 | 0.299913E-09  | 0.235307E-09  | -0.223329E-10 | 0.965170E-10  | 0.112728E-09  | -0.375459E-09 | -0.719576E-09 | 0.521001E-09  | 0.747568E-09  |  |
|                 | 0.951590E-09  | 0.103536E-08  | -0.131924E-08 | 0.712930E-09  | 0.724974E-10  | -0.759460E-09 | -0.284863E-08 | -0.369985E-08 | -0.433171E-10 |  |
|                 | 0.785435E-09  | -0.914772E-10 | -0.388385E-09 | 0.175358E-08  | 0.144393E-08  | -0.755909E-10 | -0.118134E-08 | 0.192564E-08  | -0.359671E-08 |  |
| V <sub>25</sub> | -0.364716E-08 | 0.378987E-08  | -0.375400E-08 | 0.774162E-08  | -0.298160E-08 | 0.637517E-08  | 0.273455E-09  | 0.262244E-09  | 0.910445E-09  |  |
|                 | 0.312170E-08  | 0.165948E-08  | 0.973727E-09  | -0.335151E-09 | -0.464765E-09 | 0.546625E-09  | -0.370381E-08 | 0.502811E-08  | -0.187245E-08 |  |
|                 | -0.242877E-09 | -0.574090E-07 | 0.509644E-07  | 0.115530E-06  | -0.320459E-08 | 0.317549E-06  |               |               |               |  |

**Table S26:** Anharmonic potential parameters  $\frac{\sqrt{h^3 c^3 \phi_j^2 \omega_j / E_h^3}}{N} \frac{\partial^3 V_{\text{B3LYP}}}{\partial q_i^2 \partial q_j}$  (where  $N = 2$  for  $i \neq j$  and  $N = 6$  for  $i = j$ ) for  $\text{Cp}^{85}\text{Re}(\text{CH}_3)(\text{CO})(\text{NO})$ . B3LYP/cc-pV5Z,cc-pwCVQZ-PP level harmonic force field was utilised for the anharmonic calculation at B3LYP level with (12s11p10d8f)[8s7p6d4f] contraction on Re atom and cc-pVDZ basis set for H, C, N and O atoms. Values are determined by the GAUSSIAN package. (continued).

| Mode            | VBO           |               |               |               |               |               |               |               |               |  |
|-----------------|---------------|---------------|---------------|---------------|---------------|---------------|---------------|---------------|---------------|--|
| v <sub>27</sub> | 0.189684E-10  | -0.146746E-09 | -0.209463E-09 | -0.705069E-10 | 0.116371E-09  | -0.232771E-09 | -0.122611E-09 | 0.868375E-09  | 0.324336E-10  |  |
|                 | 0.249887E-09  | 0.489848E-09  | -0.424165E-09 | 0.565707E-09  | 0.506218E-09  | -0.155815E-08 | 0.449237E-08  | 0.256424E-09  | -0.157639E-08 |  |
|                 | 0.721377E-09  | -0.721865E-09 | 0.758079E-09  | -0.136453E-08 | -0.275431E-08 | 0.242625E-08  | -0.108939E-08 | 0.112295E-08  | 0.796582E-08  |  |
|                 | -0.478565E-09 | 0.242671E-08  | -0.247427E-08 | 0.790870E-08  | -0.312753E-08 | 0.884081E-08  | 0.261874E-09  | -0.152190E-09 | 0.193640E-08  |  |
| v <sub>26</sub> | 0.346023E-10  | -0.134598E-08 | 0.887444E-09  | -0.524024E-09 | 0.120540E-08  | 0.211197E-08  | -0.247759E-08 | 0.851111E-08  | -0.119607E-08 |  |
|                 | 0.113260E-08  | -0.115075E-06 | -0.406850E-07 | -0.338452E-07 | -0.112636E-06 | 0.267475E-06  |               |               |               |  |
|                 | 0.753665E-10  | 0.490297E-10  | 0.881769E-10  | -0.322712E-10 | -0.315906E-10 | -0.509429E-10 | -0.593260E-10 | -0.120906E-09 | 0.157142E-09  |  |
|                 | 0.297300E-09  | -0.135551E-09 | -0.412263E-09 | -0.147825E-09 | 0.287581E-09  | 0.345087E-09  | 0.213827E-09  | 0.416940E-09  | 0.109312E-09  |  |
| v <sub>25</sub> | 0.128231E-09  | -0.575376E-10 | -0.137194E-09 | -0.155975E-08 | -0.261667E-09 | -0.134747E-08 | 0.412269E-09  | -0.171715E-10 | -0.394427E-09 |  |
|                 | 0.120007E-08  | 0.856945E-09  | -0.341623E-08 | 0.289829E-08  | 0.136603E-09  | 0.191004E-07  | -0.288949E-10 | 0.154103E-09  | 0.639108E-09  |  |
|                 | -0.750518E-09 | -0.967656E-09 | -0.191706E-08 | 0.127086E-09  | -0.275651E-10 | 0.656508E-09  | -0.431877E-09 | 0.375347E-09  | -0.782730E-10 |  |
|                 | 0.119569E-09  | -0.167044E-07 | 0.106058E-07  | -0.312102E-07 | -0.294817E-07 | 0.586404E-07  |               |               |               |  |
| v <sub>24</sub> | -0.102813E-09 | -0.426644E-09 | -0.779151E-09 | -0.272351E-09 | -0.648335E-10 | 0.165243E-09  | 0.695225E-09  | -0.981373E-10 | 0.253149E-08  |  |
|                 | 0.930770E-09  | 0.197227E-09  | -0.532907E-09 | 0.425856E-09  | 0.478188E-10  | -0.388432E-08 | -0.836484E-09 | 0.104620E-08  | 0.469788E-09  |  |
|                 | -0.340628E-09 | -0.642089E-09 | -0.367532E-09 | -0.200464E-08 | 0.768046E-09  | 0.169376E-08  | 0.132609E-08  | -0.127431E-08 | 0.116465E-09  |  |
|                 | 0.445129E-09  | -0.223977E-08 | -0.117130E-07 | -0.445118E-08 | 0.251696E-08  | 0.880674E-08  | 0.298194E-09  | 0.111704E-09  | 0.802196E-08  |  |
| v <sub>23</sub> | 0.693062E-10  | 0.157009E-09  | 0.106035E-07  | 0.370768E-08  | 0.100969E-08  | 0.841336E-08  | 0.449285E-09  | 0.109747E-09  | 0.102444E-07  |  |
|                 | -0.294714E-08 | -0.337550E-10 | -0.194180E-08 | 0.107299E-08  | -0.622839E-08 | 0.146038E-08  | -0.177708E-08 | 0.182216E-08  | -0.443616E-09 |  |
|                 | 0.428408E-08  | -0.937681E-07 | -0.268668E-06 | 0.151973E-06  | 0.465857E-06  | 0.535821E-06  |               |               |               |  |
|                 | 0.302347E-09  | 0.124380E-09  | 0.476922E-09  | 0.371737E-09  | -0.875767E-10 | -0.157942E-08 | -0.347594E-08 | 0.158678E-08  | -0.125552E-08 |  |
| v <sub>22</sub> | -0.788858E-09 | -0.189440E-09 | -0.609254E-09 | -0.830214E-09 | 0.445086E-09  | 0.152747E-08  | -0.257513E-09 | 0.934123E-10  | -0.820742E-11 |  |
|                 | -0.396702E-09 | 0.840317E-09  | 0.115608E-08  | -0.655546E-09 | -0.105279E-08 | 0.531505E-09  | 0.723651E-09  | -0.523815E-08 | 0.127054E-09  |  |
|                 | 0.109579E-08  | -0.182007E-08 | 0.739666E-09  | -0.518005E-09 | 0.330431E-09  | -0.262078E-08 | -0.225641E-08 | -0.217843E-07 | -0.317417E-09 |  |
|                 | -0.631356E-08 | 0.310419E-08  | -0.174087E-07 | 0.499980E-07  | -0.310334E-08 | 0.478942E-07  | -0.122614E-09 | 0.546278E-09  | -0.531610E-07 |  |
| v <sub>21</sub> | 0.159168E-07  | -0.735301E-09 | 0.729560E-08  | -0.233368E-08 | -0.613862E-09 | -0.265792E-09 | 0.660602E-10  | 0.419413E-09  | -0.312571E-09 |  |
|                 | 0.357208E-09  | -0.348372E-07 | -0.811157E-07 | -0.319091E-07 | -0.516924E-07 | 0.217596E-06  |               |               |               |  |
|                 | -0.242641E-09 | -0.735590E-10 | -0.248297E-10 | 0.221151E-10  | 0.146013E-09  | 0.143706E-09  | 0.744243E-10  | -0.223977E-08 | 0.809426E-09  |  |
|                 | 0.424644E-09  | -0.310608E-09 | 0.323573E-09  | -0.511720E-09 | -0.378680E-09 | 0.126365E-08  | -0.916759E-09 | 0.191277E-08  | 0.951613E-09  |  |
| v <sub>20</sub> | -0.772257E-09 | 0.100293E-08  | -0.823007E-09 | 0.174397E-08  | -0.115879E-08 | 0.126869E-08  | -0.522697E-10 | 0.237289E-07  | -0.106769E-08 |  |
|                 | 0.411803E-09  | 0.463233E-09  | -0.167422E-08 | -0.241375E-07 | -0.331393E-08 | 0.516965E-07  | 0.452309E-09  | -0.206121E-09 | 0.302684E-07  |  |
|                 | -0.177677E-07 | 0.761669E-09  | 0.548216E-08  | 0.748618E-09  | -0.644280E-10 | 0.853741E-09  | -0.930998E-09 | 0.532495E-09  | 0.120621E-09  |  |
|                 | -0.497267E-09 | 0.351364E-07  | 0.173362E-06  | -0.420429E-07 | 0.134958E-07  | 0.210516E-06  |               |               |               |  |
| v <sub>19</sub> | -0.152151E-09 | -0.143244E-09 | -0.780569E-10 | -0.219488E-10 | 0.522831E-10  | 0.644031E-10  | 0.174539E-09  | -0.210636E-08 | 0.189937E-08  |  |
|                 | 0.592085E-09  | -0.711530E-10 | -0.651151E-10 | 0.299614E-09  | 0.448197E-09  | -0.683424E-09 | 0.259522E-09  | 0.335274E-09  | -0.553454E-09 |  |
|                 | 0.505806E-11  | -0.638815E-09 | 0.182077E-09  | 0.365527E-09  | 0.100343E-09  | -0.218060E-08 | 0.228880E-08  | -0.586274E-08 | 0.669742E-09  |  |
|                 | -0.206762E-08 | -0.102872E-07 | -0.349355E-07 | 0.340722E-08  | 0.103669E-08  | 0.424661E-07  | 0.416034E-09  | 0.859533E-10  | -0.672566E-08 |  |
| v <sub>18</sub> | 0.105043E-07  | 0.144235E-07  | 0.302037E-07  | -0.239888E-08 | -0.341559E-09 | 0.413586E-09  | -0.834145E-10 | 0.256270E-09  | -0.138585E-09 |  |
|                 | -0.309843E-09 | -0.100595E-06 | 0.165291E-07  | -0.154248E-06 | -0.144467E-06 | 0.226990E-06  |               |               |               |  |
|                 | 0.277966E-09  | 0.106995E-09  | 0.122383E-09  | 0.694599E-10  | -0.613505E-10 | -0.361186E-09 | -0.652768E-09 | -0.102130E-08 | -0.119630E-08 |  |
|                 | -0.584991E-10 | 0.386849E-09  | -0.310717E-10 | -0.709474E-10 | 0.119014E-09  | 0.738242E-09  | 0.582808E-09  | -0.332033E-10 | 0.272238E-09  |  |
| v <sub>17</sub> | 0.703050E-09  | 0.652136E-10  | 0.264489E-09  | -0.454118E-09 | -0.234112E-09 | 0.234866E-08  | -0.102505E-08 | -0.333702E-08 | 0.460868E-09  |  |
|                 | 0.257604E-09  | 0.732414E-08  | 0.329344E-07  | -0.285288E-09 | 0.142325E-08  | 0.422034E-07  | -0.373871E-09 | 0.319317E-09  | 0.134177E-07  |  |
|                 | -0.209889E-08 | -0.132371E-07 | -0.351094E-07 | 0.218241E-08  | 0.564896E-09  | -0.259815E-10 | -0.613378E-09 | 0.397657E-09  | -0.539485E-09 |  |
|                 | 0.104059E-08  | 0.457838E-08  | -0.120719E-07 | 0.963582E-07  | 0.192571E-06  | 0.290739E-06  |               |               |               |  |

**Table S26:** Anharmonic potential parameters  $\frac{\sqrt{h^3 c^3 \phi_j^2 \omega_j / E_h}}{N} \frac{\partial^3 V_{\text{ReO}}}{\partial q_i^2 \partial q_j}$  (where  $N = 2$  for  $i \neq j$  and  $N = 6$  for  $i = j$ ) for  $\text{Cp}^{85}\text{Re}(\text{CH}_3)(\text{CO})(\text{NO})$ . B3LYP/cc-pV5Z,cc-pwCVQZ-PP level harmonic force field was utilised for the anharmonic calculation at B3LYP level with (12s11p10d8f)[8s7p6d4f] contraction on Re atom and cc-pVDZ basis set for H, C, N and O atoms. Values are determined by the GAUSSIAN package. (continued).

| Mode            | VBO           |               |               |               |               |               |               |               |               |  |
|-----------------|---------------|---------------|---------------|---------------|---------------|---------------|---------------|---------------|---------------|--|
| V <sub>19</sub> | -0.674884E-10 | -0.572151E-10 | 0.157684E-09  | 0.469726E-10  | 0.879065E-11  | -0.151660E-09 | -0.327653E-09 | -0.422086E-08 | 0.751964E-09  |  |
|                 | 0.939661E-09  | 0.922257E-10  | -0.312828E-09 | 0.173549E-09  | 0.323212E-09  | 0.145480E-09  | -0.362232E-09 | -0.630118E-09 | -0.656011E-10 |  |
|                 | 0.297433E-09  | -0.103476E-08 | 0.617505E-10  | -0.515661E-08 | -0.181268E-08 | -0.178578E-08 | -0.337583E-09 | 0.395277E-08  | -0.158147E-08 |  |
|                 | -0.487512E-08 | 0.182283E-08  | -0.407546E-08 | 0.115214E-07  | -0.181817E-08 | 0.412330E-07  | -0.766126E-10 | -0.117123E-09 | 0.916370E-08  |  |
| V <sub>18</sub> | -0.565102E-08 | 0.103143E-08  | -0.884328E-08 | 0.967316E-09  | 0.166327E-10  | 0.594514E-10  | -0.248458E-10 | 0.690522E-10  | -0.704352E-10 |  |
|                 | -0.836893E-11 | -0.145123E-08 | 0.807617E-08  | -0.426857E-08 | 0.105341E-08  | 0.424042E-07  |               |               |               |  |
|                 | -0.122115E-09 | 0.512599E-10  | 0.768987E-09  | 0.491113E-09  | 0.435222E-09  | 0.995717E-09  | -0.711924E-09 | -0.130863E-08 | 0.859780E-09  |  |
|                 | 0.536230E-09  | -0.503673E-08 | -0.150243E-07 | -0.242511E-07 | 0.563670E-08  | -0.238921E-08 | 0.560629E-09  | -0.910931E-09 | -0.164365E-09 |  |
| V <sub>17</sub> | -0.867388E-09 | 0.312662E-08  | -0.374042E-08 | 0.345534E-09  | -0.178880E-08 | 0.178097E-08  | -0.249404E-08 | -0.239665E-09 | -0.540973E-09 |  |
|                 | 0.311671E-09  | 0.293689E-09  | 0.297642E-08  | -0.239199E-09 | 0.388446E-09  | 0.996535E-09  | 0.630528E-07  | -0.398267E-09 | -0.808676E-09 |  |
|                 | 0.199509E-08  | -0.545774E-10 | 0.135101E-08  | 0.407925E-08  | -0.952738E-08 | 0.706143E-08  | -0.711616E-08 | 0.526629E-06  | 0.490071E-07  |  |
|                 | 0.105419E-06  | -0.408346E-09 | -0.521690E-09 | 0.842853E-11  | 0.559831E-09  | 0.198793E-09  |               |               |               |  |
| V <sub>16</sub> | 0.224344E-10  | -0.365156E-10 | -0.715825E-11 | 0.125360E-10  | 0.165574E-10  | -0.101178E-09 | -0.155277E-09 | -0.184095E-08 | 0.341706E-09  |  |
|                 | 0.252751E-09  | 0.149171E-09  | -0.131318E-09 | 0.183488E-10  | 0.553522E-10  | -0.628404E-10 | 0.799156E-10  | 0.344432E-09  | 0.205940E-10  |  |
|                 | -0.212527E-11 | -0.133132E-10 | -0.37760E-09  | 0.241862E-08  | 0.134179E-08  | 0.232318E-09  | 0.608040E-09  | -0.145758E-08 | -0.193890E-09 |  |
|                 | -0.587717E-09 | 0.690377E-09  | -0.288342E-08 | 0.263437E-08  | 0.118540E-09  | 0.234561E-07  | 0.577773E-10  | 0.780615E-10  | 0.399087E-09  |  |
| V <sub>15</sub> | -0.703761E-10 | 0.117015E-09  | -0.609675E-09 | -0.223409E-09 | -0.455638E-10 | 0.152103E-09  | -0.377909E-09 | 0.244366E-09  | -0.470846E-09 |  |
|                 | 0.347395E-09  | -0.544654E-07 | 0.262860E-07  | -0.554675E-07 | -0.426087E-08 | 0.399407E-06  |               |               |               |  |
|                 | 0.107506E-09  | -0.136856E-09 | 0.359797E-10  | -0.683050E-10 | 0.551070E-10  | -0.417565E-09 | -0.152420E-09 | -0.665827E-08 | 0.241920E-08  |  |
|                 | 0.455324E-08  | 0.534085E-09  | 0.131320E-09  | 0.415462E-11  | -0.672922E-09 | 0.353524E-09  | -0.123181E-08 | 0.141286E-08  | 0.127064E-08  |  |
| V <sub>14</sub> | 0.141158E-08  | -0.404204E-08 | -0.260413E-08 | -0.635348E-08 | 0.419024E-08  | -0.502849E-08 | 0.209338E-08  | 0.343428E-08  | -0.674619E-08 |  |
|                 | -0.590407E-08 | 0.653643E-07  | -0.900991E-07 | 0.339140E-08  | 0.712304E-08  | 0.166969E-06  | 0.151479E-08  | 0.133563E-08  | 0.446308E-08  |  |
|                 | -0.268651E-07 | -0.585692E-07 | 0.108996E-06  | -0.826172E-08 | -0.244378E-08 | -0.102844E-08 | 0.305405E-08  | 0.531050E-09  | -0.561358E-09 |  |
|                 | -0.246029E-09 | -0.878559E-08 | 0.331171E-07  | 0.210530E-07  | -0.184229E-06 | 0.224255E-06  | -0.224695E-09 | -0.421499E-08 | 0.953687E-09  |  |
| V <sub>13</sub> | -0.302351E-09 | 0.211781E-10  | 0.119236E-09  | 0.209769E-09  | 0.671195E-10  | 0.169729E-09  | -0.224695E-09 | -0.421499E-08 | 0.953687E-09  |  |
|                 | -0.913110E-09 | 0.134518E-09  | 0.768980E-09  | 0.175644E-09  | 0.189413E-08  | -0.249203E-09 | 0.917582E-09  | -0.947697E-09 | -0.184531E-08 |  |
|                 | 0.699769E-09  | 0.220233E-11  | 0.340122E-08  | -0.567737E-08 | -0.809052E-08 | -0.102269E-08 | -0.549742E-08 | 0.163547E-09  | 0.244212E-08  |  |
|                 | -0.854918E-08 | -0.566005E-07 | 0.417708E-07  | 0.374343E-07  | -0.768779E-08 | 0.177857E-06  | -0.151635E-08 | -0.145916E-08 | -0.588390E-08 |  |
| V <sub>12</sub> | 0.760362E-08  | 0.625743E-07  | -0.965508E-07 | 0.746954E-08  | 0.189399E-08  | -0.202213E-08 | 0.203211E-08  | -0.596205E-09 | 0.280126E-09  |  |
|                 | 0.105975E-08  | -0.122061E-07 | 0.713827E-07  | -0.105873E-06 | 0.115998E-06  | 0.200084E-06  |               |               |               |  |
|                 | 0.634540E-09  | 0.726546E-10  | 0.287042E-09  | -0.360364E-10 | -0.451869E-09 | -0.623194E-09 | -0.838927E-09 | -0.496511E-08 | -0.136466E-08 |  |
|                 | 0.407307E-09  | 0.819608E-09  | -0.824810E-09 | 0.671913E-09  | 0.103654E-08  | -0.964114E-09 | 0.330722E-08  | -0.695276E-09 | -0.246937E-09 |  |
| V <sub>11</sub> | 0.151354E-08  | -0.616171E-09 | 0.257249E-08  | -0.411088E-08 | 0.221566E-08  | -0.120631E-07 | -0.749818E-08 | -0.282101E-07 | 0.274958E-08  |  |
|                 | -0.672719E-09 | 0.274561E-08  | 0.249594E-07  | 0.194397E-07  | 0.172223E-07  | 0.112363E-06  | -0.873815E-09 | 0.946420E-09  | 0.782009E-09  |  |
|                 | 0.555954E-07  | -0.643664E-08 | -0.391093E-07 | 0.183184E-08  | 0.201007E-08  | -0.118394E-08 | -0.398584E-09 | -0.104559E-09 | -0.754644E-09 |  |
|                 | 0.153822E-08  | -0.593016E-07 | -0.191758E-06 | 0.586772E-08  | 0.639111E-07  | 0.280093E-06  |               |               |               |  |
| V <sub>10</sub> | -0.525829E-09 | -0.103751E-09 | 0.618374E-11  | 0.314596E-10  | 0.342693E-09  | 0.282136E-09  | 0.112316E-09  | -0.503978E-08 | 0.119341E-08  |  |
|                 | 0.474996E-09  | -0.677994E-09 | 0.482958E-09  | -0.929084E-09 | -0.513351E-09 | 0.227253E-08  | -0.298236E-08 | 0.276869E-08  | 0.170591E-08  |  |
|                 | -0.139440E-08 | 0.475389E-09  | -0.255648E-08 | 0.220068E-09  | -0.208723E-08 | 0.731590E-08  | 0.683347E-08  | 0.336789E-07  | -0.352634E-08 |  |
|                 | -0.307255E-08 | -0.495081E-08 | -0.633414E-08 | -0.147602E-07 | -0.108272E-07 | 0.110754E-06  | 0.894063E-09  | -0.771575E-09 | 0.744766E-07  |  |
| V <sub>9</sub>  | -0.663002E-07 | 0.128635E-07  | -0.831675E-09 | 0.342422E-08  | -0.794323E-09 | 0.123019E-08  | -0.543587E-09 | 0.212801E-08  | -0.161402E-09 |  |
|                 | -0.135555E-08 | -0.218404E-07 | 0.181603E-06  | -0.505557E-07 | 0.765339E-08  | 0.231128E-06  |               |               |               |  |
|                 | 0.160987E-09  | 0.224761E-09  | 0.464055E-09  | 0.508371E-09  | 0.348569E-09  | -0.147964E-08 | 0.327644E-09  | 0.108822E-08  | 0.237649E-09  |  |
|                 | 0.680418E-11  | 0.103024E-09  | -0.169905E-08 | -0.266540E-08 | 0.943117E-09  | 0.505752E-09  | 0.503608E-09  | -0.126845E-08 | 0.724630E-10  |  |
| V <sub>8</sub>  | -0.997205E-09 | 0.136077E-07  | -0.834509E-08 | -0.279506E-08 | -0.239933E-08 | 0.522472E-09  | -0.125732E-08 | -0.120127E-09 | -0.496539E-09 |  |
|                 | -0.145946E-08 | 0.211118E-09  | 0.215033E-10  | 0.830864E-09  | -0.266628E-09 | 0.420433E-09  | 0.347416E-07  | -0.520671E-10 | -0.320979E-08 |  |
|                 | 0.504212E-09  | -0.849945E-09 | 0.876206E-08  | 0.377316E-07  | 0.177864E-07  | -0.255184E-09 | 0.828888E-09  | 0.349169E-06  | 0.546111E-07  |  |
|                 | -0.152223E-06 | -0.430249E-09 | 0.205935E-09  | 0.277091E-09  | 0.122179E-08  | 0.164645E-08  |               |               |               |  |

**Table S26:** Anharmonic potential parameters  $\frac{\sqrt{h^3 c^3 \phi_j^2 \omega_j / E_h}}{N} \frac{\partial^3 V_{\text{ReO}}}{\partial q_i^2 \partial q_j}$  (where  $N = 2$  for  $i \neq j$  and  $N = 6$  for  $i = j$ ) for  $\text{Cp}^{85}\text{Re}(\text{CH}_3)(\text{CO})(\text{NO})$ . B3LYP/cc-pV5Z,cc-pwCVQZ-PP level harmonic force field was utilised for the anharmonic calculation at B3LYP level with (12s11p10d8f)[8s7p6d4f] contraction on Re atom and cc-pVDZ basis set for H, C, N and O atoms. Values are determined by the GAUSSIAN package. (continued).

| Mode            | VBO           |               |               |               |               |               |               |               |               |               |
|-----------------|---------------|---------------|---------------|---------------|---------------|---------------|---------------|---------------|---------------|---------------|
| V <sub>11</sub> | -0.274407E-09 | 0.214109E-09  | 0.588591E-09  | 0.642297E-09  | 0.221020E-10  | 0.142956E-08  | -0.170131E-08 | 0.799504E-09  | 0.847576E-09  | -0.963381E-09 |
|                 | 0.193685E-09  | -0.835409E-09 | -0.202945E-08 | -0.372374E-08 | 0.120010E-08  | 0.159470E-08  | 0.790467E-09  | -0.122767E-08 | -0.315020E-08 | -0.108940E-08 |
|                 | -0.279567E-09 | -0.105527E-07 | 0.671683E-08  | 0.226801E-08  | 0.141497E-08  | 0.720010E-09  | -0.426110E-09 | 0.108940E-08  | -0.121989E-09 | 0.170265E-08  |
|                 | 0.336207E-08  | -0.214193E-09 | 0.881182E-09  | -0.769709E-09 | 0.745953E-10  | 0.277196E-09  | 0.358916E-07  | 0.101408E-09  | 0.271190E-06  | -0.458642E-08 |
| V <sub>10</sub> | 0.383852E-09  | 0.951888E-09  | -0.801767E-08 | -0.105332E-06 | -0.110780E-07 | 0.311069E-09  | 0.101408E-09  | 0.271190E-06  | -0.458642E-08 | -0.458642E-08 |
|                 | 0.281093E-06  | 0.185597E-09  | 0.109026E-08  | -0.411718E-09 | -0.625695E-09 | -0.151516E-09 | 0.101408E-09  | 0.271190E-06  | -0.458642E-08 | -0.458642E-08 |
|                 | -0.449789E-09 | 0.725400E-09  | 0.201941E-08  | -0.638777E-09 | -0.346251E-08 | 0.162815E-08  | 0.451211E-08  | 0.358705E-08  | 0.331484E-08  | 0.331484E-08  |
|                 | -0.184194E-08 | -0.117769E-07 | -0.685152E-08 | 0.803342E-08  | 0.264745E-08  | -0.377584E-08 | 0.628687E-07  | -0.583519E-07 | 0.108222E-06  | 0.108222E-06  |
| V <sub>9</sub>  | -0.105636E-06 | -0.122684E-07 | -0.141737E-08 | -0.438520E-08 | -0.998216E-08 | -0.286627E-08 | 0.396974E-08  | 0.918611E-09  | -0.685466E-08 | -0.685466E-08 |
|                 | 0.205841E-08  | 0.204670E-08  | 0.105182E-08  | -0.246550E-08 | -0.229017E-08 | -0.489593E-09 | 0.200963E-07  | 0.163948E-09  | 0.545804E-08  | 0.545804E-08  |
|                 | -0.912789E-08 | 0.575116E-08  | 0.234788E-08  | -0.153354E-08 | 0.279952E-08  | -0.332435E-06 | 0.168327E-06  | -0.426145E-08 | 0.472742E-09  | 0.472742E-09  |
|                 | -0.101522E-08 | -0.251583E-09 | 0.612616E-09  | -0.598378E-09 | -0.261381E-09 | 0.534297E-09  | 0.168327E-06  | -0.426145E-08 | 0.472742E-09  | 0.472742E-09  |
| V <sub>8</sub>  | 0.570503E-09  | -0.483134E-09 | 0.250698E-08  | -0.288025E-09 | 0.352056E-08  | 0.238831E-08  | 0.233672E-08  | 0.463132E-08  | -0.156423E-08 | -0.156423E-08 |
|                 | 0.201302E-08  | 0.461090E-08  | -0.806553E-07 | 0.474257E-07  | -0.169561E-07 | 0.991083E-08  | 0.174718E-09  | 0.125206E-07  | 0.247998E-08  | 0.247998E-08  |
|                 | -0.230729E-07 | -0.222240E-08 | -0.295273E-08 | -0.110191E-07 | -0.712287E-08 | 0.415257E-08  | -0.309479E-08 | 0.306965E-08  | 0.769677E-08  | 0.769677E-08  |
|                 | 0.524745E-08  | -0.455473E-08 | 0.524210E-08  | -0.533916E-08 | 0.225257E-08  | -0.209496E-08 | 0.195348E-07  | -0.365994E-09 | 0.976603E-08  | 0.976603E-08  |
| V <sub>7</sub>  | 0.556925E-08  | -0.253742E-08 | -0.202029E-08 | -0.313796E-09 | -0.386126E-08 | 0.168210E-06  | 0.453372E-06  | -0.640182E-08 | -0.339846E-08 | -0.339846E-08 |
|                 | -0.363223E-08 | 0.770107E-09  | -0.485251E-09 | -0.753086E-09 | -0.825856E-09 | 0.328984E-09  | 0.453372E-06  | -0.640182E-08 | -0.339846E-08 | -0.339846E-08 |
|                 | 0.234661E-09  | 0.882011E-09  | 0.101674E-08  | 0.952278E-09  | 0.483034E-09  | -0.500688E-09 | 0.168978E-08  | 0.168978E-08  | -0.339191E-08 | -0.339191E-08 |
|                 | -0.992587E-09 | 0.495167E-08  | 0.908149E-08  | 0.181279E-07  | -0.308214E-08 | 0.114935E-07  | 0.691057E-09  | -0.344703E-08 | -0.144928E-08 | -0.144928E-08 |
| V <sub>6</sub>  | 0.869051E-09  | -0.132290E-07 | 0.767073E-08  | -0.650096E-08 | 0.173121E-08  | -0.685530E-08 | 0.655699E-08  | 0.812693E-09  | 0.318837E-08  | 0.318837E-08  |
|                 | -0.939139E-08 | -0.396606E-09 | -0.518633E-08 | 0.881269E-09  | 0.910444E-08  | -0.317211E-08 | -0.120273E-06 | 0.695329E-09  | -0.731428E-09 | -0.731428E-09 |
|                 | 0.345971E-11  | 0.138727E-08  | 0.149672E-08  | -0.588982E-08 | 0.222949E-07  | 0.134438E-07  | -0.202724E-07 | -0.150763E-05 | 0.451220E-06  | 0.451220E-06  |
|                 | 0.740305E-06  | 0.479935E-08  | 0.913981E-08  | -0.325045E-08 | -0.654243E-08 | -0.888715E-09 | -0.151363E-08 | 0.256644E-08  | -0.439383E-08 | -0.439383E-08 |
| V <sub>5</sub>  | 0.212534E-09  | 0.215092E-08  | 0.197333E-08  | 0.170726E-08  | -0.410557E-09 | -0.817675E-09 | -0.151363E-08 | 0.256644E-08  | -0.439383E-08 | -0.439383E-08 |
|                 | -0.144018E-08 | 0.663499E-08  | 0.164836E-07  | 0.318821E-07  | -0.875968E-08 | 0.193563E-07  | 0.666525E-09  | -0.507297E-08 | -0.377296E-08 | -0.377296E-08 |
|                 | 0.125820E-08  | -0.321399E-07 | 0.145390E-07  | -0.601778E-08 | 0.170530E-08  | -0.123410E-07 | 0.114807E-07  | 0.241961E-08  | 0.344981E-08  | 0.344981E-08  |
|                 | -0.978550E-08 | -0.162149E-08 | -0.987371E-08 | 0.655062E-09  | -0.866936E-09 | -0.526024E-08 | -0.371182E-06 | 0.100422E-08  | 0.571177E-08  | 0.571177E-08  |
| V <sub>4</sub>  | -0.527798E-08 | 0.497307E-08  | -0.227114E-07 | -0.317597E-06 | 0.115020E-09  | 0.101383E-07  | -0.208912E-07 | -0.508561E-05 | -0.296228E-06 | -0.296228E-06 |
|                 | 0.242181E-05  | 0.826489E-08  | 0.187616E-07  | -0.812125E-08 | -0.132547E-07 | -0.546511E-08 | -0.208912E-07 | -0.508561E-05 | -0.296228E-06 | -0.296228E-06 |
|                 | -0.249408E-09 | 0.924755E-09  | 0.384276E-09  | 0.218291E-09  | -0.150567E-08 | -0.218726E-08 | -0.510782E-08 | -0.126700E-08 | 0.200348E-08  | 0.200348E-08  |
|                 | -0.193679E-09 | 0.231854E-08  | 0.968738E-08  | 0.222440E-07  | -0.841279E-08 | 0.120753E-07  | 0.216635E-08  | -0.356484E-08 | -0.167862E-08 | -0.167862E-08 |
| V <sub>3</sub>  | 0.299589E-08  | 0.606450E-08  | -0.134602E-08 | -0.908294E-09 | 0.194986E-08  | -0.641863E-08 | 0.665742E-08  | 0.219558E-08  | 0.239800E-08  | 0.239800E-08  |
|                 | -0.744167E-08 | -0.109220E-08 | -0.813215E-08 | 0.144496E-08  | -0.912324E-09 | -0.352572E-09 | -0.365202E-06 | 0.618520E-09  | -0.498998E-08 | -0.498998E-08 |
|                 | 0.153502E-09  | -0.263823E-08 | 0.220561E-07  | 0.318178E-06  | 0.125707E-07  | 0.120816E-07  | -0.313791E-07 | -0.350447E-05 | -0.654921E-06 | -0.654921E-06 |
|                 | -0.195870E-05 | -0.711119E-08 | -0.211246E-07 | 0.110140E-07  | 0.164881E-07  | 0.859222E-08  | -0.313791E-07 | -0.350447E-05 | -0.654921E-06 | -0.654921E-06 |
| V <sub>2</sub>  | -0.371275E-10 | 0.551209E-08  | 0.131918E-09  | 0.182757E-09  | 0.253287E-09  | -0.415556E-09 | -0.688222E-09 | 0.101827E-08  | -0.132357E-08 | -0.132357E-08 |
|                 | 0.118888E-08  | 0.117023E-08  | 0.886989E-09  | 0.180099E-09  | -0.225654E-08 | 0.815048E-09  | -0.143518E-08 | -0.152705E-08 | -0.106509E-08 | -0.106509E-08 |
|                 | 0.879934E-09  | -0.460072E-09 | -0.858088E-09 | -0.906661E-09 | 0.385953E-08  | 0.544153E-09  | -0.607537E-09 | -0.483318E-09 | -0.812325E-08 | -0.812325E-08 |
|                 | -0.338609E-08 | -0.156570E-07 | -0.242925E-07 | 0.127218E-07  | -0.736713E-08 | 0.108831E-06  | 0.835191E-09  | -0.943164E-09 | 0.218946E-07  | 0.218946E-07  |
| V <sub>1</sub>  | 0.136916E-07  | 0.682623E-07  | 0.455442E-07  | -0.195415E-08 | -0.979512E-09 | 0.205321E-08  | -0.973209E-09 | -0.361415E-09 | 0.117924E-09  | 0.117924E-09  |
|                 | 0.430588E-08  | 0.116309E-05  | -0.904415E-06 | 0.378124E-05  | 0.631235E-06  | -0.289817E-05 | -0.973209E-09 | -0.361415E-09 | 0.117924E-09  | 0.117924E-09  |
|                 | -0.332308E-09 | 0.238316E-09  | 0.391156E-10  | 0.503497E-10  | -0.117538E-09 | -0.737981E-09 | -0.139302E-08 | 0.271749E-08  | 0.324766E-08  | 0.324766E-08  |
|                 | 0.116077E-09  | -0.771498E-09 | 0.929202E-09  | 0.150364E-08  | -0.734939E-09 | -0.273296E-08 | -0.147763E-08 | 0.184482E-09  | -0.234387E-08 | -0.234387E-08 |
| V <sub>0</sub>  | -0.928652E-09 | -0.412715E-08 | 0.388586E-08  | 0.210357E-08  | -0.219315E-08 | -0.495142E-08 | 0.294131E-08  | 0.165396E-10  | -0.392642E-08 | -0.392642E-08 |
|                 | -0.449941E-09 | 0.148757E-07  | 0.266434E-08  | 0.127518E-07  | 0.130757E-08  | 0.109728E-06  | 0.555765E-08  | 0.214094E-08  | 0.611890E-08  | 0.611890E-08  |
|                 | -0.365016E-08 | -0.495950E-07 | -0.396104E-07 | 0.227038E-08  | 0.161505E-08  | 0.326515E-09  | -0.398112E-08 | 0.118870E-08  | 0.749159E-08  | 0.749159E-08  |
|                 | -0.108839E-07 | -0.485711E-07 | -0.371325E-06 | -0.221010E-05 | -0.845628E-06 | -0.411657E-05 | -0.398112E-08 | 0.118870E-08  | 0.749159E-08  | 0.749159E-08  |

**Table S26:** Anharmonic potential parameters  $\frac{\sqrt{h^3 c^3 \omega_0^2 \omega_j / E_h^3}}{N} \frac{\partial^3 V_{\text{B02}}}{\partial q_i \partial q_j}$  (where  $N = 2$  for  $i \neq j$  and  $N = 6$  for  $i = j$ ) for  $\text{Cp}^{185}\text{Re}(\text{CH}_3)(\text{CO})(\text{NO})$ , B3LYP/cc-pV5Z,cc-pwCVQZ-PP level harmonic force field was utilised for the anharmonic calculation at B3LYP level with (12s11p10d8f)[8s7p6d4f] contraction on Re atom and cc-pVDZ basis set for H, C, N and O atoms. Values are determined by the GAUSSIAN package. (continued).

| Mode           | VBO           |               |               |               |               |               |               |               |               |  |
|----------------|---------------|---------------|---------------|---------------|---------------|---------------|---------------|---------------|---------------|--|
| v <sub>3</sub> | 0.174329E-11  | 0.353815E-09  | -0.105740E-09 | -0.123771E-09 | 0.806573E-10  | -0.353490E-09 | -0.491896E-09 | 0.122678E-08  | 0.834863E-09  |  |
|                | 0.872721E-09  | 0.529802E-09  | 0.808325E-09  | 0.686523E-09  | -0.123025E-08 | -0.190428E-08 | -0.101363E-08 | 0.132775E-08  | -0.232180E-09 |  |
|                | 0.713618E-09  | -0.196688E-08 | 0.217388E-08  | -0.186972E-08 | -0.212173E-10 | -0.423134E-08 | -0.650499E-10 | 0.149191E-08  | -0.252459E-08 |  |
|                | -0.267734E-09 | -0.548448E-08 | -0.436008E-08 | 0.114219E-07  | -0.486362E-09 | 0.117618E-06  | 0.271629E-08  | 0.220090E-09  | 0.240628E-08  |  |
|                | 0.223300E-07  | 0.170335E-07  | -0.229858E-07 | 0.292956E-08  | 0.680237E-09  | -0.822771E-09 | -0.172418E-08 | -0.263050E-08 | 0.133663E-08  |  |
| v <sub>2</sub> | 0.543989E-08  | 0.250555E-06  | -0.283226E-05 | 0.367712E-06  | -0.107307E-05 | -0.343444E-05 |               |               |               |  |
|                | 0.470212E-09  | -0.651476E-10 | 0.414930E-09  | 0.490671E-09  | -0.972290E-10 | -0.600186E-09 | -0.181555E-08 | 0.184029E-08  | 0.125825E-08  |  |
|                | 0.432991E-09  | 0.127885E-08  | 0.959112E-09  | 0.851413E-09  | 0.479670E-09  | -0.106445E-08 | 0.188720E-08  | -0.169171E-08 | -0.384272E-08 |  |
|                | -0.622965E-09 | -0.255926E-08 | 0.115549E-08  | 0.613040E-08  | 0.657292E-08  | -0.637059E-08 | 0.210181E-08  | -0.268838E-08 | -0.581177E-08 |  |
|                | -0.256384E-08 | 0.788958E-08  | -0.123946E-07 | 0.164951E-07  | 0.588077E-08  | 0.117789E-06  | 0.426442E-08  | -0.535698E-09 | 0.200004E-07  |  |
| v <sub>1</sub> | -0.362266E-07 | -0.949937E-08 | 0.810096E-08  | -0.826367E-09 | -0.192983E-08 | 0.212278E-08  | 0.319713E-09  | 0.187083E-08  | 0.826448E-08  |  |
|                | -0.131191E-07 | -0.132873E-05 | 0.260468E-05  | 0.345580E-06  | 0.385281E-06  | -0.428577E-05 |               |               |               |  |
|                | 0.1117340E-09 | 0.132765E-09  | 0.276904E-09  | 0.219310E-09  | -0.107345E-09 | -0.624622E-09 | -0.147821E-08 | 0.113871E-08  | 0.160220E-08  |  |
|                | 0.721999E-09  | 0.424142E-09  | 0.810631E-09  | 0.985991E-09  | -0.279621E-09 | -0.166066E-08 | 0.102154E-09  | -0.888820E-09 | -0.259004E-08 |  |
|                | -0.492919E-09 | -0.302340E-08 | 0.207014E-08  | 0.312996E-08  | 0.257346E-08  | -0.510251E-08 | 0.187243E-08  | -0.108296E-08 | -0.510264E-08 |  |
| v <sub>1</sub> | -0.239354E-08 | 0.102591E-07  | -0.524596E-08 | 0.155461E-07  | 0.294782E-08  | 0.123739E-06  | 0.407327E-08  | 0.661998E-09  | 0.137284E-07  |  |
|                | -0.131945E-07 | -0.225480E-07 | -0.148753E-07 | 0.981139E-09  | -0.116448E-09 | 0.615154E-09  | -0.945751E-09 | 0.986507E-09  | 0.686680E-08  |  |
|                | -0.976481E-08 | -0.273272E-06 | 0.394032E-06  | -0.419210E-06 | 0.463263E-07  | -0.134743E-05 |               |               |               |  |

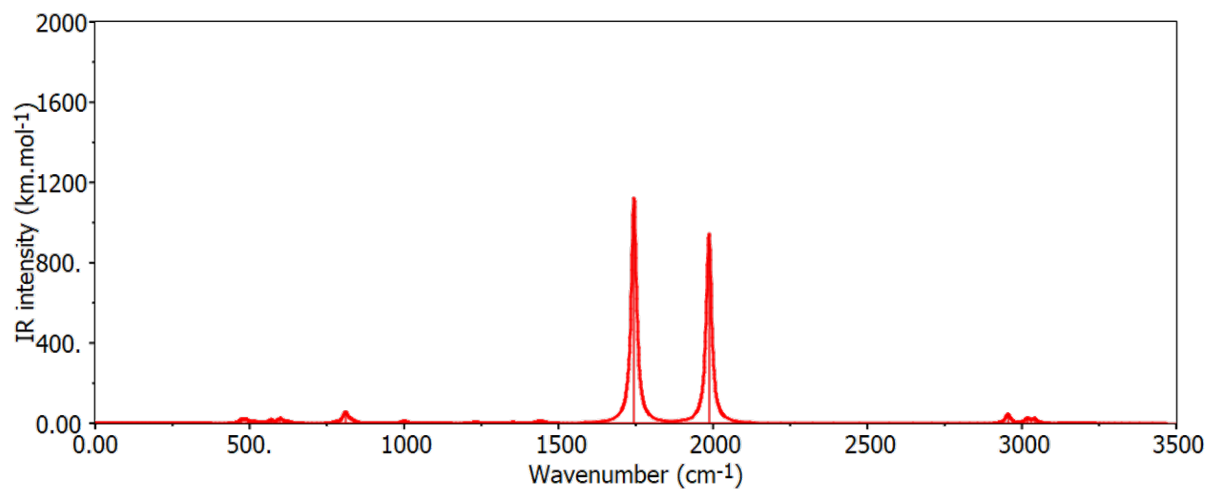

Figure S2: Harmonic vibrational spectrum of  $\text{Cp}^{187}\text{Re}(\text{CH}_3)(\text{CO})(\text{NO})$  at B3LYP/cc-pV5Z,cc-pwCVQZ-PP level of theory. Spectrum is convoluted with Lorentzian function using a full-width at half-maximum of  $20\text{ cm}^{-1}$ . Peak positions are scaled by 0.980. The most intense peaks in the spectrum are due to the NO (left:  $\nu_{10}$ ) and CO (right:  $\nu_9$ ) stretching vibrations.

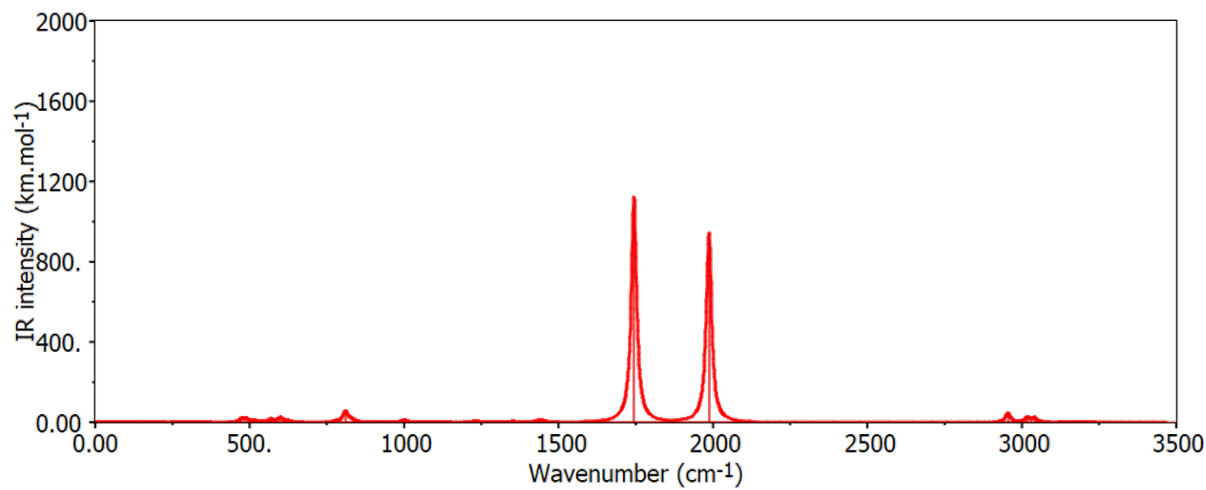

Figure S3: Harmonic vibrational spectrum of  $\text{Cp}^{185}\text{Re}(\text{CH}_3)(\text{CO})(\text{NO})$  at B3LYP/cc-pV5Z,cc-pwCVQZ-PP level of theory. Spectrum is convoluted with Lorentzian function using a full-width at half-maximum of  $20\text{ cm}^{-1}$ . Peak positions are scaled by 0.980. The most intense peaks in the spectrum are due to the NO (left:  $\nu_{10}$ ) and CO (right:  $\nu_9$ ) stretching vibrations.

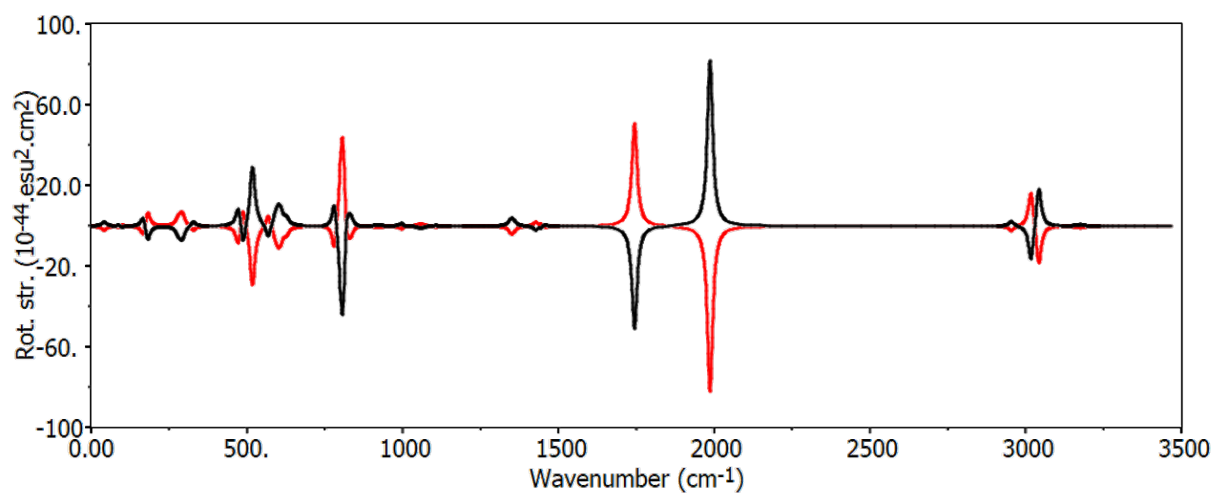

Figure S4: Harmonic vibrational circular dichroism spectrum of (R)- (red) and (S)- (black) enantiomers of  $\text{Cp}^{187}\text{Re}(\text{CH}_3)(\text{CO})(\text{NO})$  at B3LYP/cc-pV5Z,cc-pwCVQZ-PP level of theory. Spectrum is convoluted with Lorentzian function using a full-width at half-maximum of  $20\text{ cm}^{-1}$ . Peak positions are scaled by 0.980.

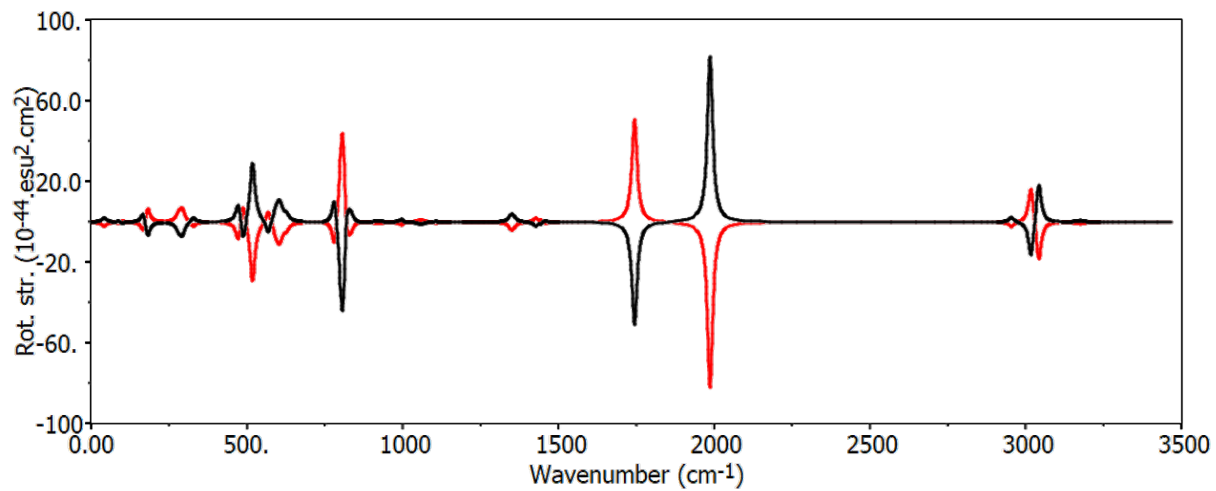

Figure S5: Harmonic vibrational circular dichroism spectrum of (R)- (red) and (S)- (black) enantiomers of  $\text{Cp}^{185}\text{Re}(\text{CH}_3)(\text{CO})(\text{NO})$  at B3LYP/cc-pV5Z,cc-pwCVQZ-PP level of theory. Spectrum is convoluted with Lorentzian function using a full-width at half-maximum of  $20\text{ cm}^{-1}$ . Peak positions are scaled by 0.980.

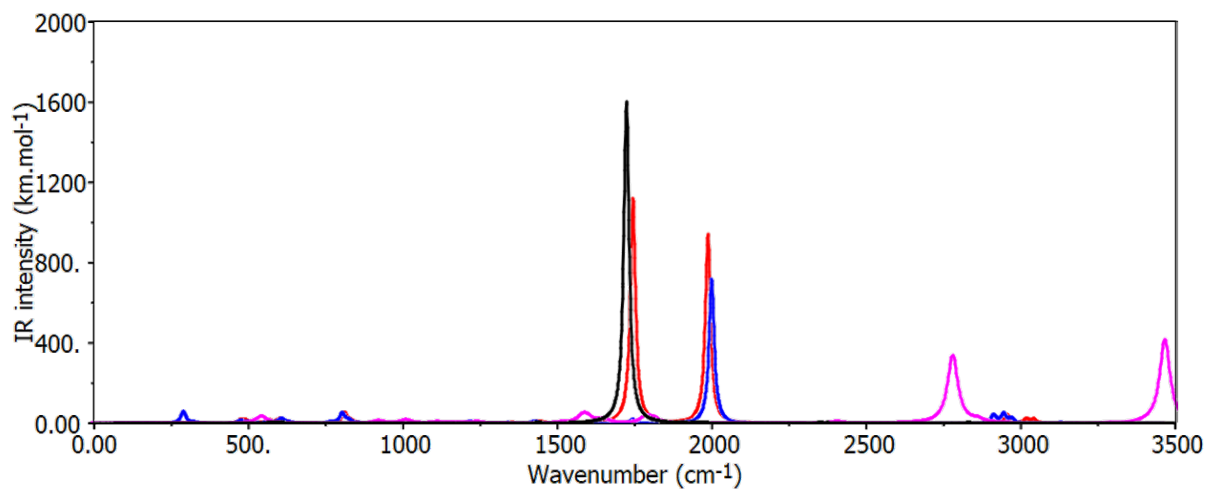

Figure S6: Scaled (0.980) harmonic (red), anharmonic fundamentals (blue), overtones (magenta) and combination (black) bands for  $\text{Cp}^{187}\text{Re}(\text{CH}_3)(\text{CO})(\text{NO})$  structure optimized at B3LYP/cc-pV5Z,cc-pwCVQZ-PP level of theory. The harmonic treatment is done at B3LYP/cc-pV5Z,cc-pwCVQZ-PP level of theory, whereas the anharmonic calculations are performed at B3LYP level with (12s11p10d8f)/[8s7p6d4f] contraction on Re atom and cc-pVDZ basis set for H, C, N and O atoms employing the second order vibrational perturbation (VPT2) theory within Gaussian16 software package. Spectrum is convoluted with Lorentzian function using a full-width at half-maximum of  $20\text{ cm}^{-1}$ . Overtone and combination bands up to  $3500\text{ cm}^{-1}$  are included in the plot. Intensity of the overtone bands are 20 times enhanced as compared to other bands. The peak from the combination bands (black) at  $1724.69\text{ cm}^{-1}$  is due to the combination of  $\nu_{29}$  and  $\nu_{24}$  bands.

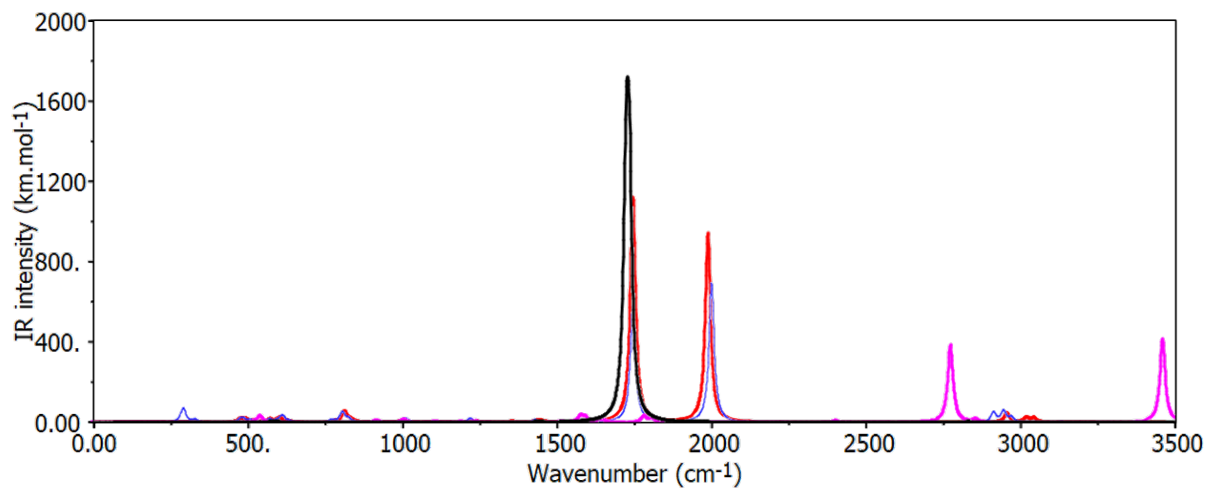

Figure S7: Scaled (0.980) harmonic (red), anharmonic fundamentals (blue), overtones (magenta) and combination (black) bands for  $\text{Cp}^{185}\text{Re}(\text{CH}_3)(\text{CO})(\text{NO})$  structure optimized at B3LYP/cc-pV5Z,cc-pwCVQZ-PP level of theory. The harmonic treatment is done at B3LYP/cc-pV5Z,cc-pwCVQZ-PP level of theory, whereas the anharmonic calculations are performed at B3LYP level with (12s11p10d8f)/[8s7p6d4f] contraction on Re atom and cc-pVDZ basis set for H, C, N and O atoms employing the second order vibrational perturbation (VPT2) theory within Gaussian16 software package. Spectrum is convoluted with Lorentzian function using a full-width at half-maximum of  $20\text{ cm}^{-1}$ . Overtone and combination bands up to  $3500\text{ cm}^{-1}$  are included in the plot. Intensity of the overtone bands are 20 times enhanced, whereas the intensity of combination bands are scaled to 66% as compared to other bands. The peaks in the combination bands (black) at  $1734.94\text{ cm}^{-1}$  and  $1724.64\text{ cm}^{-1}$  are due to the combination of  $\nu_{27}$  and  $\nu_{25}$ ,  $\nu_{29}$  and  $\nu_{24}$  bands.

## References

- [1] C. Medcraft, R. Wolf, M. Schnell, *Angew. Chem. Int. Ed.* **2014**, *53*, 11656–11659.
- [2] P. Pyykkö, *Mol. Phys.* **2018**, *116*, 1328–1338.
- [3] M. J. Frisch, G. W. Trucks, H. B. Schlegel, G. E. Scuseria, M. A. Robb, J. R. Cheeseman, G. Scalmani, V. Barone, B. Mennucci, G. A. Petersson, H. Nakatsuji, M. Caricato, X. Li, H. P. Hratchian, A. F. Izmaylov, J. Bloino, G. Zheng, J. Sonnenberg, M. Hada, M. Ehara, K. Toyota, R. Fukuda, J. Hasegawa, M. Ishida, T. Nakajima, Y. Honda, O. Kitao, H. Nakai, T. Vreven, J. A. Montgomery, J. E. Peralta, F. Ogliaro, M. Bearpark, J. J. Heyd, E. Brothers, K. N. Kudin, V. N. Staroverov, R. Kobayashi, J. Normand, K. Raghavachari, A. Rendell, J. C. Burant, S. S. Iyengar, J. Tomasi, M. Cossi, N. Rega, J. M. Millam, M. Klene, J. E. Knox, J. B. Cross, V. Bakken, C. Adamo, J. Jaramillo, R. Gomperts, R. Stratmann, O. Yazyev, A. J. Austin, R. Cammi, C. Pomelli, J. W. Ochterski, R. Martin, K. Morokuma, V. G. Zakrzewski, G. A. Voth, P. Salvador, J. J. Dannenberg, S. Dapprich, A. D. Daniels, Farkas, J. B. Foresman, J. V. Ortiz, J. Cioslowski, D. J. Fox, *Gaussian 09*, Wallingford CT, 2009.
- [4] D. Figgen, K. A. Peterson, M. Dolg, H. Stoll, *J. Chem. Phys.* **2009**, *130*, 164108.
- [5] J. Y. A. Weigand, X. Cao, M. Dolg, *Theor. Chem. Acc.* **2010**, *126*, 117–127.
- [6] V. Barone, M. Biczysko, J. Bloino, C. Puzzarini, *J. Chem. Phys.* **2014**, *141*, 034107.
- [7] D. Andrae, U. Häußermann, M. Dolg, H. Stoll, H. Preuß, *Theor. Chim. Acta* **1990**, *77*, 123–141.
- [8] R. Berger, J. L. Stuber, *Mol. Phys.* **2007**, *105*, 41–49.
- [9] A. D. Buckingham, W. Urland, *Chem. Rev.* **1975**, *75*, 113–117.
- [10] S. A. Brueck, N. Sahu, K. Gaul, R. Berger, *arXiv:2102.09897 [physics.chem-ph]* **2021**.
- [11] M. Quack, J. Stohner, *J. Chem. Phys.* **2003**, *119*, 11228–11240.
- [12] K. Gaul, M. G. Kozlov, T. A. Isaev, R. Berger, *Phys. Rev. Lett.* **2020**, *125*, 123004.
- [13] K. Gaul, M. G. Kozlov, T. A. Isaev, R. Berger, *Phys. Rev. A* **2020**, *102*, 032816.
